# Supplementary material for: Adaptive Cholesky Gaussian Processes
Source: arXiv:2202.10769 source file (2023-02-23)
Supplement: Supplementary file 1 [file appendix_bound_plots.tex]

\subsubsection{Bounds for experiments on \texttt{metro}}
\label{subsec:bounds_metro}
\begin{figure}[htb!]
	\begin{minipage}[b]{.5\textwidth}
		\centering
		\includegraphics[width=0.96\textwidth]{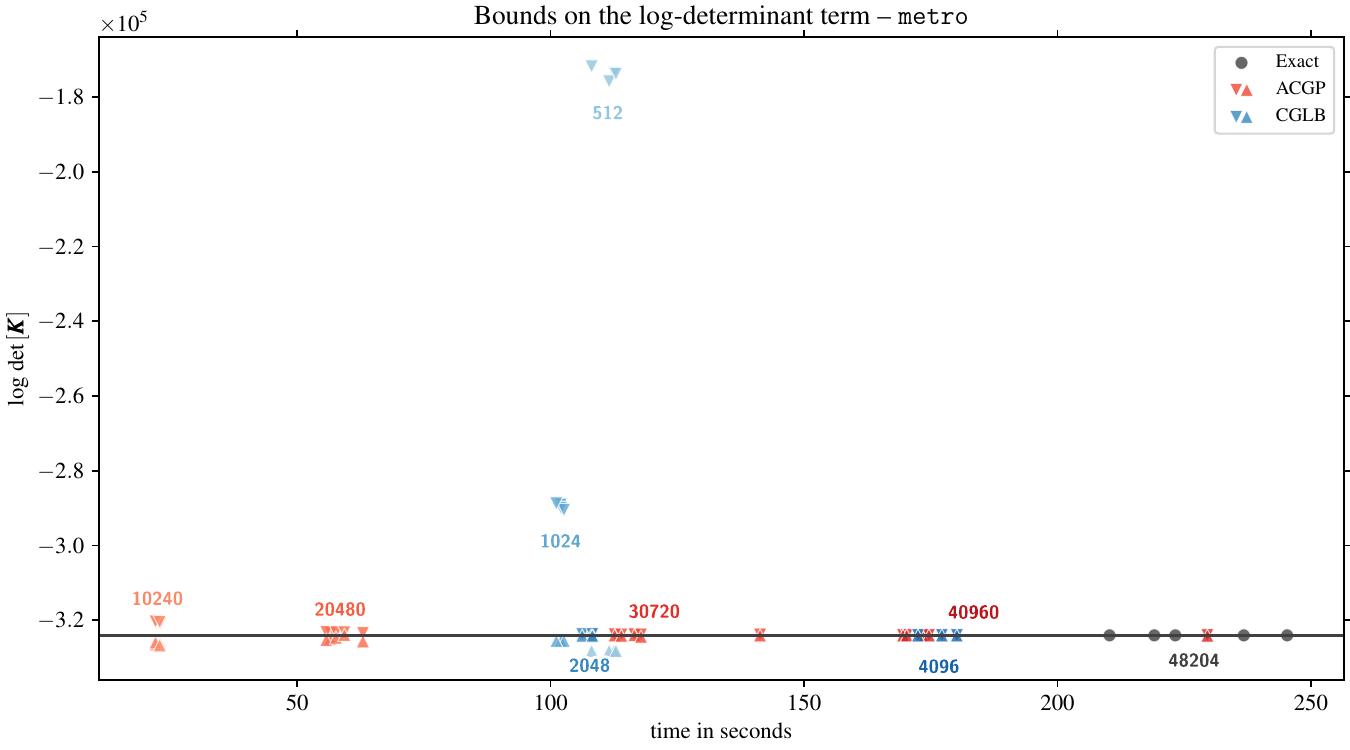}
		\subcaption{SE kernel, $\log\ell = -1$}
		\label{subfig:metro_rbf_loget_-1}
	\end{minipage}
	\begin{minipage}[b]{.5\textwidth}
		\centering
		\includegraphics[width=0.96\textwidth]{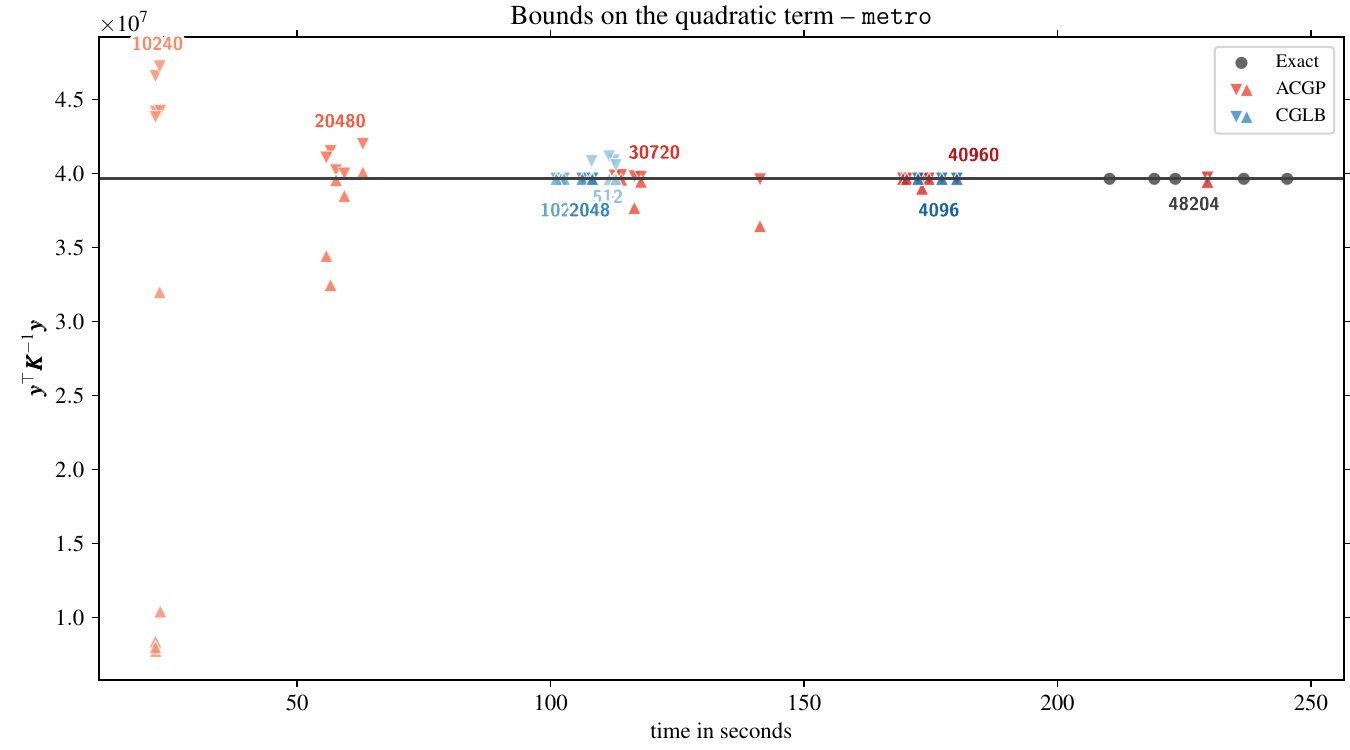}
		\subcaption{SE kernel, $\log\ell = -1$}
		\label{subfig:metro_rbf_quadratic_-1}
	\end{minipage}
	\begin{minipage}[b]{.5\textwidth}
		\centering
		\includegraphics[width=0.96\textwidth]{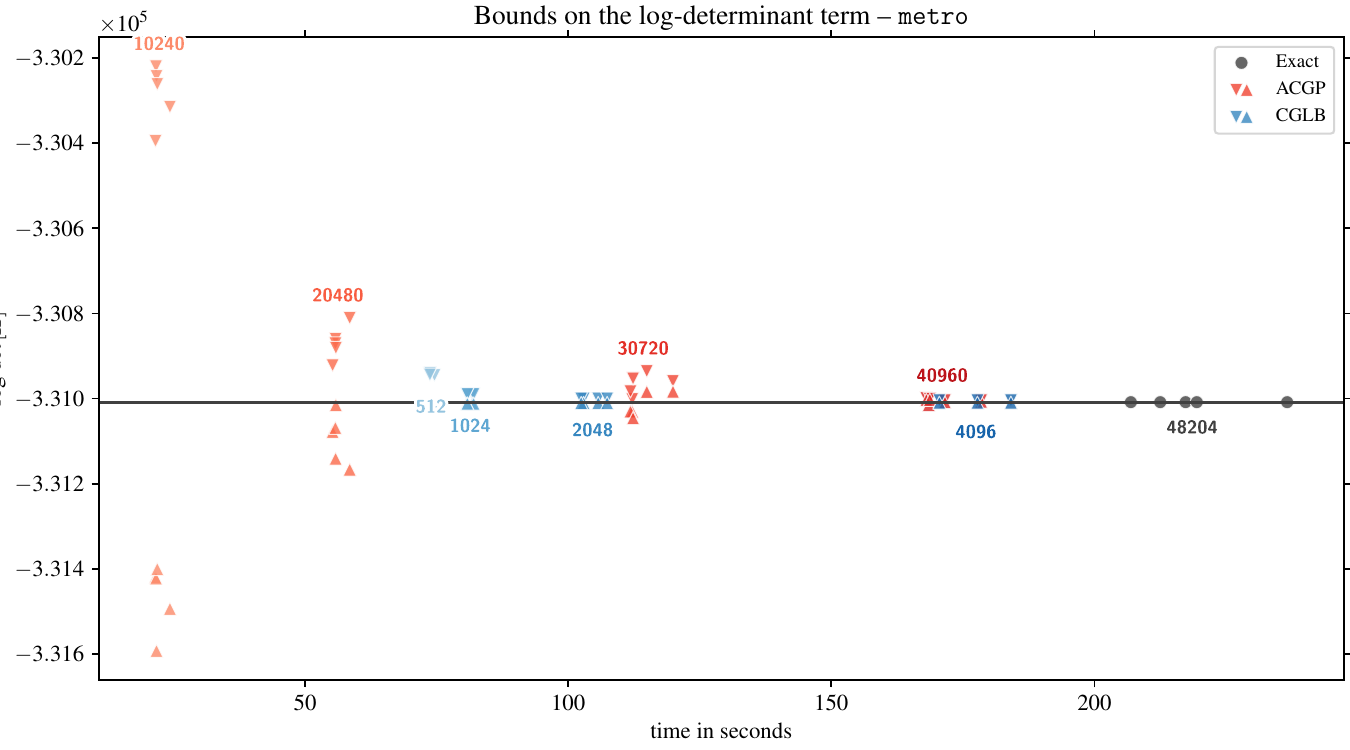}
		\subcaption{SE kernel, $\log\ell = 0$}
		\label{subfig:metro_rbf_loget_0}
	\end{minipage}
	\begin{minipage}[b]{.5\textwidth}
		\centering
		\includegraphics[width=0.96\textwidth]{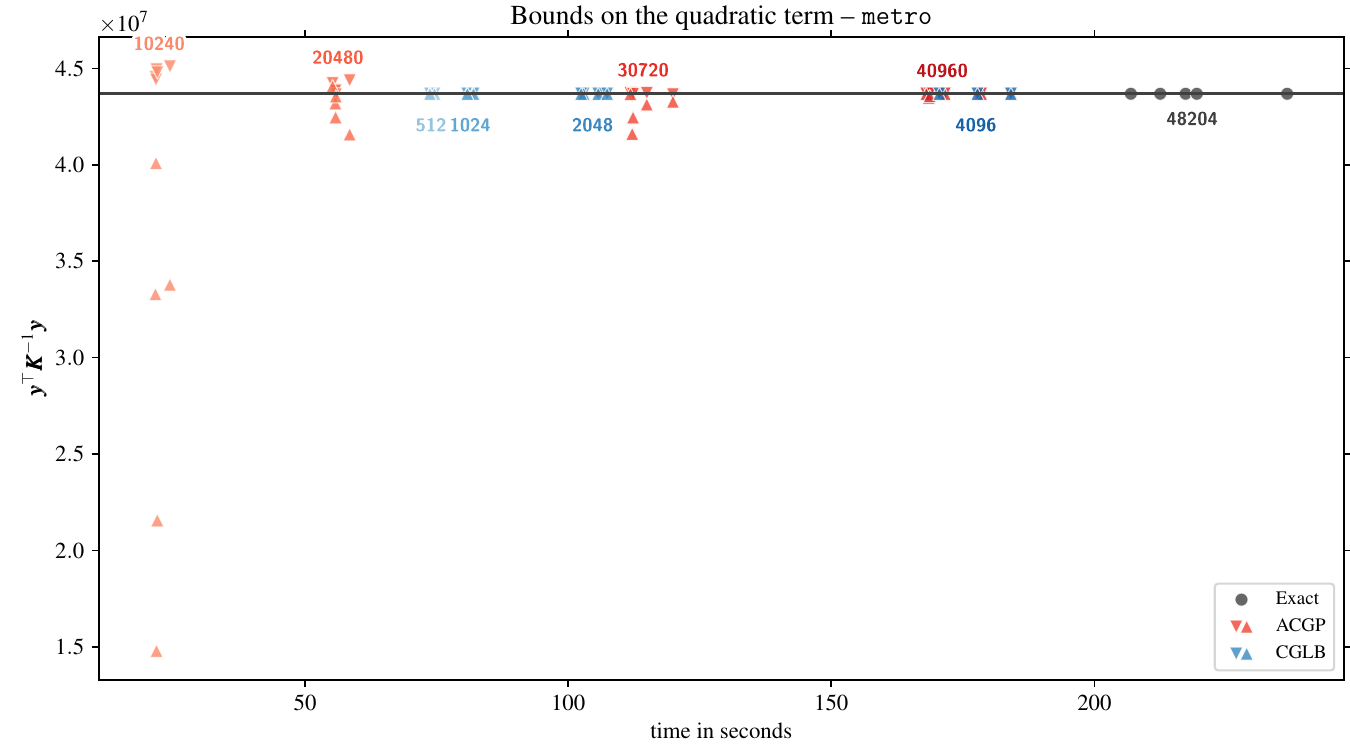}
		\subcaption{SE kernel, $\log\ell = 0$}
		\label{subfig:metro_rbf_quadratic_0}
	\end{minipage}
	\begin{minipage}[b]{.5\textwidth}
		\centering
		\includegraphics[width=0.96\textwidth]{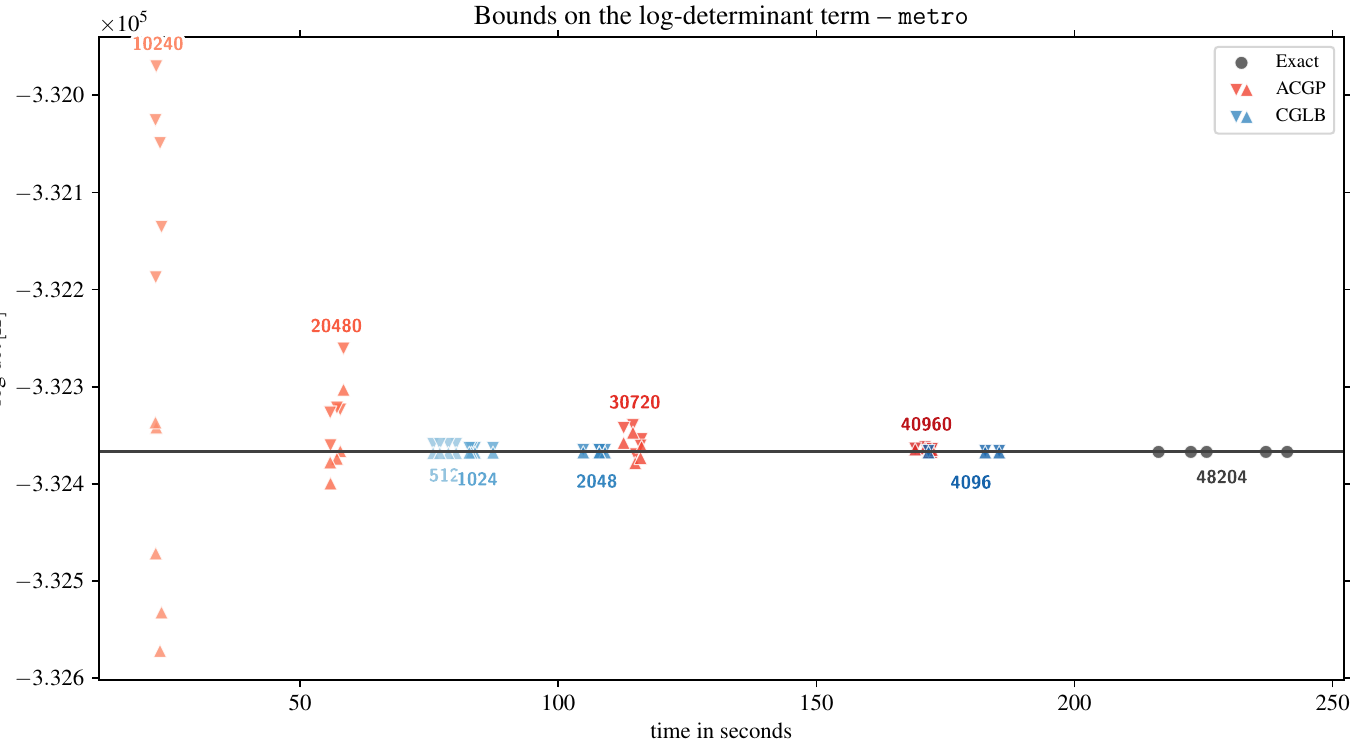}
		\subcaption{SE kernel, $\log\ell = 1$}
		\label{subfig:metro_rbf_loget_1}
	\end{minipage}
	\begin{minipage}[b]{.5\textwidth}
		\centering
		\includegraphics[width=0.96\textwidth]{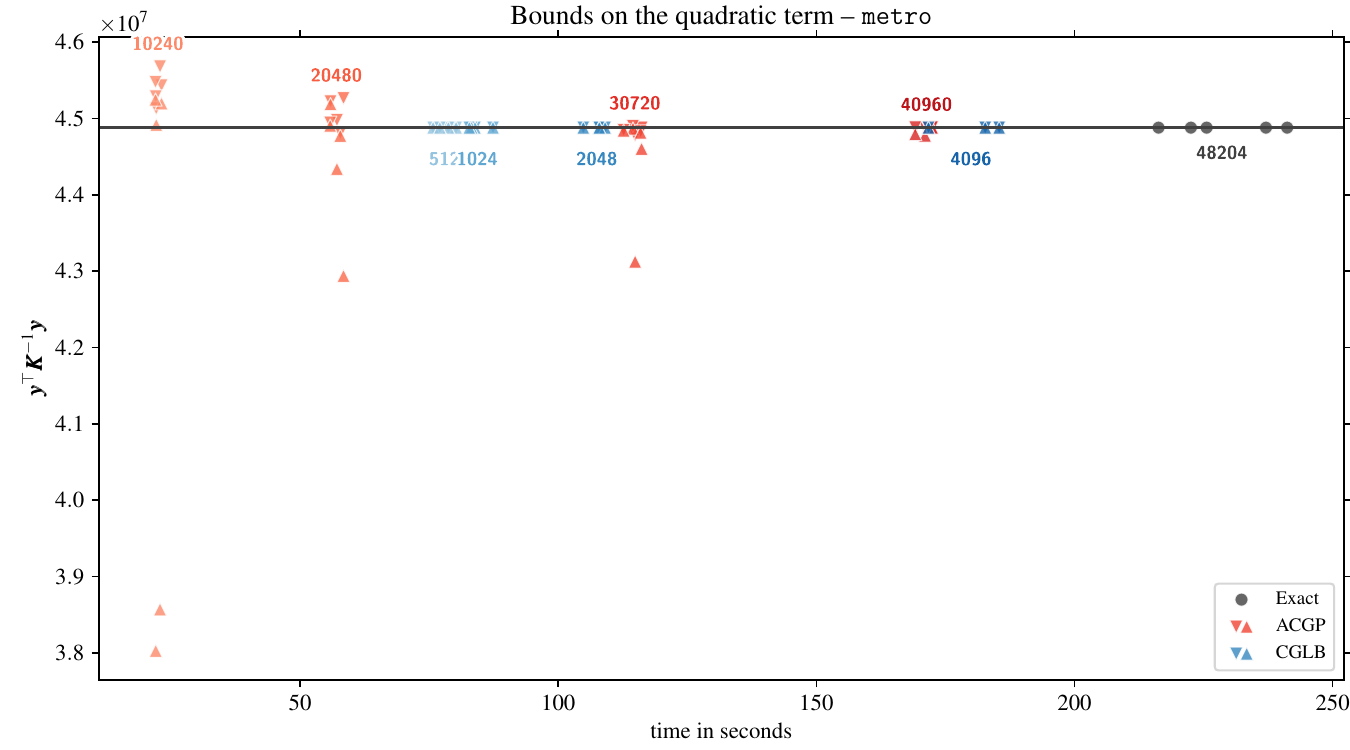}
		\subcaption{SE kernel, $\log\ell = 1$}
		\label{subfig:metro_rbf_quadratic_1}
	\end{minipage}
	\begin{minipage}[b]{.5\textwidth}
		\centering
		\includegraphics[width=0.96\textwidth]{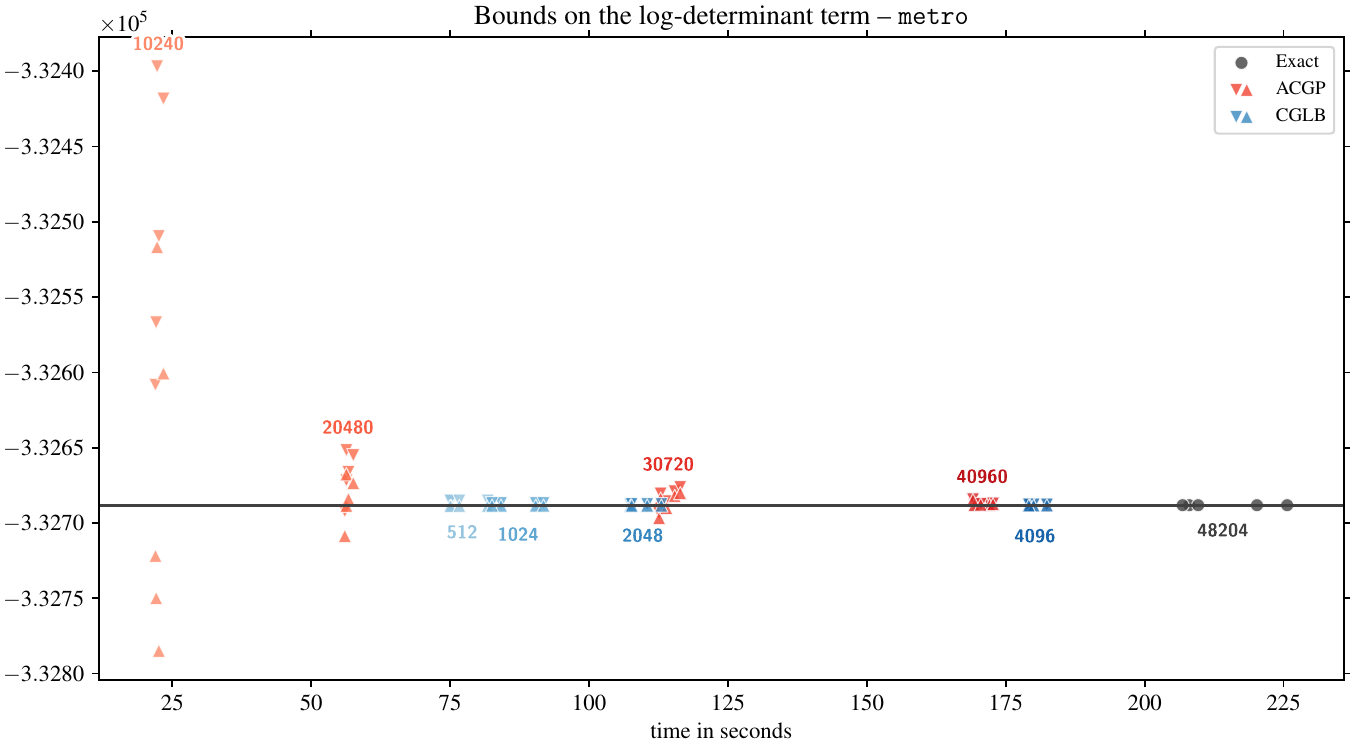}
		\subcaption{SE kernel, $\log\ell = 2$}
		\label{subfig:metro_rbf_loget_2}
	\end{minipage}
	\begin{minipage}[b]{.5\textwidth}
		\centering
		\includegraphics[width=0.96\textwidth]{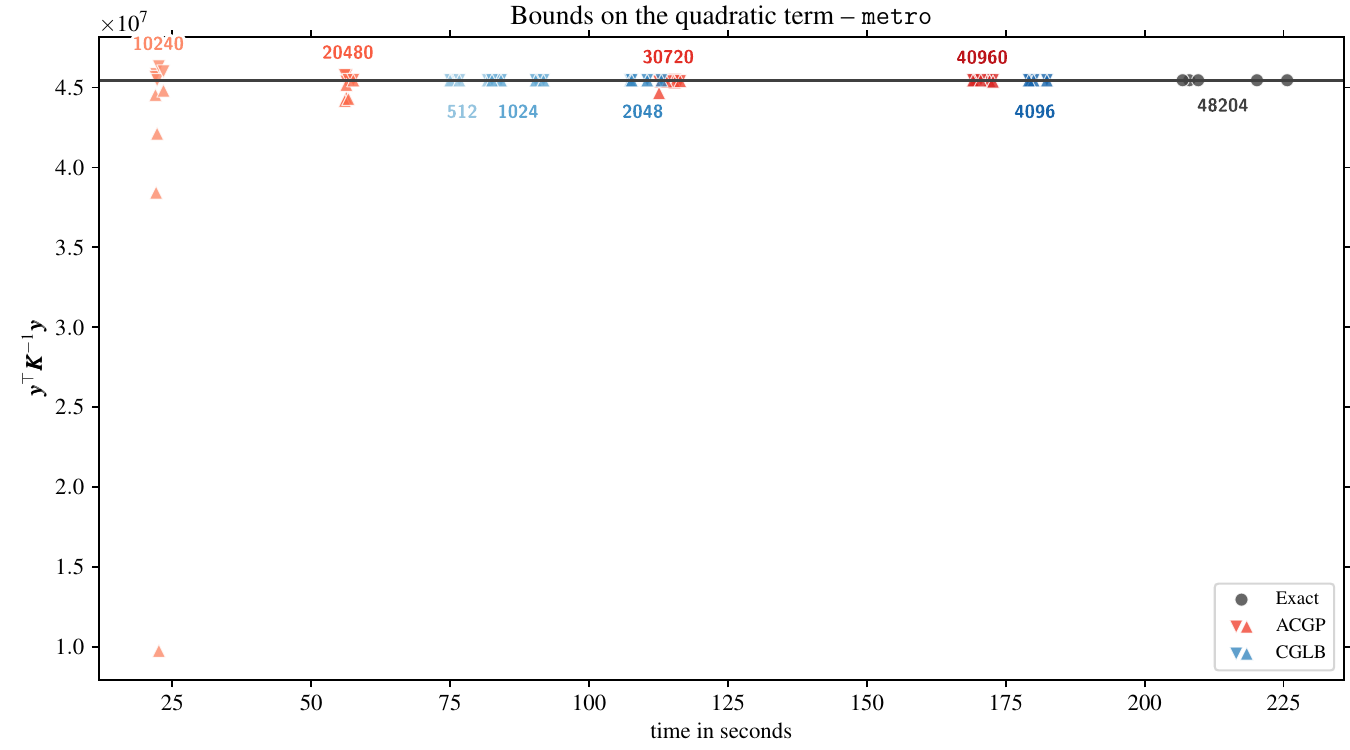}
		\subcaption{SE kernel, $\log\ell = 2$}
		\label{subfig:metro_rbf_quadratic_2}
	\end{minipage}
    \caption{Upper and lower bounds on the log-determinant term (left column) and the quadratic term (right column) for the \texttt{metro} dataset when using a squared exponential (SE) kernel.}
	\label{fig:bounds_metro_rbf}
\end{figure}
\clearpage
\begin{figure}[htb]
	\begin{minipage}[b]{.5\textwidth}
		\centering
		\includegraphics[width=0.96\textwidth]{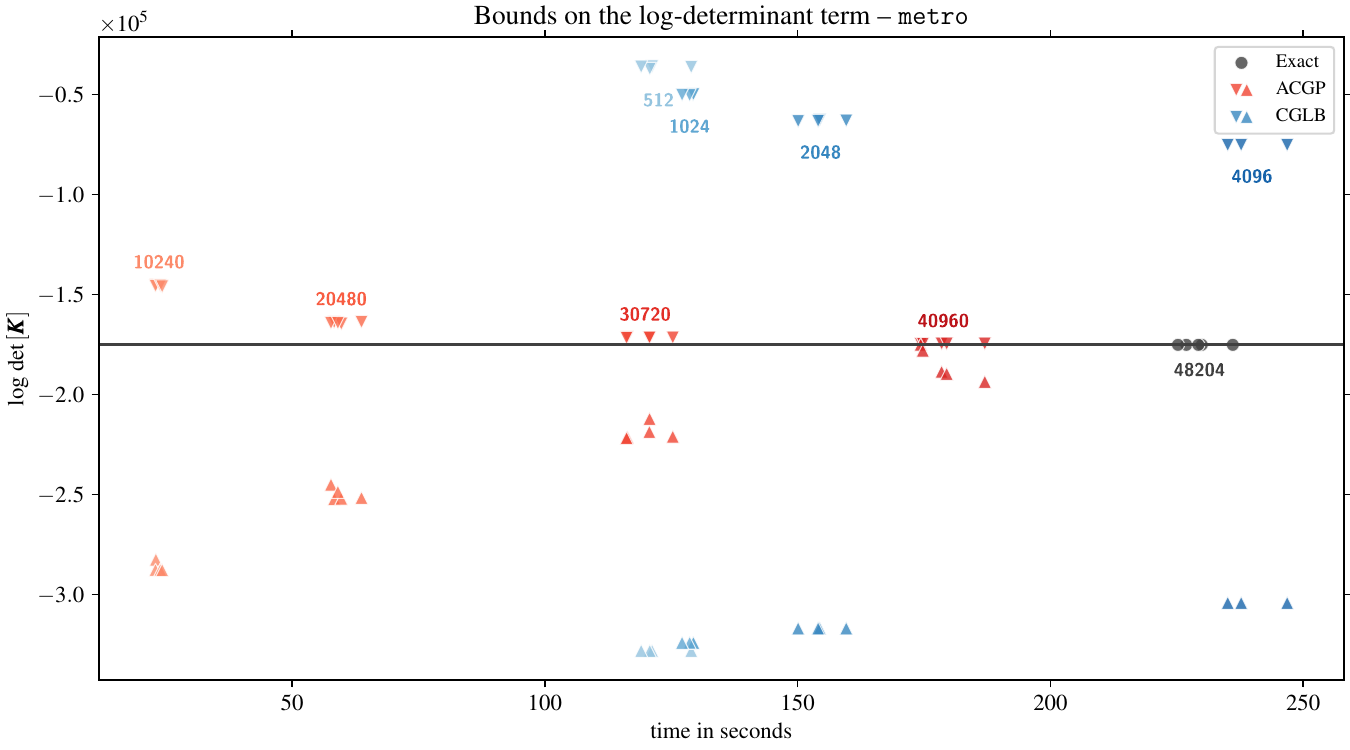}
		\subcaption{OU kernel, $\log\ell = -1$}
		\label{subfig:metro_ou_loget_-1}
	\end{minipage}
	\begin{minipage}[b]{.5\textwidth}
		\centering
		\includegraphics[width=0.96\textwidth]{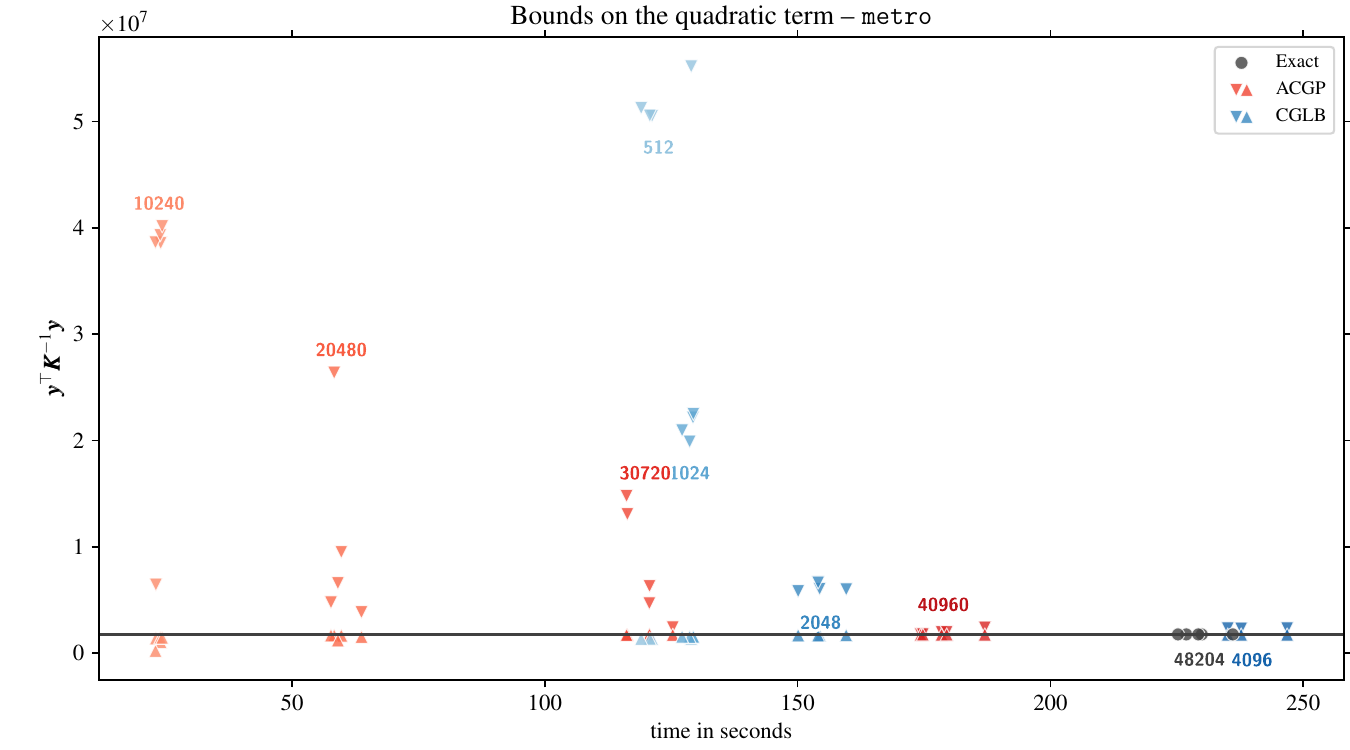}
		\subcaption{OU kernel, $\log\ell = -1$}
		\label{subfig:metro_ou_quadratic_-1}
	\end{minipage}

	\begin{minipage}[b]{.5\textwidth}
		\centering
		\includegraphics[width=0.96\textwidth]{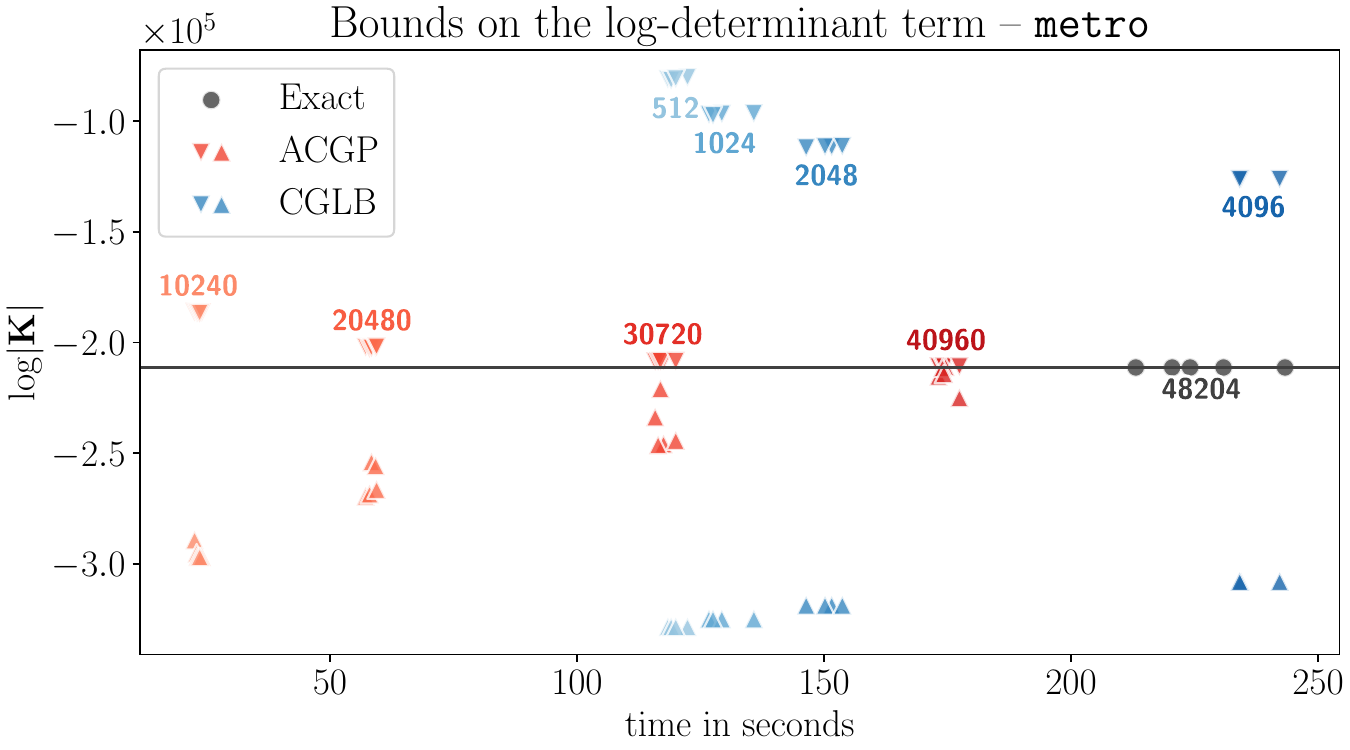}
		\subcaption{OU kernel, $\log\ell = 0$}
		\label{subfig:metro_ou_loget_0}
	\end{minipage}
	\begin{minipage}[b]{.5\textwidth}
		\centering
		\includegraphics[width=0.96\textwidth]{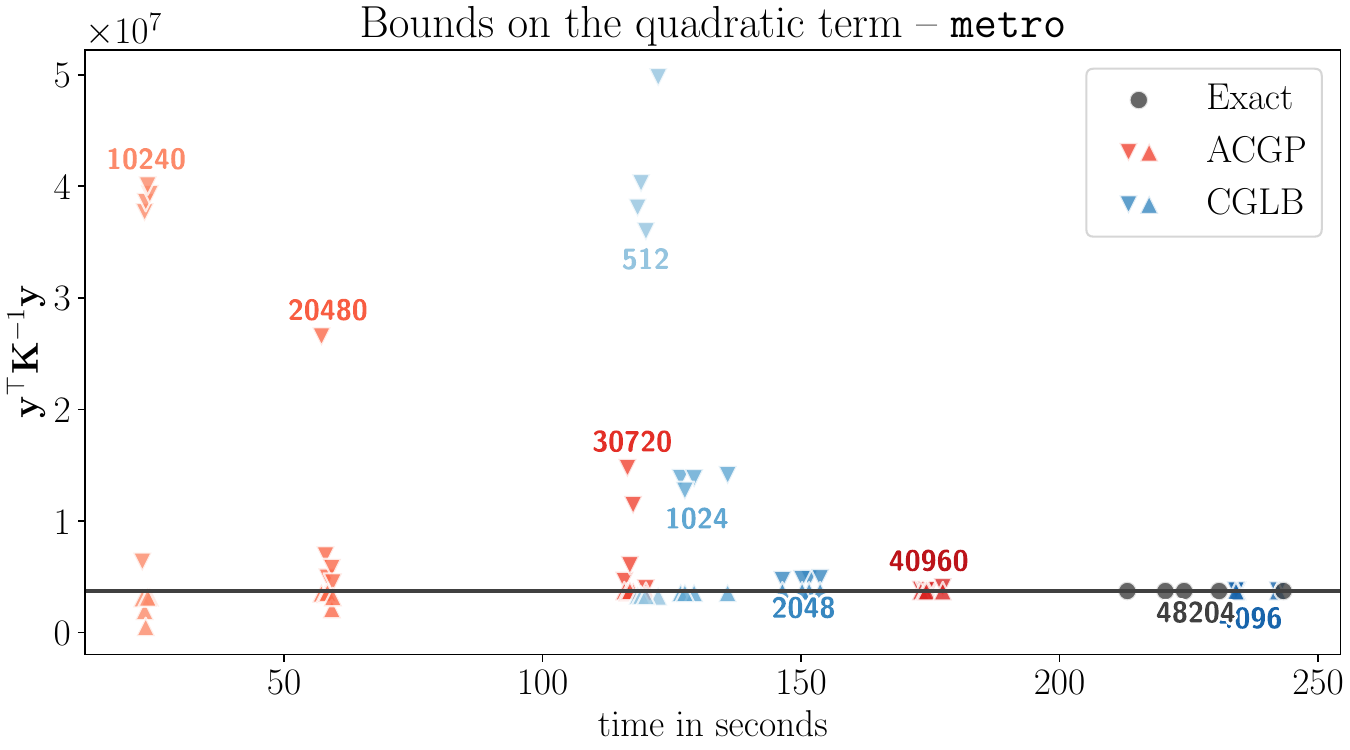}
		\subcaption{OU kernel, $\log\ell = 0$}
		\label{subfig:metro_ou_quadratic_0}
	\end{minipage}

	\begin{minipage}[b]{.5\textwidth}
		\centering
		\includegraphics[width=0.96\textwidth]{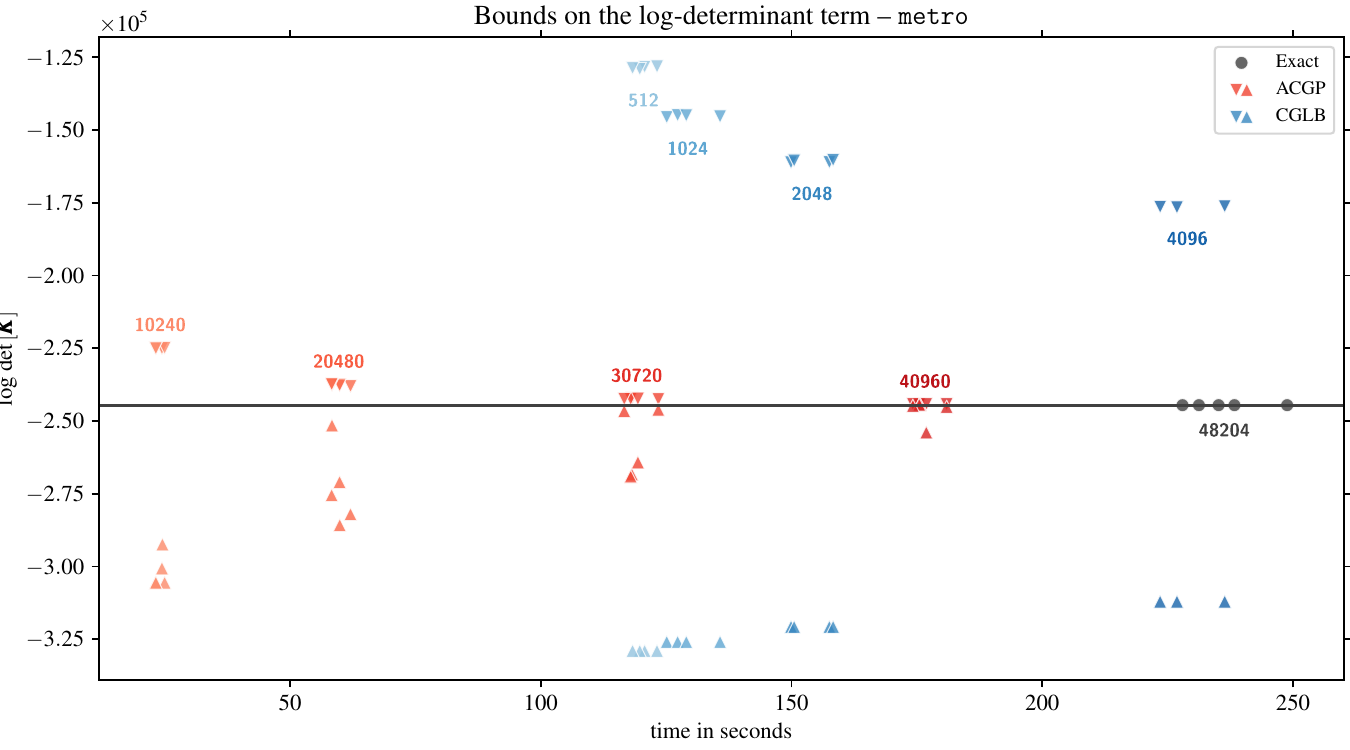}
		\subcaption{OU kernel, $\log\ell = 1$}
		\label{subfig:metro_ou_loget_1}
	\end{minipage}
	\begin{minipage}[b]{.5\textwidth}
		\centering
		\includegraphics[width=0.96\textwidth]{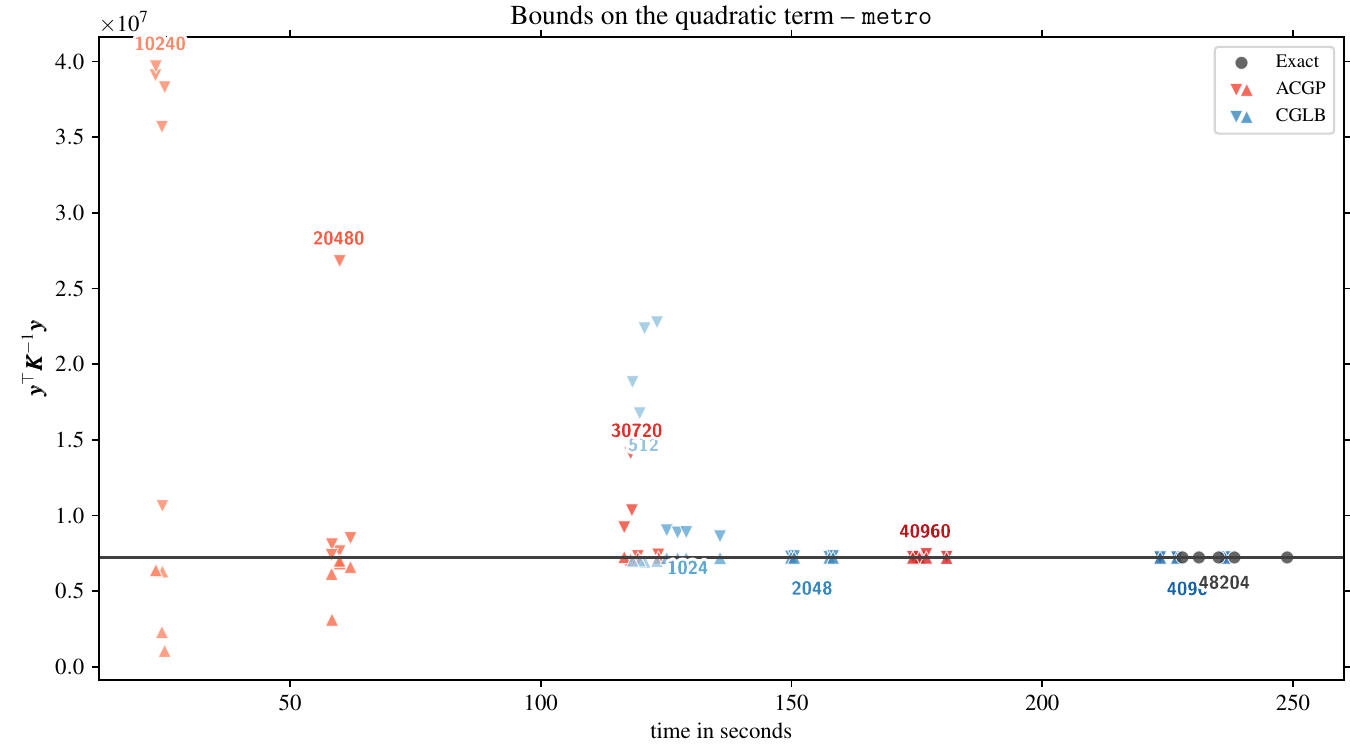}
		\subcaption{OU kernel, $\log\ell = 1$}
		\label{subfig:metro_ou_quadratic_1}
	\end{minipage}

	\begin{minipage}[b]{.5\textwidth}
		\centering
		\includegraphics[width=0.96\textwidth]{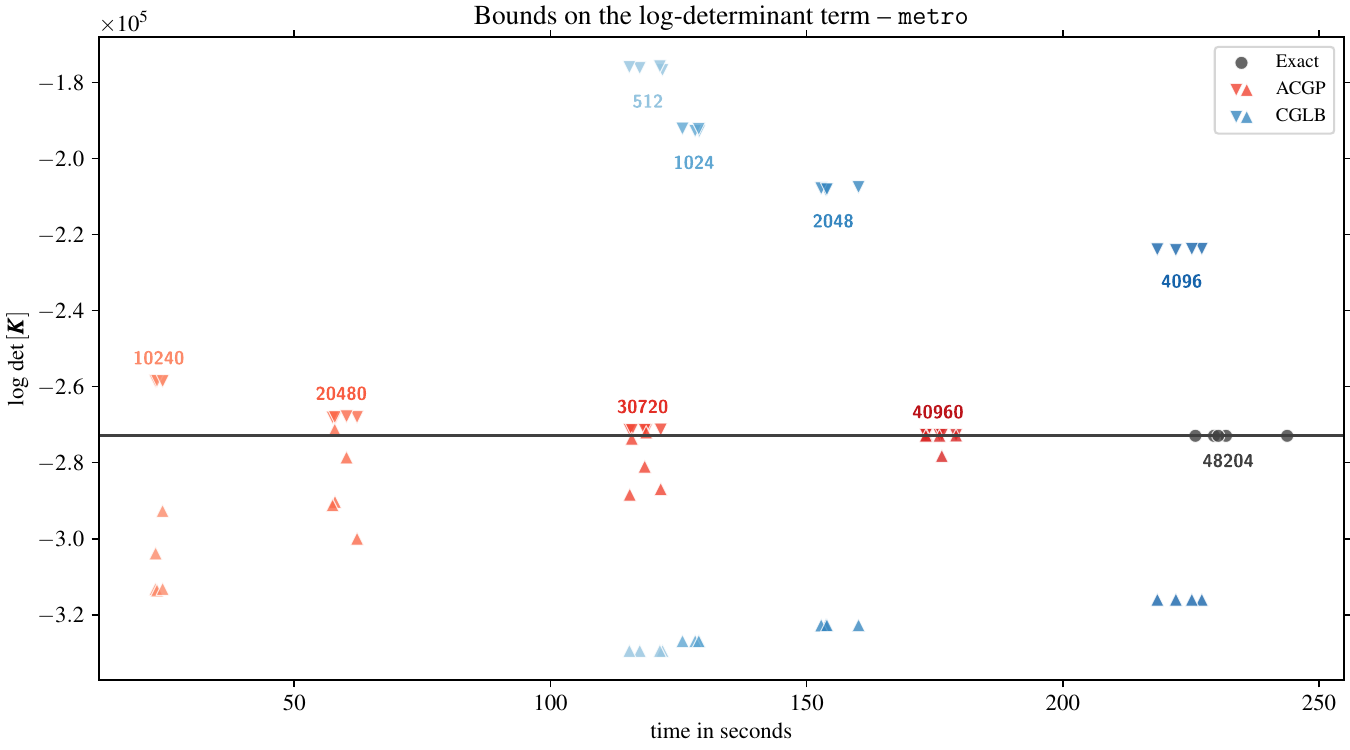}
		\subcaption{OU kernel, $\log\ell = 2$}
		\label{subfig:metro_ou_loget_2}
	\end{minipage}
	\begin{minipage}[b]{.5\textwidth}
		\centering
		\includegraphics[width=0.96\textwidth]{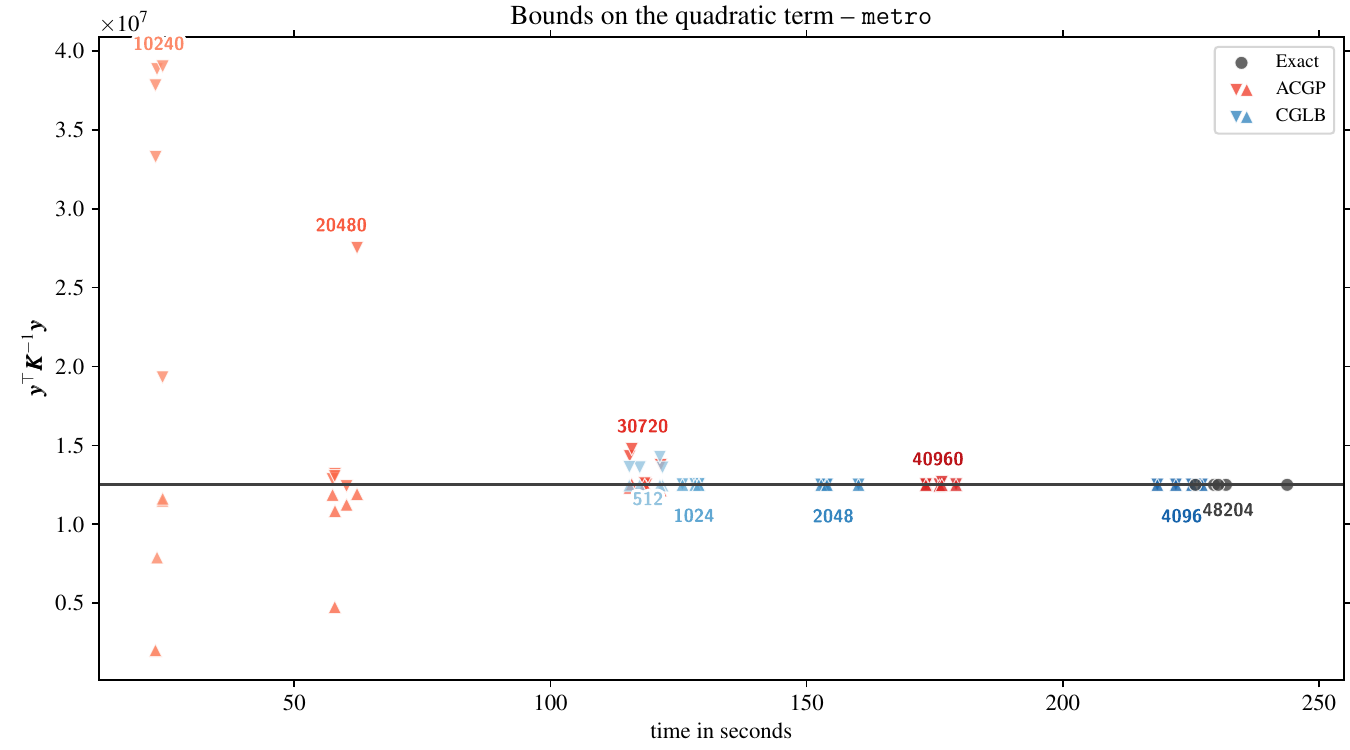}
		\subcaption{OU kernel, $\log\ell = 2$}
		\label{subfig:metro_ou_quadratic_2}
	\end{minipage}
    \caption{Upper and lower bounds on the log-determinant term (left column) and the quadratic term (right column) for the \texttt{metro} dataset using an Ornstein-Uhlenbeck (OU) kernel.}
	\label{fig:bounds_metro_ou}
\end{figure}

\clearpage
\subsubsection{Bounds for experiments on \texttt{pm25}}
\label{subsec:bounds_pm25}
\begin{figure}[htb!]
	\begin{minipage}[b]{.5\textwidth}
		\centering
		\includegraphics[width=0.96\textwidth]{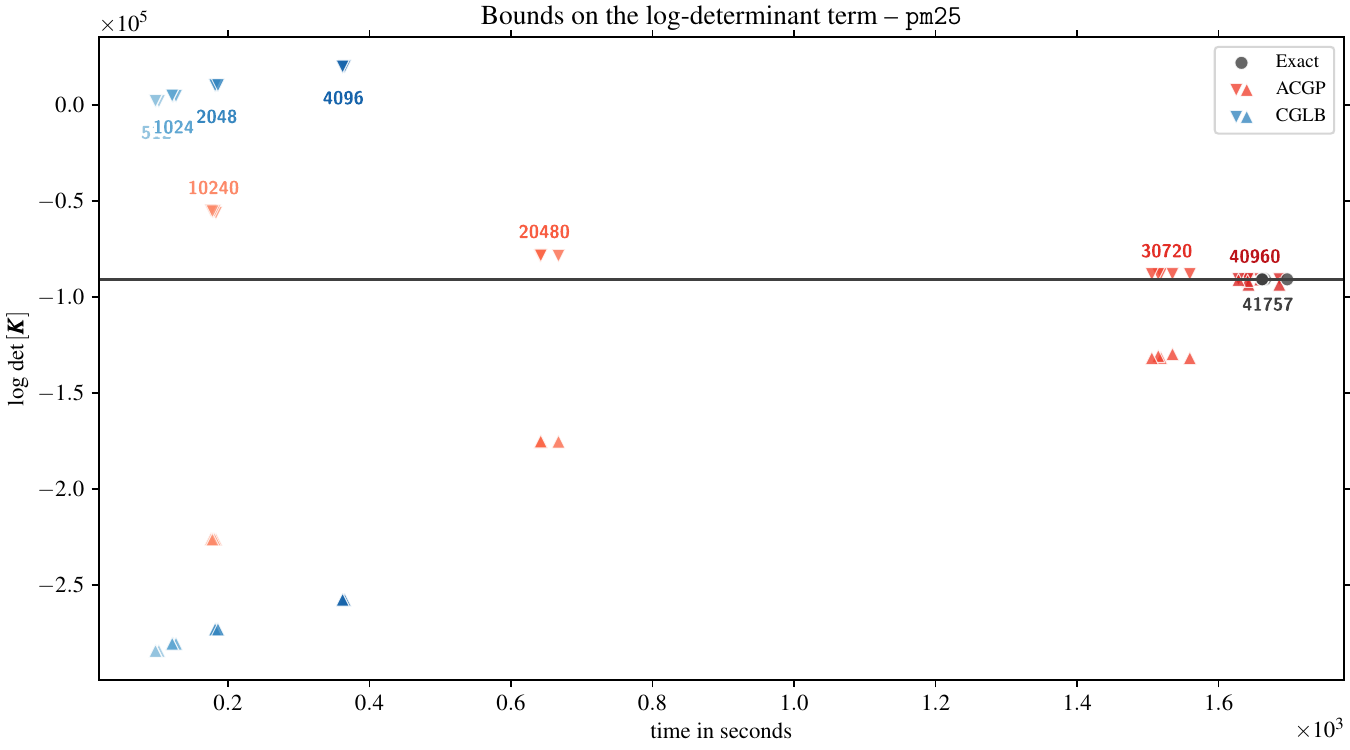}
		\subcaption{SE kernel, $\log\ell = -1$}
		\label{subfig:pm25_rbf_loget_-1}
	\end{minipage}
	\begin{minipage}[b]{.5\textwidth}
		\centering
		\includegraphics[width=0.96\textwidth]{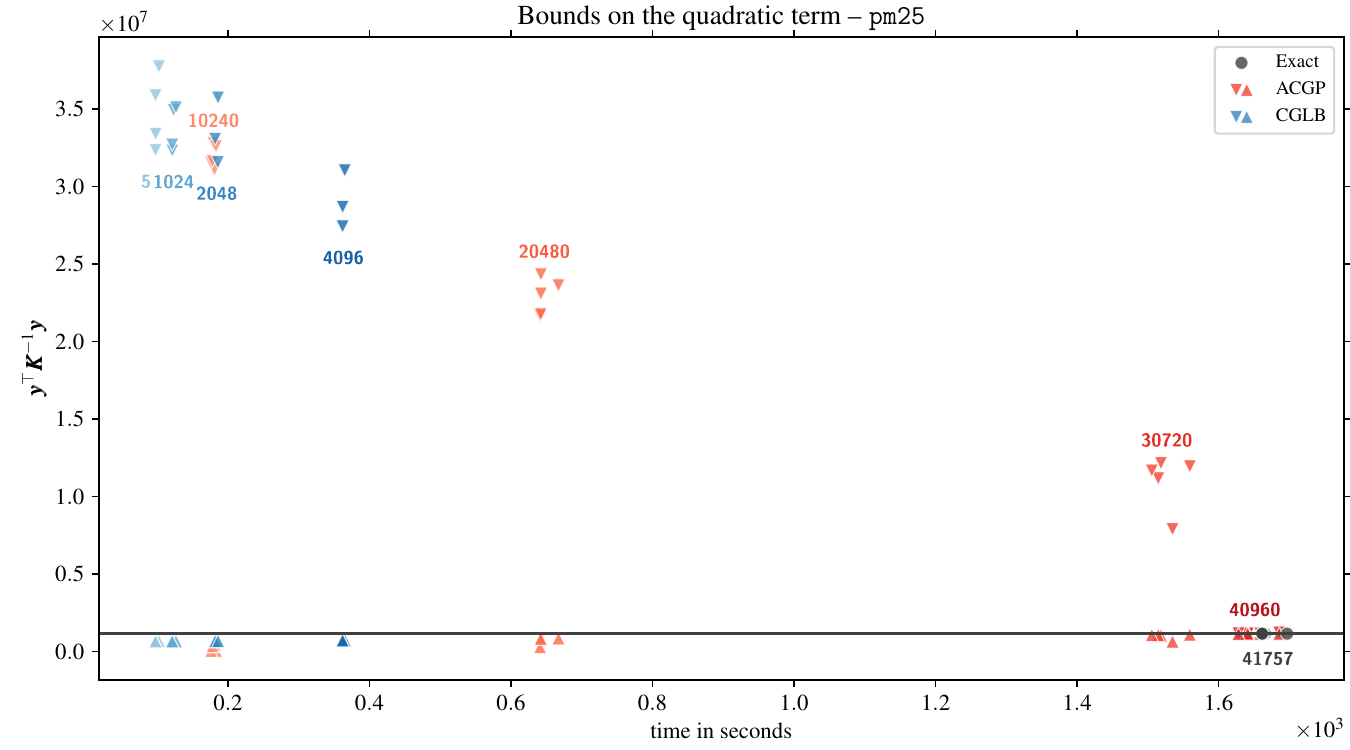}
		\subcaption{SE kernel, $\log\ell = -1$}
		\label{subfig:pm25_rbf_quadratic_-1}
	\end{minipage}

	\begin{minipage}[b]{.5\textwidth}
		\centering
		\includegraphics[width=0.96\textwidth]{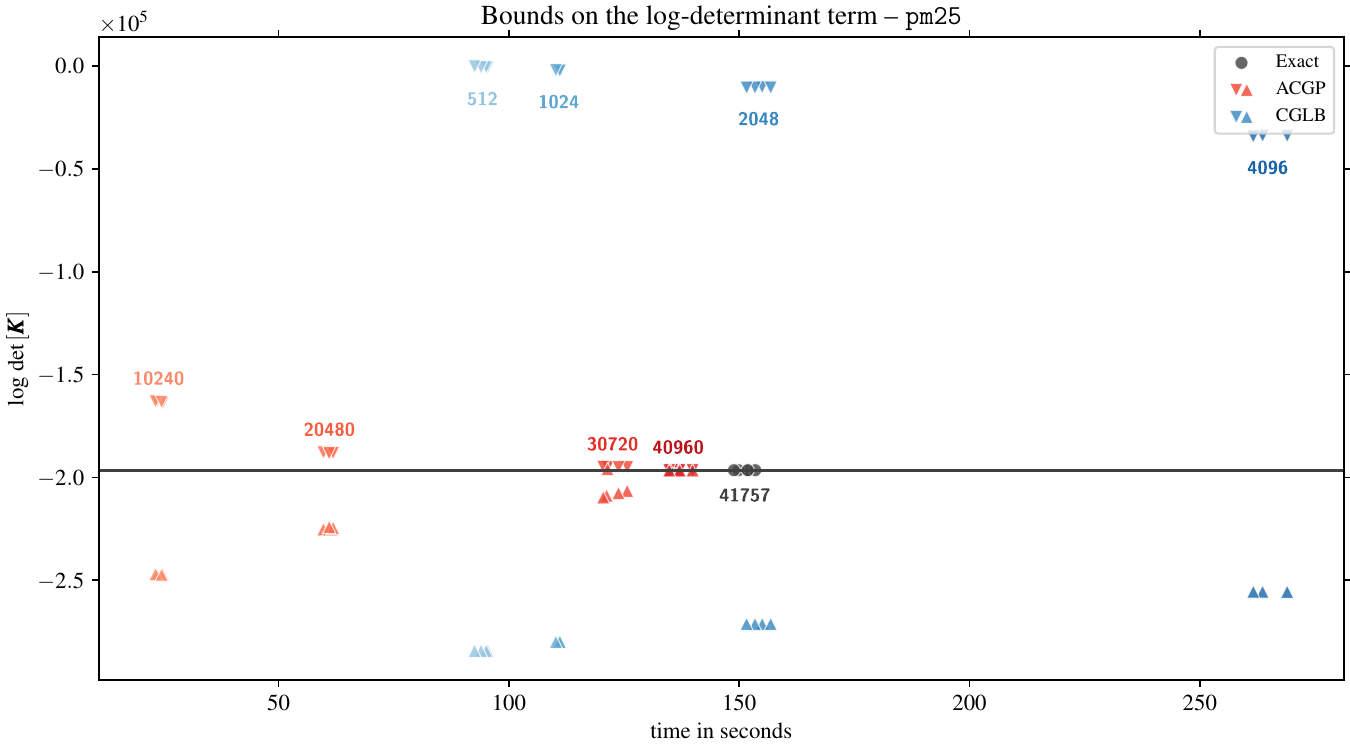}
		\subcaption{SE kernel, $\log\ell = 0$}
		\label{subfig:pm25_rbf_loget_0}
	\end{minipage}
	\begin{minipage}[b]{.5\textwidth}
		\centering
		\includegraphics[width=0.96\textwidth]{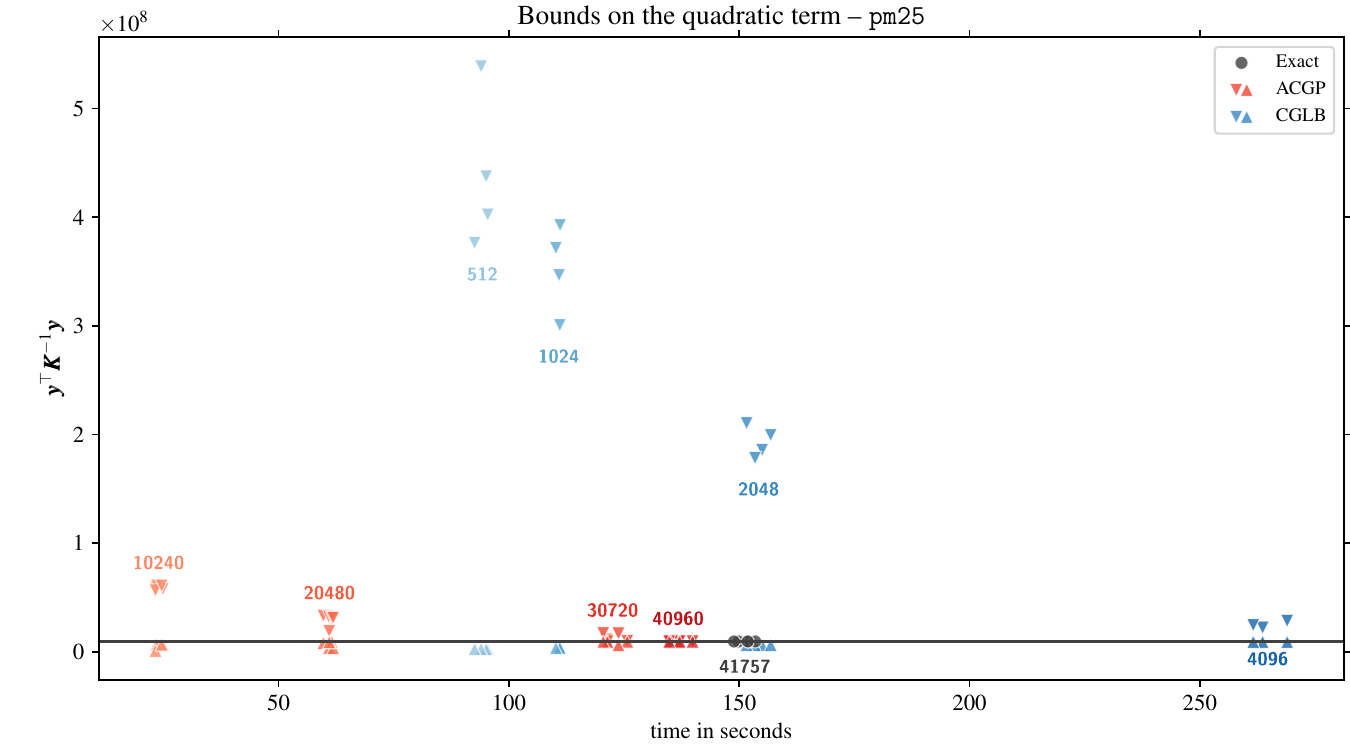}
		\subcaption{SE kernel, $\log\ell = 0$}
		\label{subfig:pm25_rbf_quadratic_0}
	\end{minipage}

	\begin{minipage}[b]{.5\textwidth}
		\centering
		\includegraphics[width=0.96\textwidth]{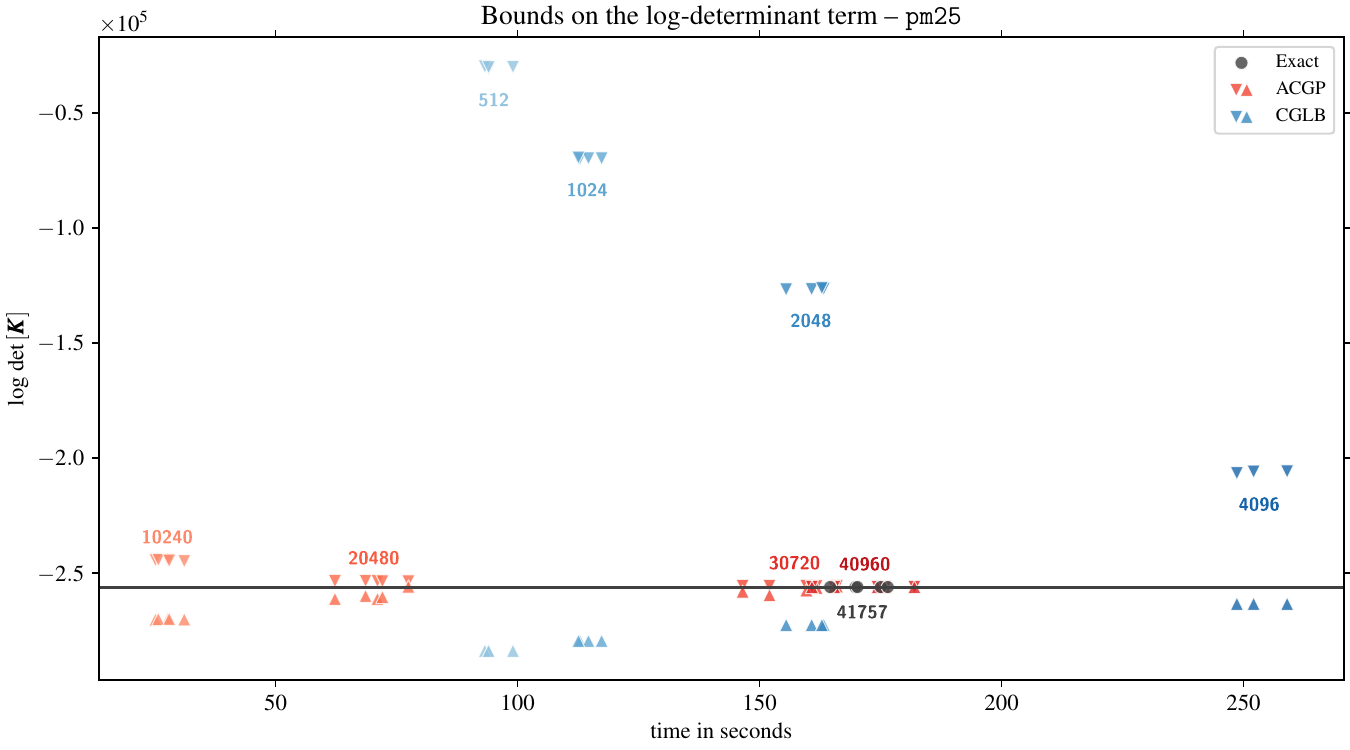}
		\subcaption{SE kernel, $\log\ell = 1$}
		\label{subfig:pm25_rbf_loget_1}
	\end{minipage}
	\begin{minipage}[b]{.5\textwidth}
		\centering
		\includegraphics[width=0.96\textwidth]{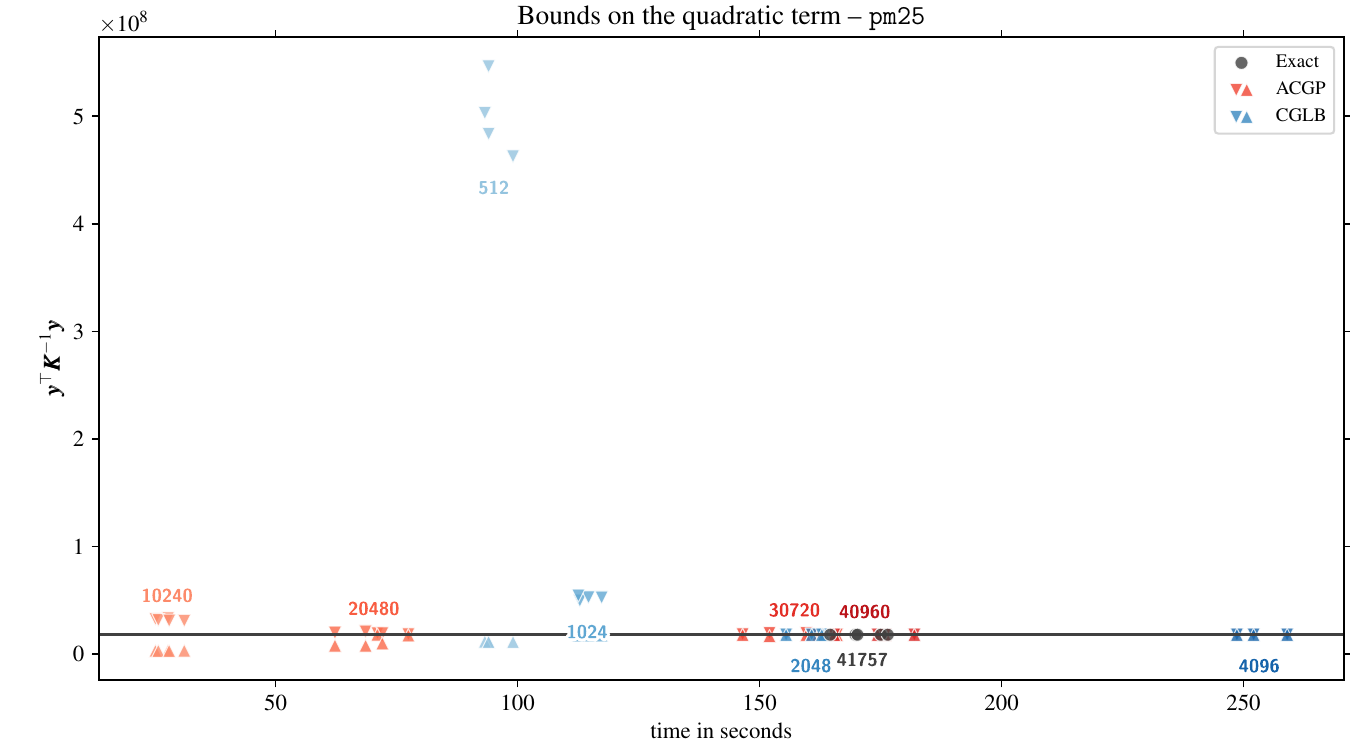}
		\subcaption{SE kernel, $\log\ell = 1$}
		\label{subfig:pm25_rbf_quadratic_1}
	\end{minipage}

	\begin{minipage}[b]{.5\textwidth}
		\centering
		\includegraphics[width=0.96\textwidth]{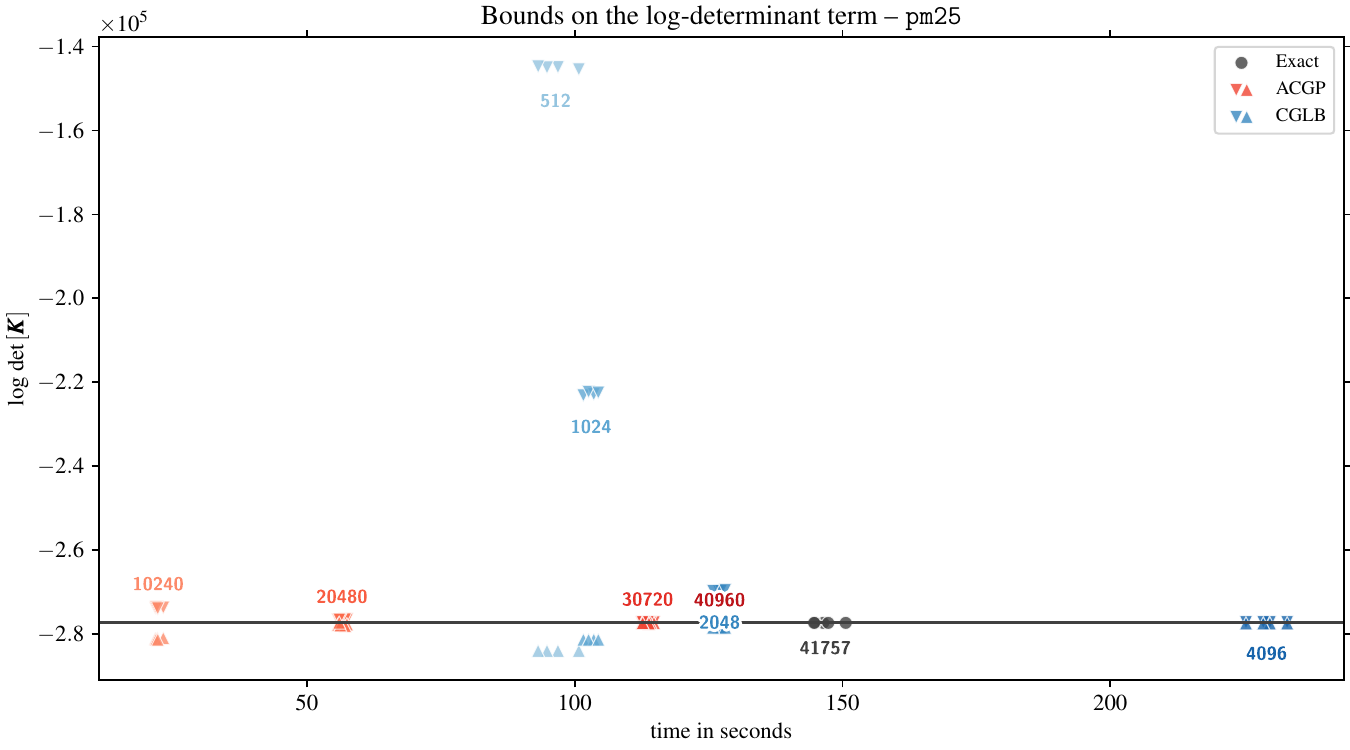}
		\subcaption{SE kernel, $\log\ell = 2$}
		\label{subfig:pm25_rbf_loget_2}
	\end{minipage}
	\begin{minipage}[b]{.5\textwidth}
		\centering
		\includegraphics[width=0.96\textwidth]{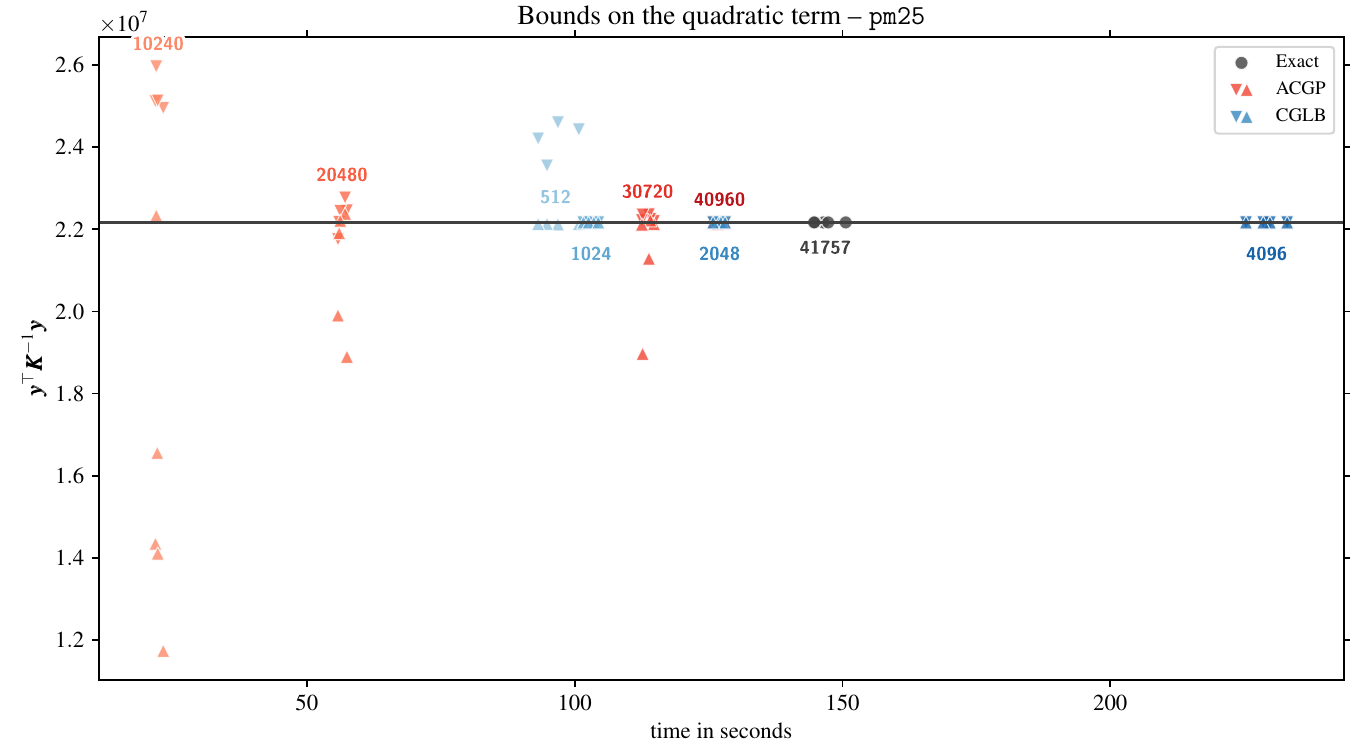}
		\subcaption{SE kernel, $\log\ell = 2$}
		\label{subfig:pm25_rbf_quadratic_2}
	\end{minipage}
    \caption{Upper and lower bounds on the log-determinant term (left column) and the quadratic term (right column) for the \texttt{pm25} dataset.}
	\label{fig:bounds_pm25_rbf}
\end{figure}
\begin{figure}[htb]
	\begin{minipage}[b]{.5\textwidth}
		\centering
		\includegraphics[width=0.96\textwidth]{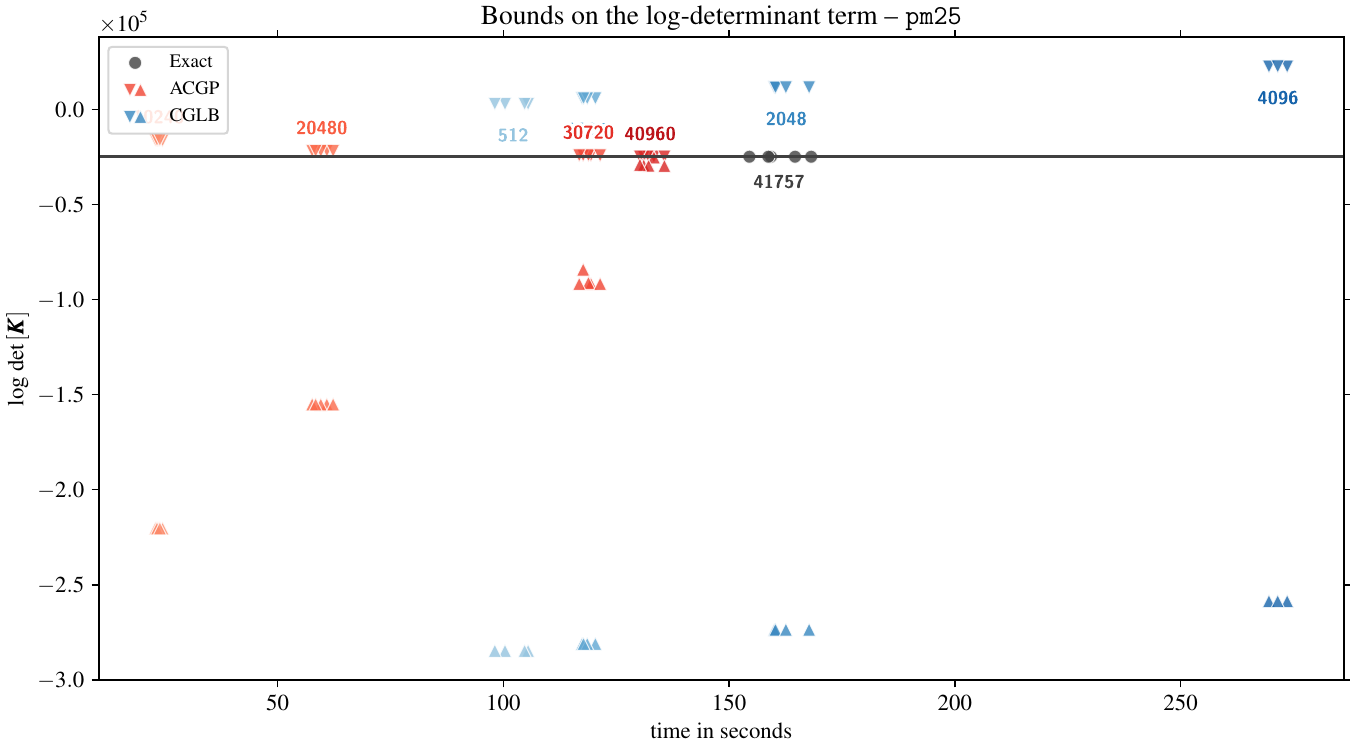}
		\subcaption{OU kernel, $\log\ell = -1$}
		\label{subfig:pm25_ou_loget_-1}
	\end{minipage}
	\begin{minipage}[b]{.5\textwidth}
		\centering
		\includegraphics[width=0.96\textwidth]{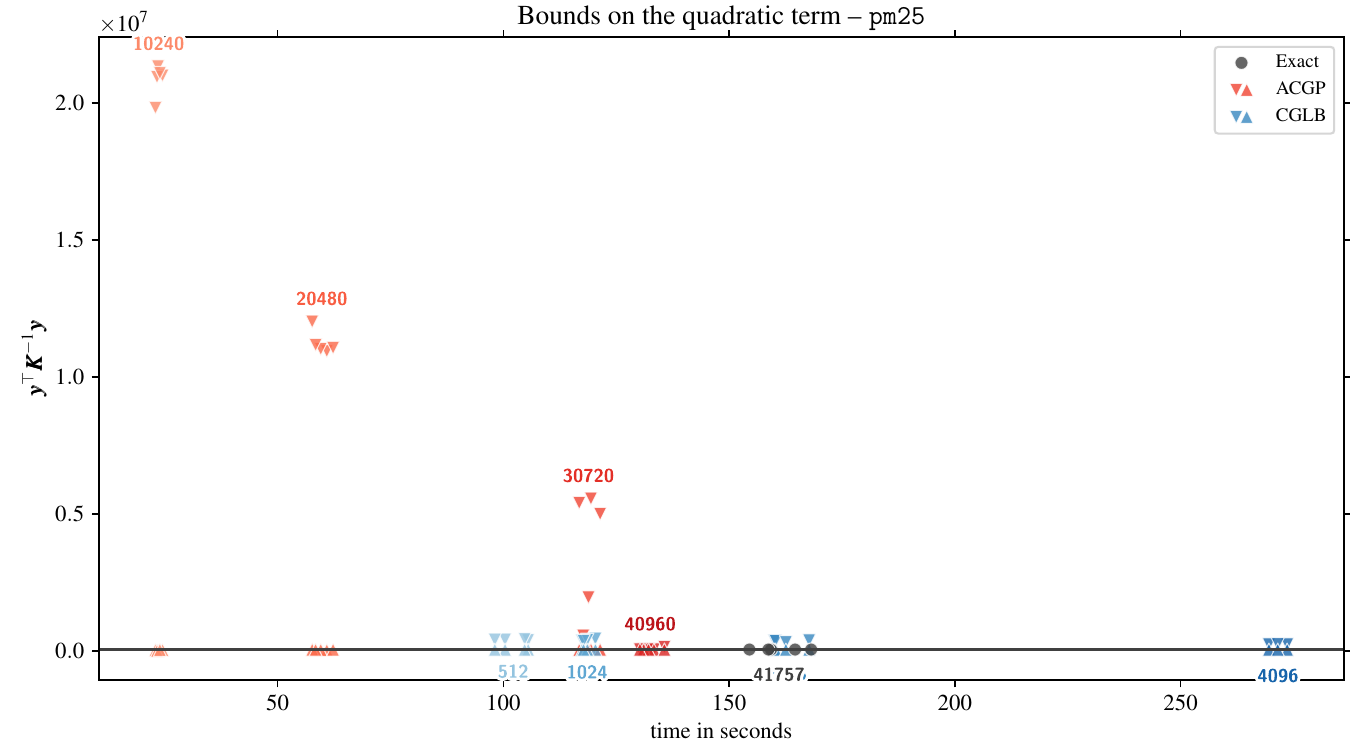}
		\subcaption{OU kernel, $\log\ell = -1$}
		\label{subfig:pm25_ou_quadratic_-1}
	\end{minipage}

	\begin{minipage}[b]{.5\textwidth}
		\centering
		\includegraphics[width=0.96\textwidth]{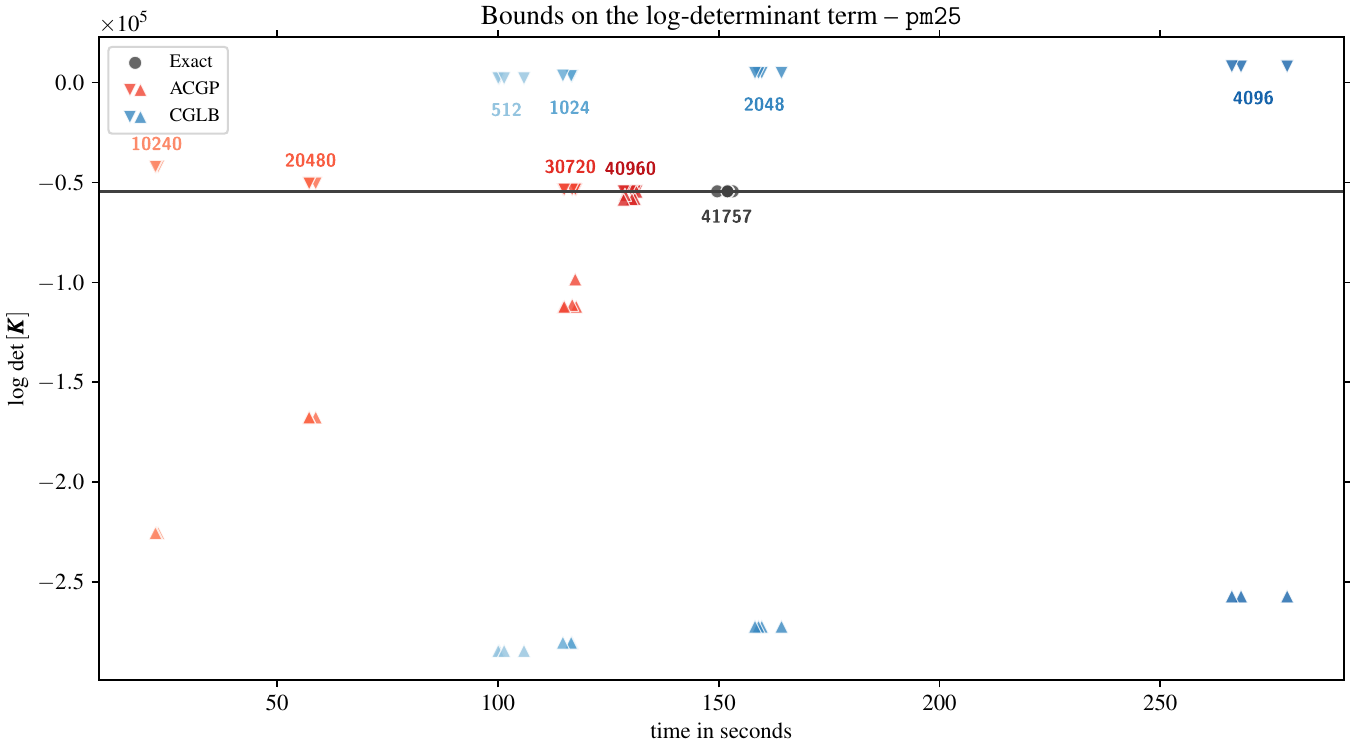}
		\subcaption{OU kernel, $\log\ell = 0$}
		\label{subfig:pm25_ou_loget_0}
	\end{minipage}
	\begin{minipage}[b]{.5\textwidth}
		\centering
		\includegraphics[width=0.96\textwidth]{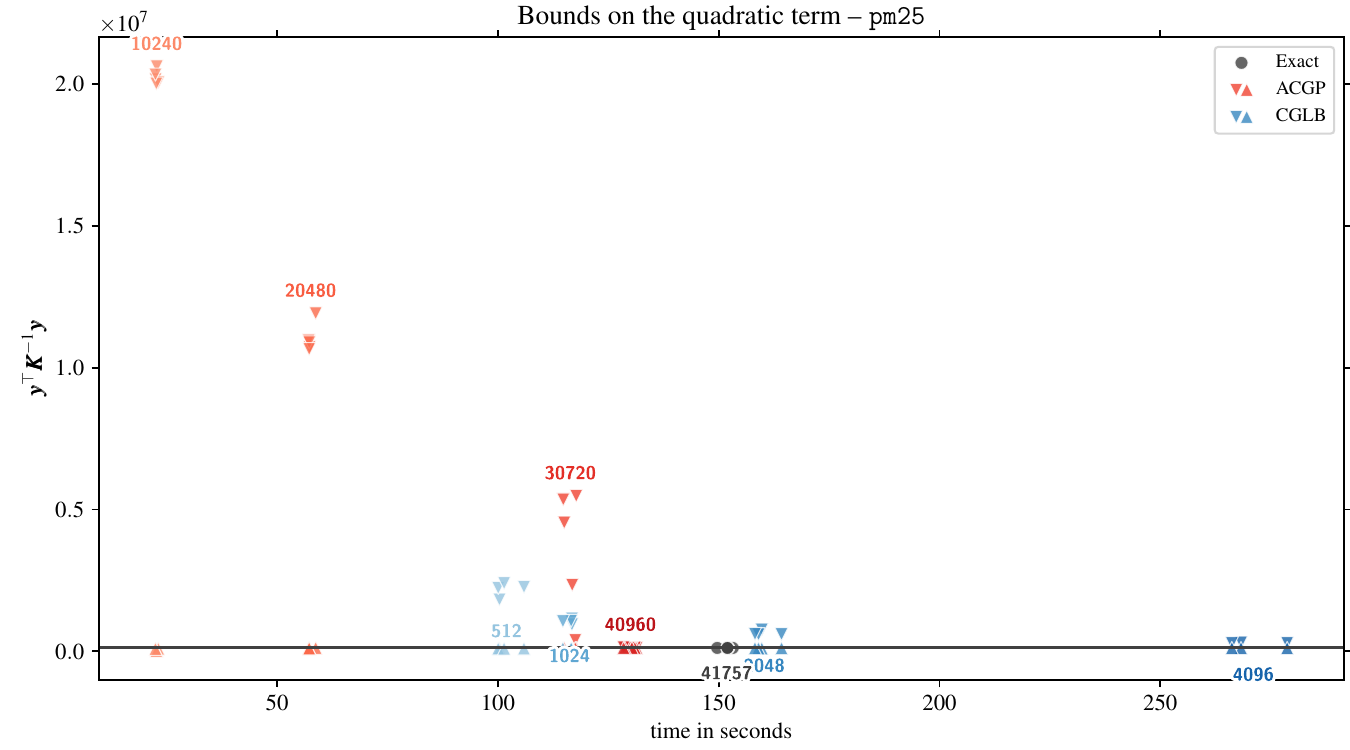}
		\subcaption{OU kernel, $\log\ell = 0$}
		\label{subfig:pm25_ou_quadratic_0}
	\end{minipage}

	\begin{minipage}[b]{.5\textwidth}
		\centering
		\includegraphics[width=0.96\textwidth]{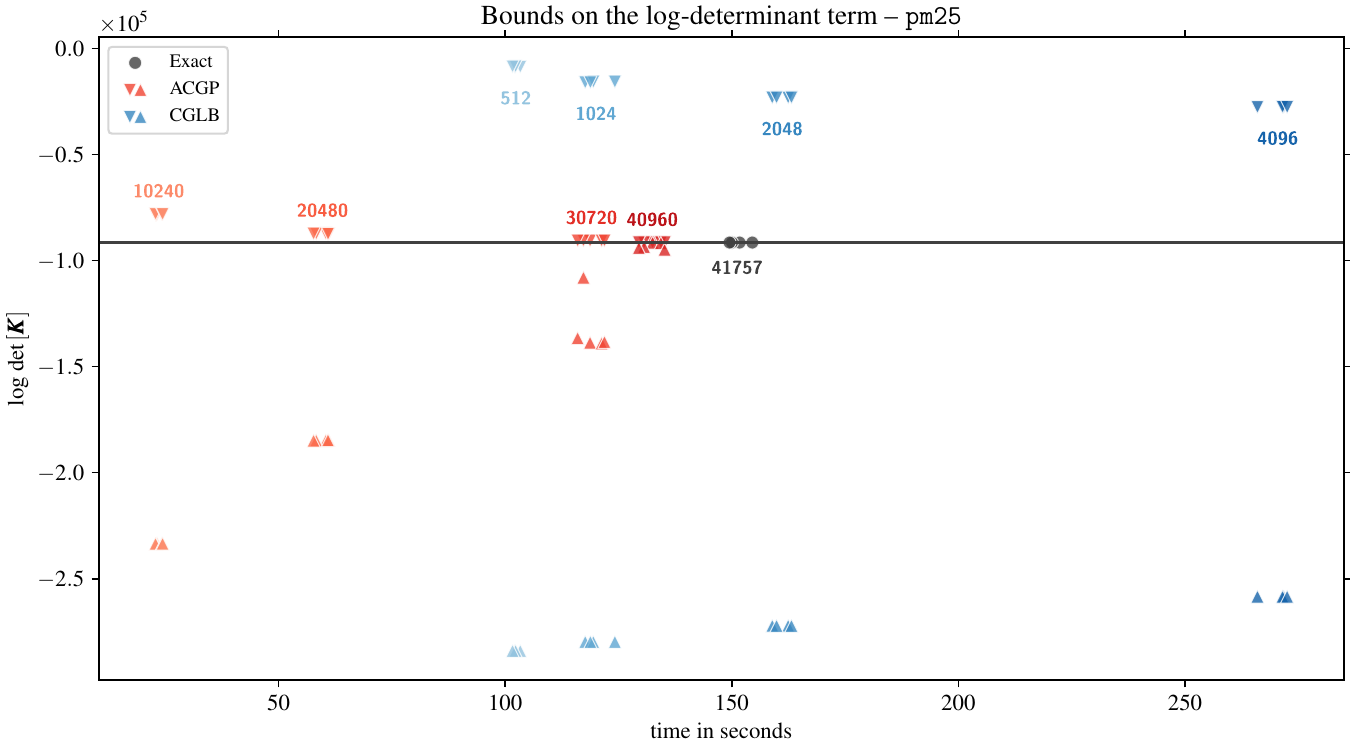}
		\subcaption{OU kernel, $\log\ell = 1$}
		\label{subfig:pm25_ou_loget_1}
	\end{minipage}
	\begin{minipage}[b]{.5\textwidth}
		\centering
		\includegraphics[width=0.96\textwidth]{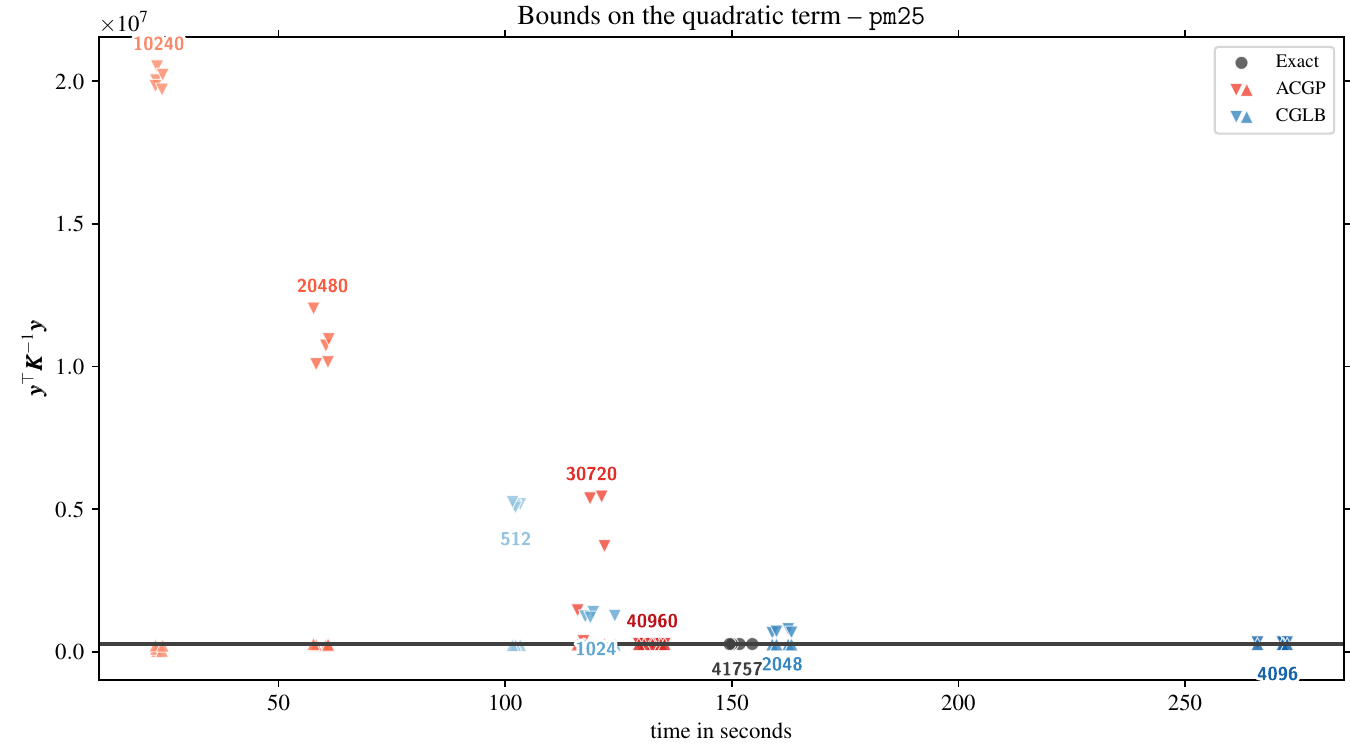}
		\subcaption{OU kernel, $\log\ell = 1$}
		\label{subfig:pm25_ou_quadratic_1}
	\end{minipage}

	\begin{minipage}[b]{.5\textwidth}
		\centering
		\includegraphics[width=0.96\textwidth]{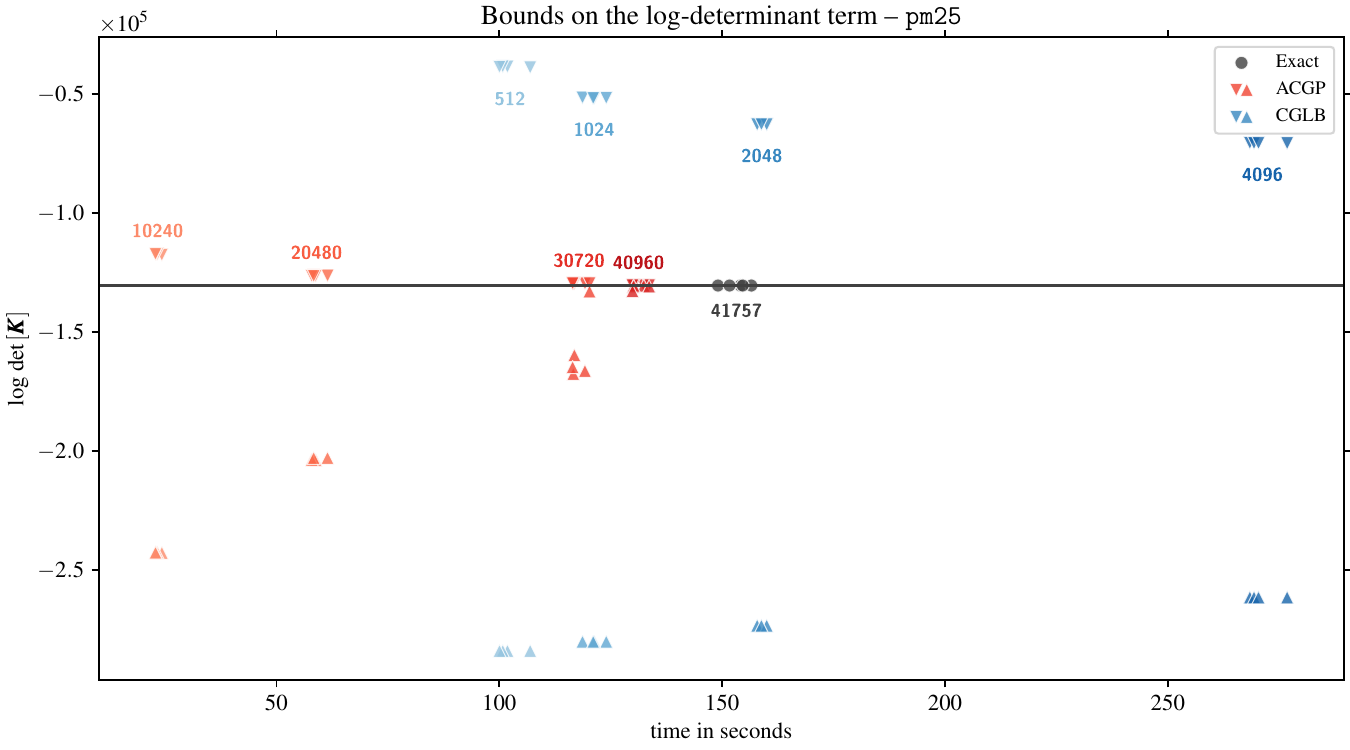}
		\subcaption{OU kernel, $\log\ell = 2$}
		\label{subfig:pm25_ou_loget_2}
	\end{minipage}
	\begin{minipage}[b]{.5\textwidth}
		\centering
		\includegraphics[width=0.96\textwidth]{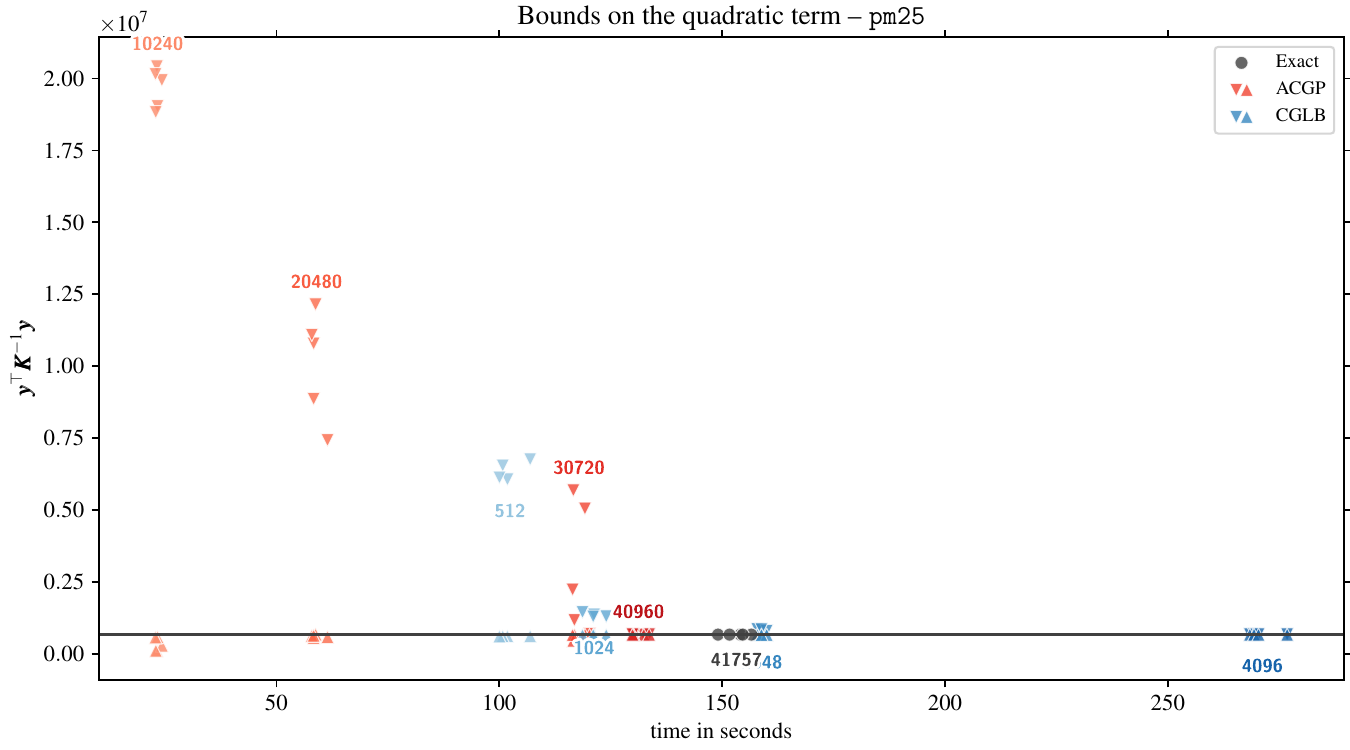}
		\subcaption{OU kernel, $\log\ell = 2$}
		\label{subfig:pm25_ou_quadratic_2}
	\end{minipage}
    \caption{Upper and lower bounds on the log-determinant term (left column) and the quadratic term (right column) for the \texttt{pm25} dataset using an Ornstein-Uhlenbeck (OU) kernel.}
	\label{fig:bounds_pm25_ou}
\end{figure}

\clearpage
\subsubsection{Bounds for experiments on \texttt{protein}}
\label{subsec:bounds_protein}
\begin{figure}[htb!]
	\begin{minipage}[b]{.5\textwidth}
		\centering
		\includegraphics[width=0.96\textwidth]{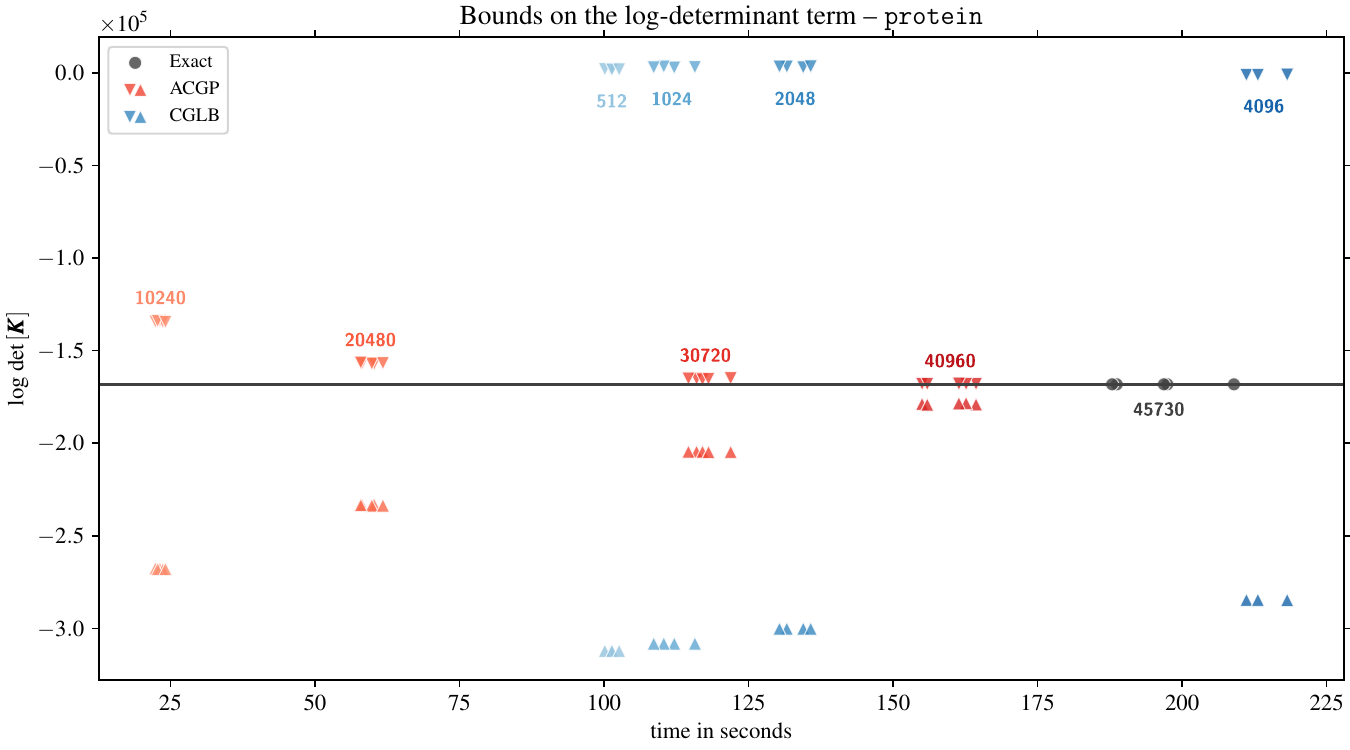}
		\subcaption{SE kernel, $\log\ell = -1$}
		\label{subfig:protein_rbf_loget_-1}
	\end{minipage}
	\begin{minipage}[b]{.5\textwidth}
		\centering
		\includegraphics[width=0.96\textwidth]{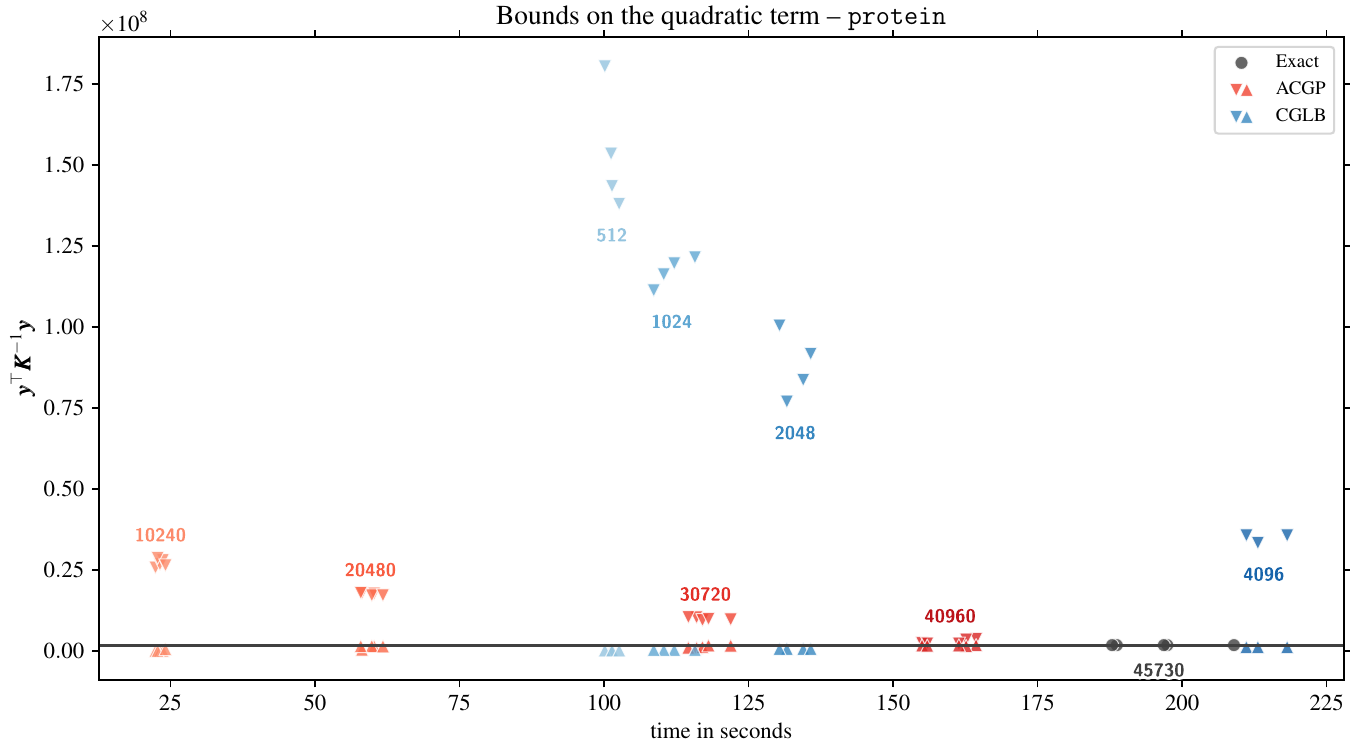}
		\subcaption{SE kernel, $\log\ell = -1$}
		\label{subfig:protein_rbf_quadratic_-1}
	\end{minipage}

	\begin{minipage}[b]{.5\textwidth}
		\centering
		\includegraphics[width=0.96\textwidth]{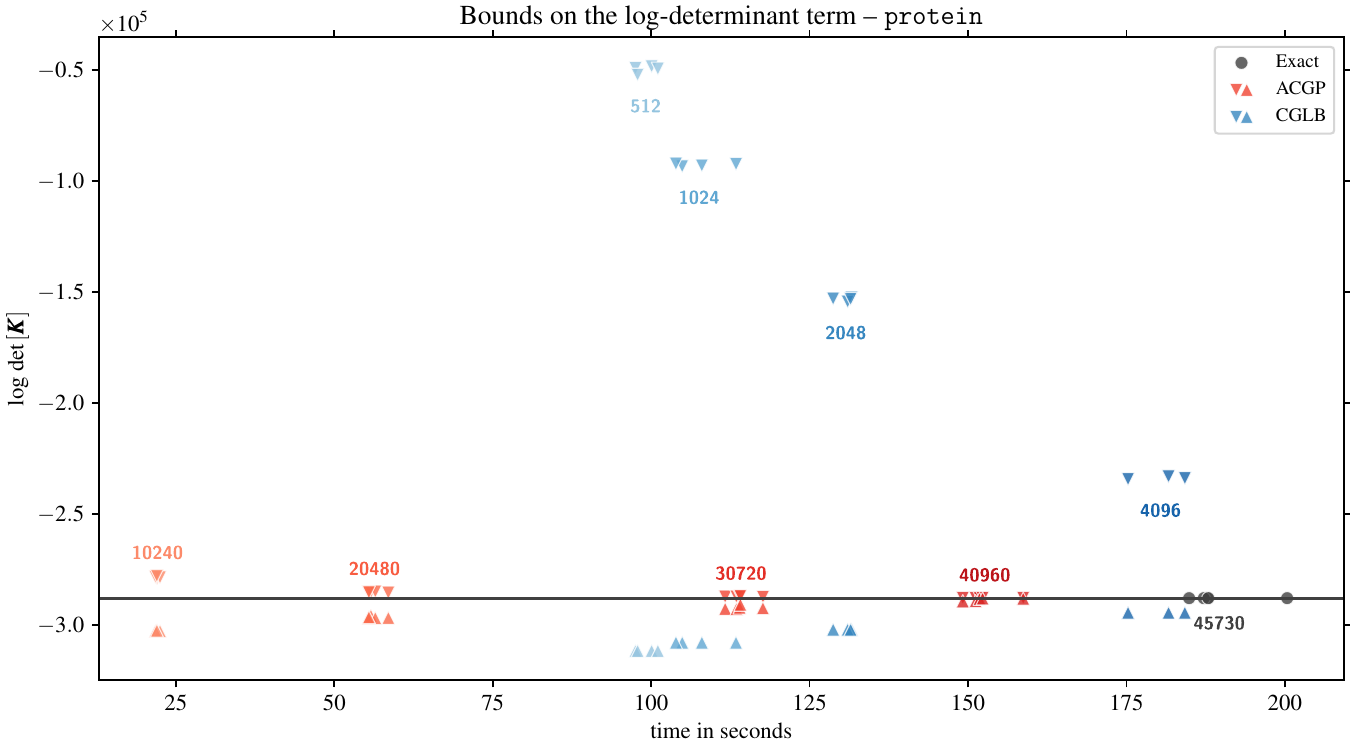}
		\subcaption{SE kernel, $\log\ell = 0$}
		\label{subfig:protein_rbf_loget_0}
	\end{minipage}
	\begin{minipage}[b]{.5\textwidth}
		\centering
		\includegraphics[width=0.96\textwidth]{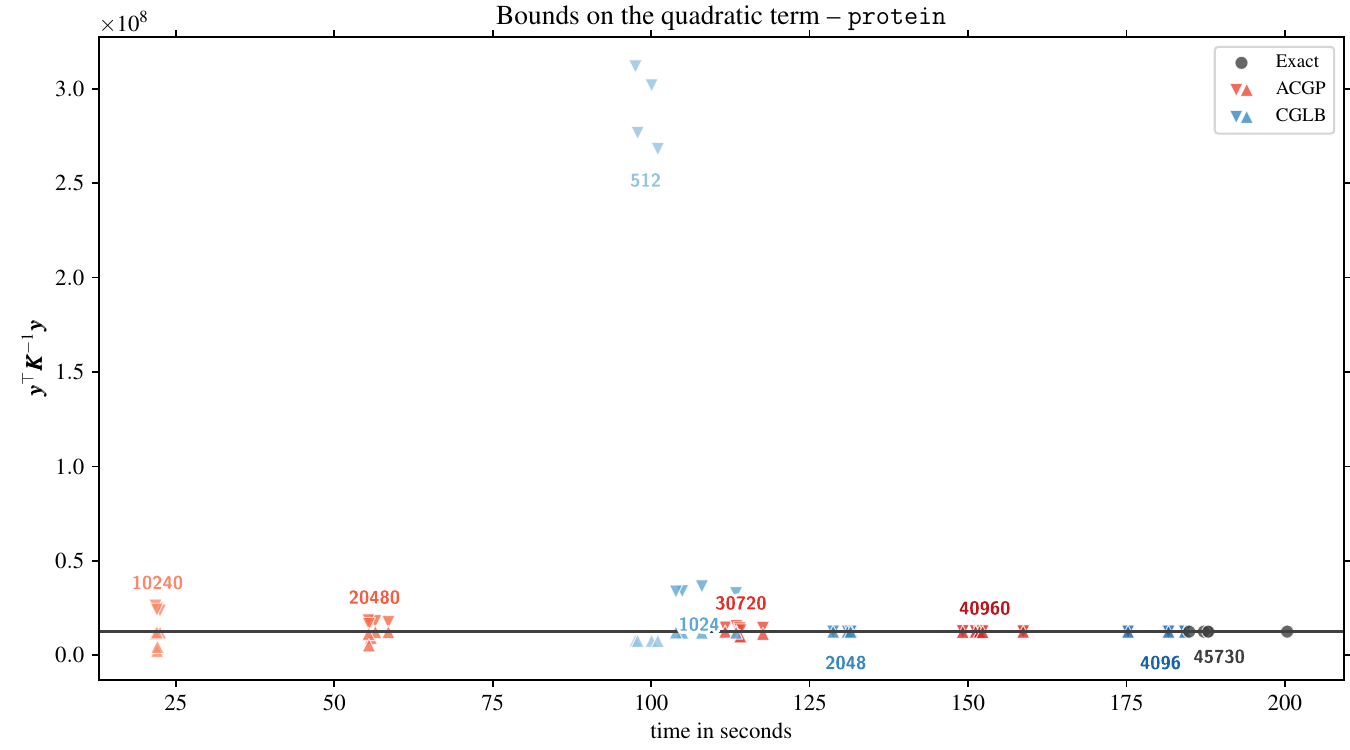}
		\subcaption{SE kernel, $\log\ell = 0$}
		\label{subfig:protein_rbf_quadratic_0}
	\end{minipage}

	\begin{minipage}[b]{.5\textwidth}
		\centering
		\includegraphics[width=0.96\textwidth]{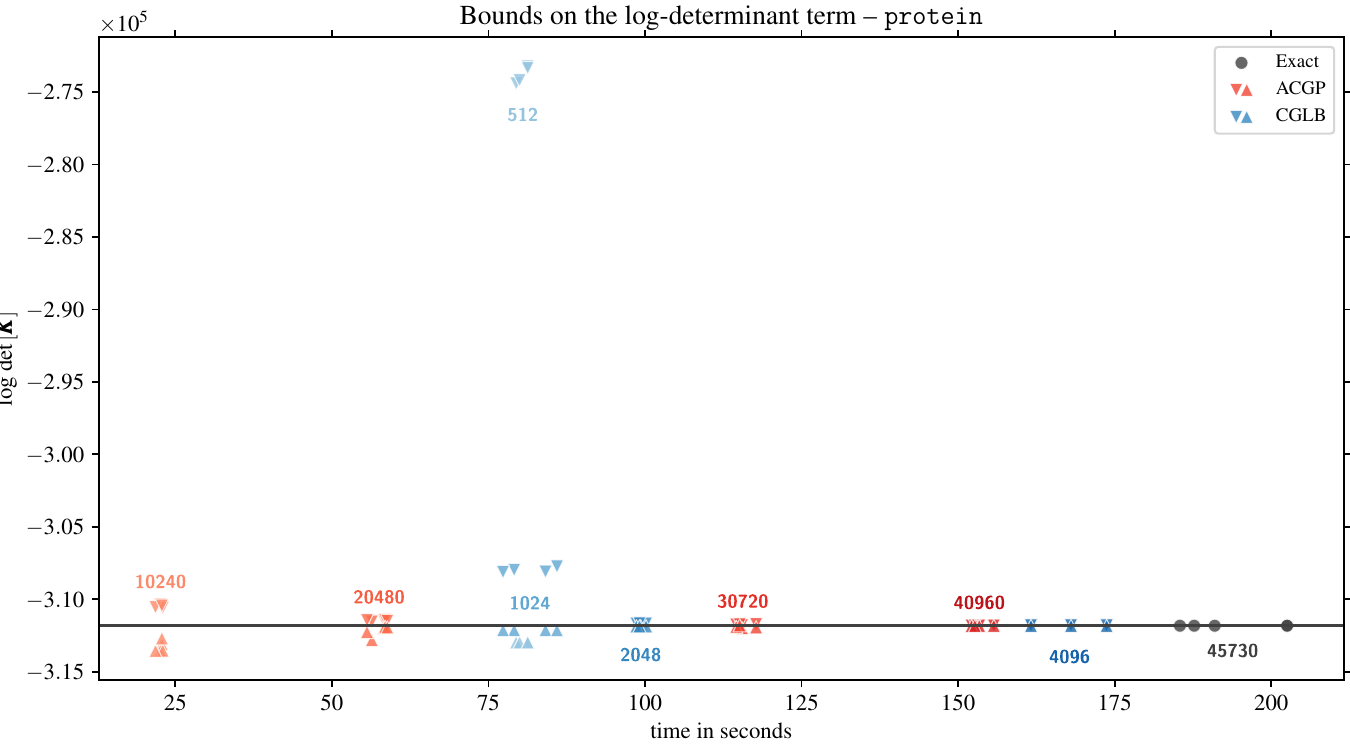}
		\subcaption{SE kernel, $\log\ell = 1$}
		\label{subfig:protein_rbf_loget_1}
	\end{minipage}
	\begin{minipage}[b]{.5\textwidth}
		\centering
		\includegraphics[width=0.96\textwidth]{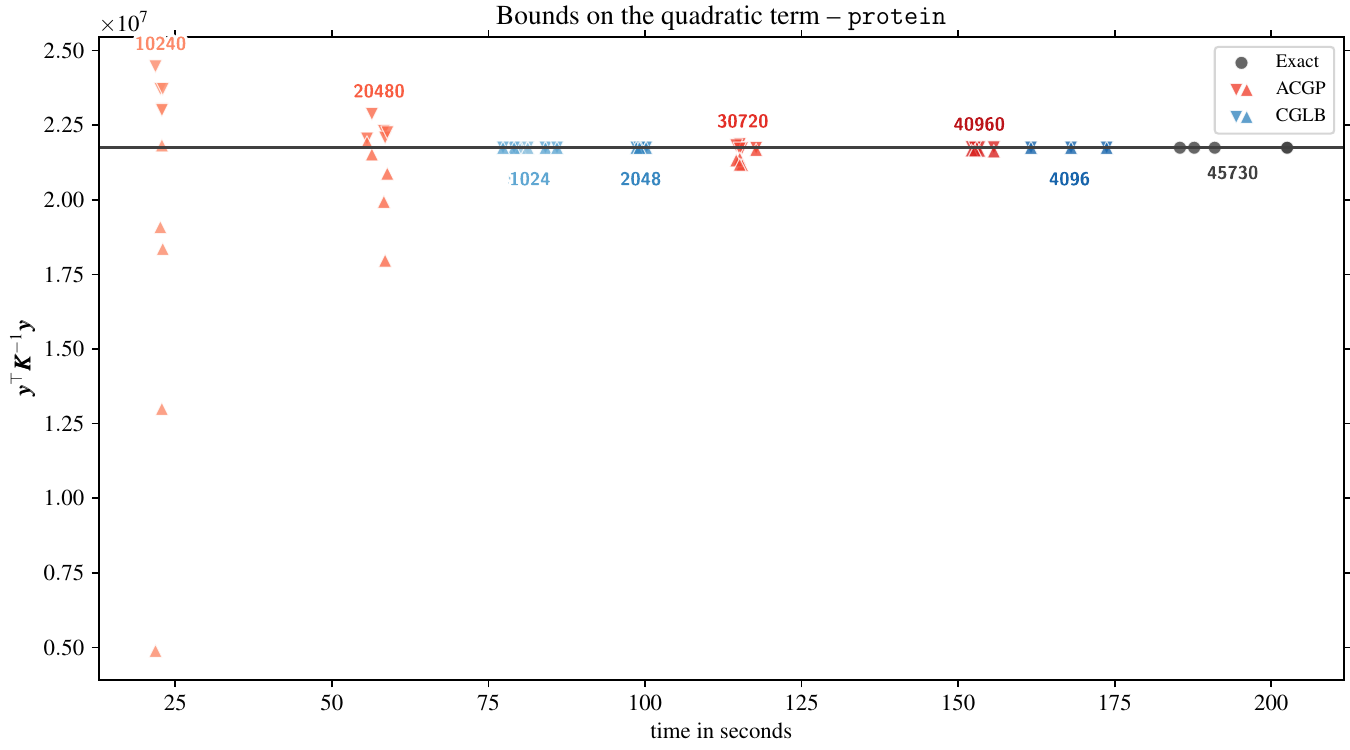}
		\subcaption{SE kernel, $\log\ell = 1$}
		\label{subfig:protein_rbf_quadratic_1}
	\end{minipage}

	\begin{minipage}[b]{.5\textwidth}
		\centering
		\includegraphics[width=0.96\textwidth]{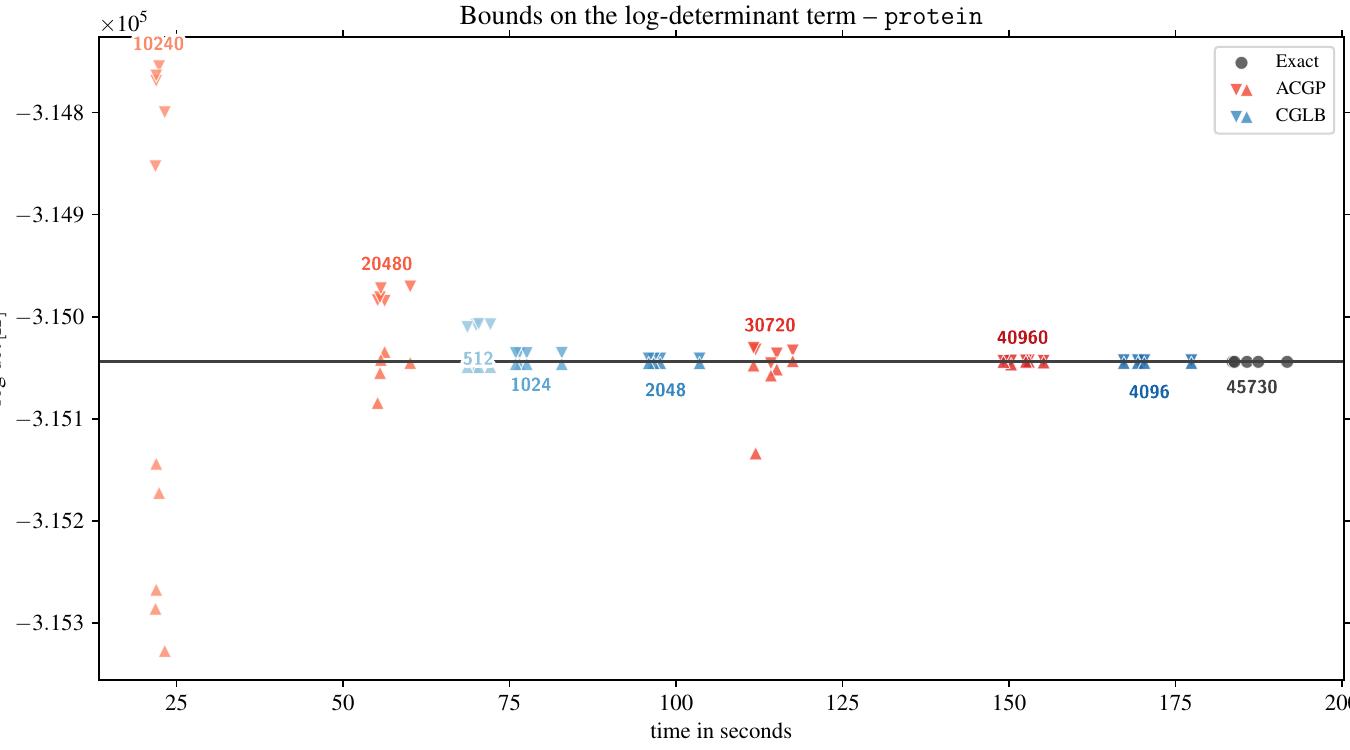}
		\subcaption{SE kernel, $\log\ell = 2$}
		\label{subfig:protein_rbf_loget_2}
	\end{minipage}
	\begin{minipage}[b]{.5\textwidth}
		\centering
		\includegraphics[width=0.96\textwidth]{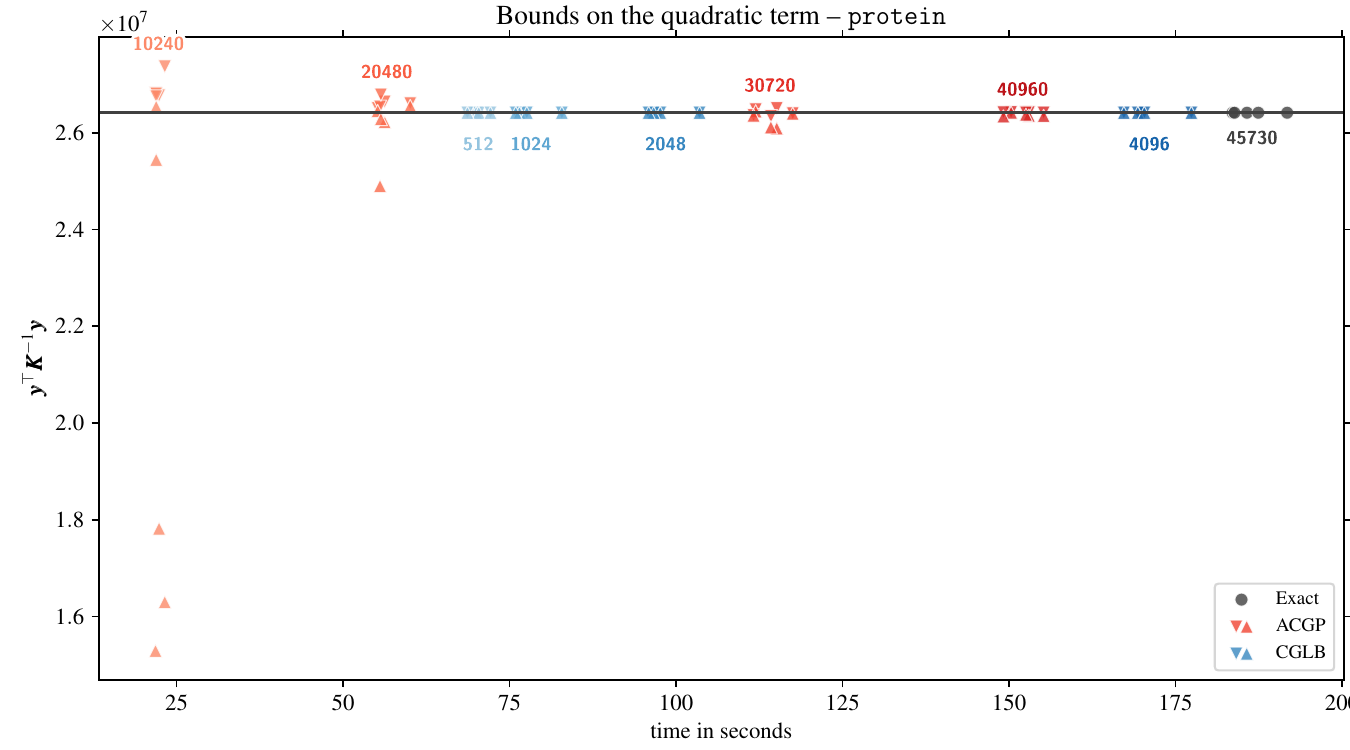}
		\subcaption{SE kernel, $\log\ell = 2$}
		\label{subfig:protein_rbf_quadratic_2}
	\end{minipage}
    \caption{Upper and lower bounds on the log-determinant term (left column) and the quadratic term (right column) for the \texttt{protein} dataset.}
	\label{fig:bounds_protein_rbf}
\end{figure}

\begin{figure}[htb]
	\begin{minipage}[b]{.5\textwidth}
		\centering
		\includegraphics[width=0.96\textwidth]{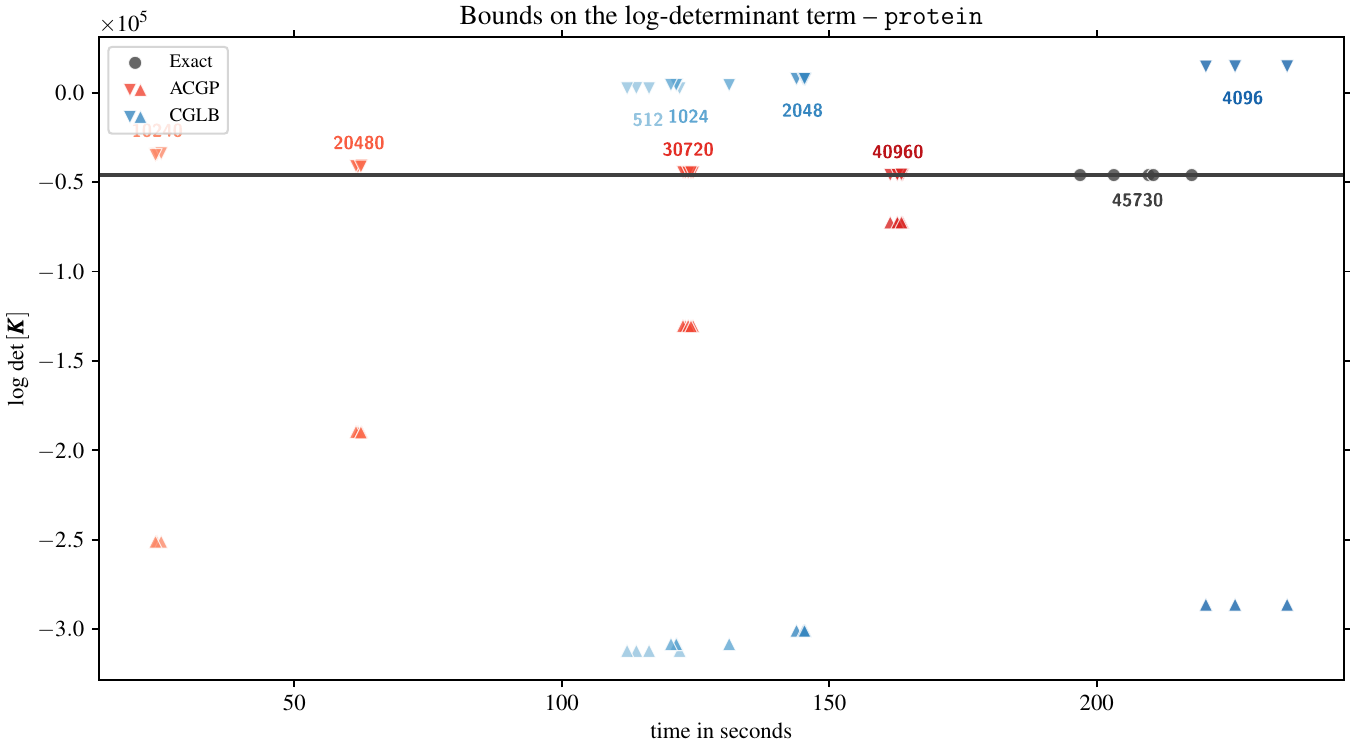}
		\subcaption{OU kernel, $\log\ell = -1$}
		\label{subfig:protein_ou_loget_-1}
	\end{minipage}
	\begin{minipage}[b]{.5\textwidth}
		\centering
		\includegraphics[width=0.96\textwidth]{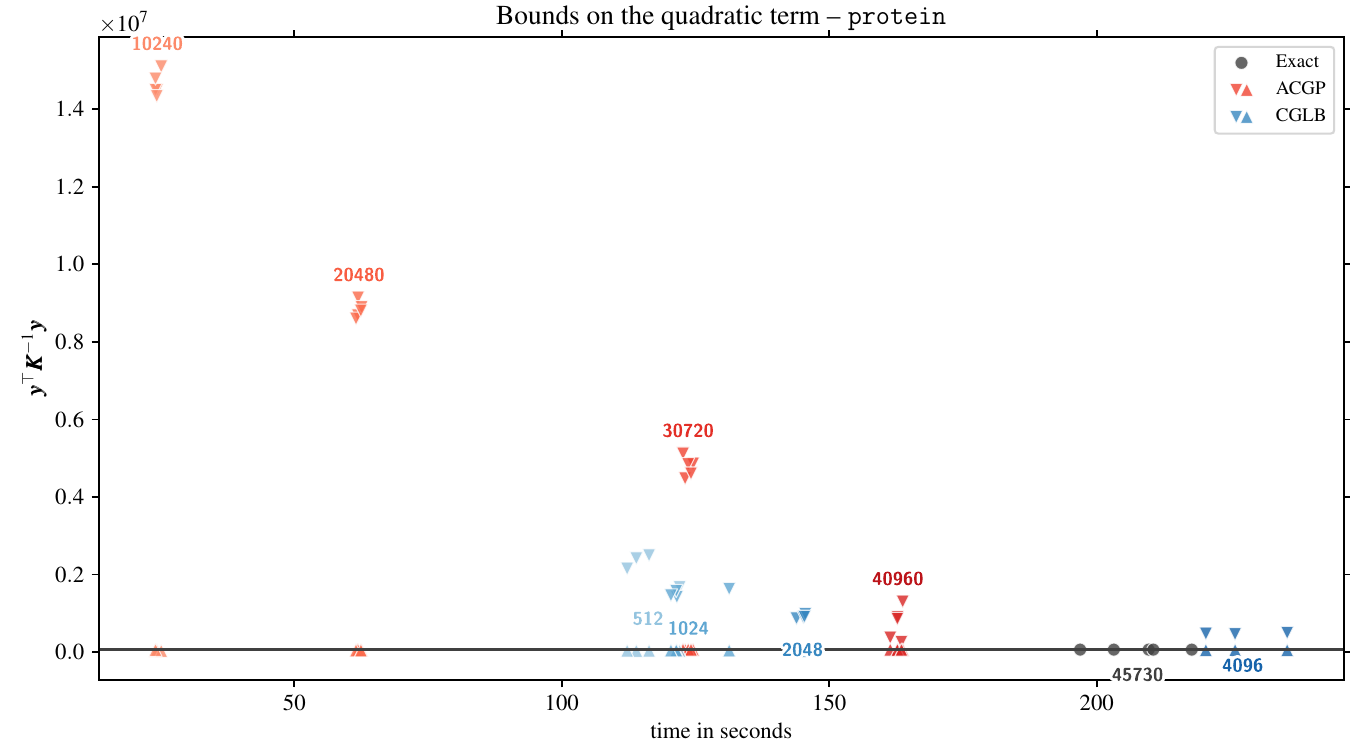}
		\subcaption{OU kernel, $\log\ell = -1$}
		\label{subfig:protein_ou_quadratic_-1}
	\end{minipage}

	\begin{minipage}[b]{.5\textwidth}
		\centering
		\includegraphics[width=0.96\textwidth]{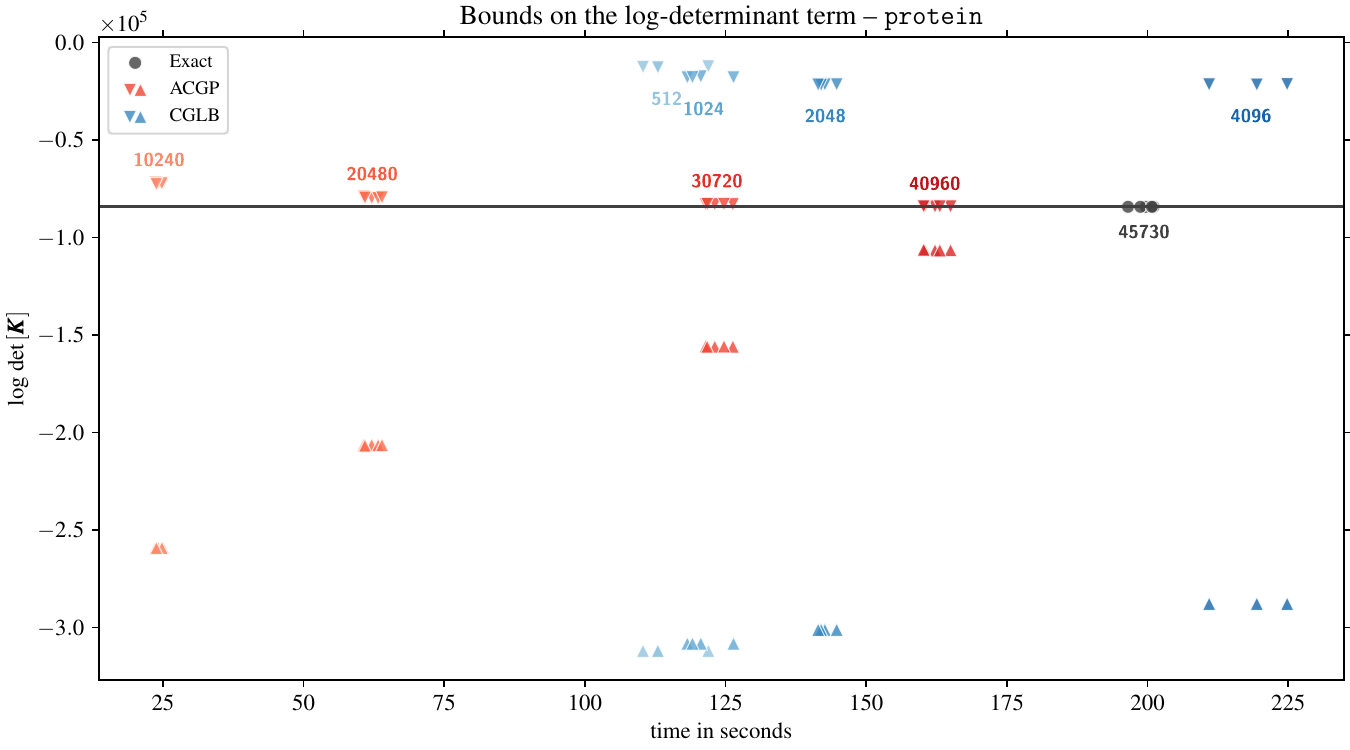}
		\subcaption{OU kernel, $\log\ell = 0$}
		\label{subfig:protein_ou_loget_0}
	\end{minipage}
	\begin{minipage}[b]{.5\textwidth}
		\centering
		\includegraphics[width=0.96\textwidth]{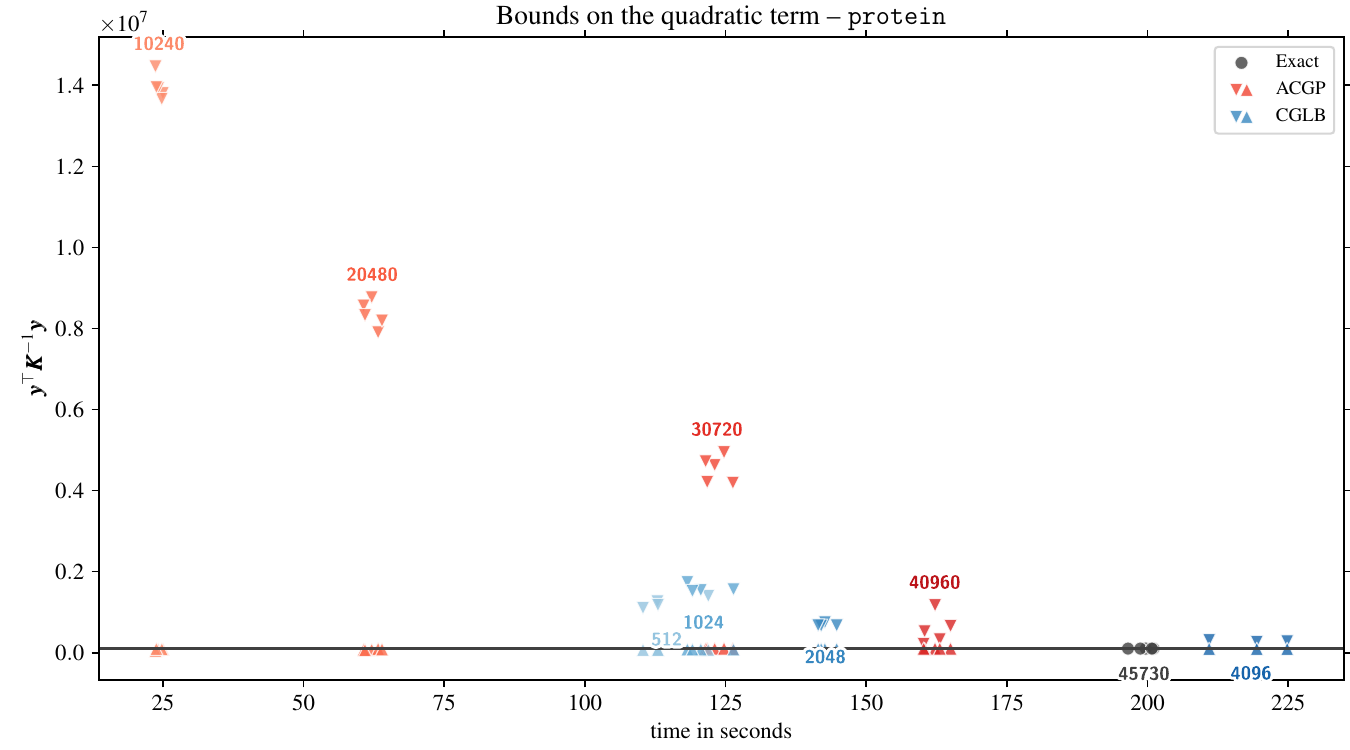}
		\subcaption{OU kernel, $\log\ell = 0$}
		\label{subfig:protein_ou_quadratic_0}
	\end{minipage}

	\begin{minipage}[b]{.5\textwidth}
		\centering
		\includegraphics[width=0.96\textwidth]{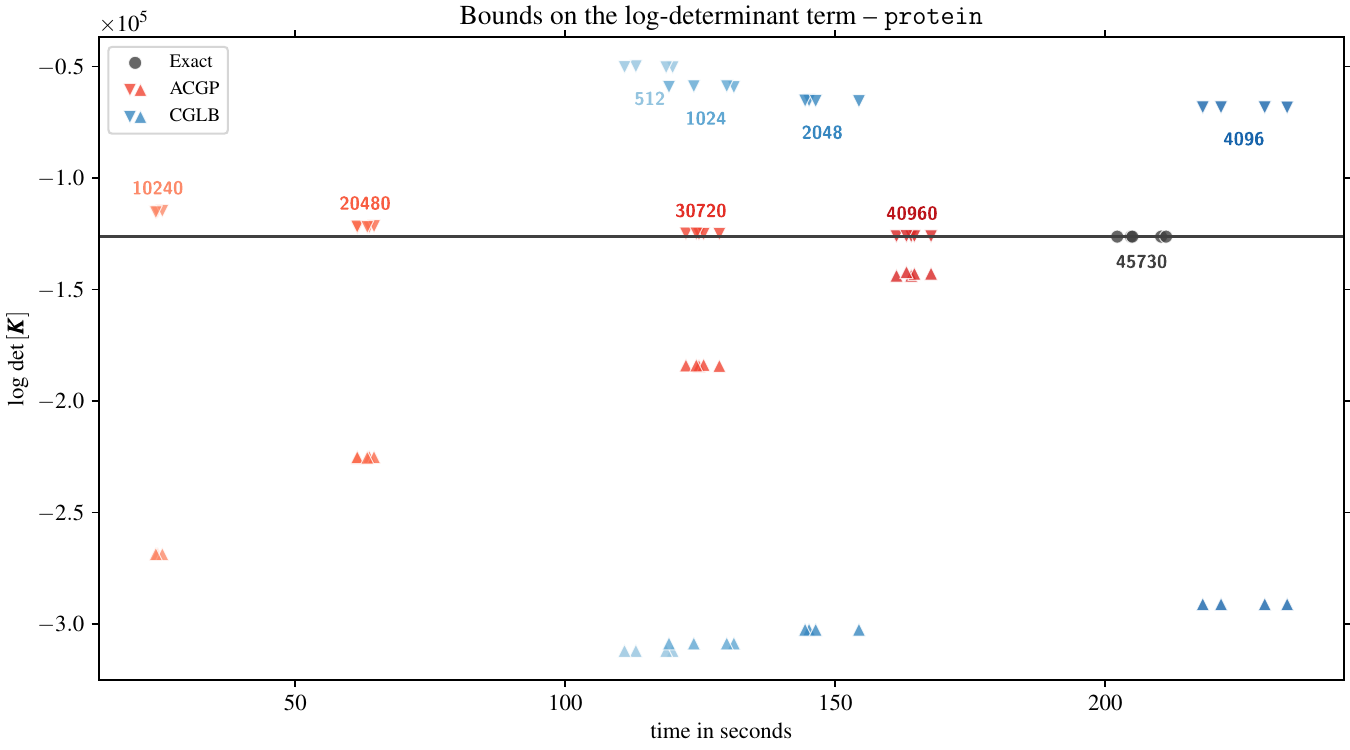}
		\subcaption{OU kernel, $\log\ell = 1$}
		\label{subfig:protein_ou_loget_1}
	\end{minipage}
	\begin{minipage}[b]{.5\textwidth}
		\centering
		\includegraphics[width=0.96\textwidth]{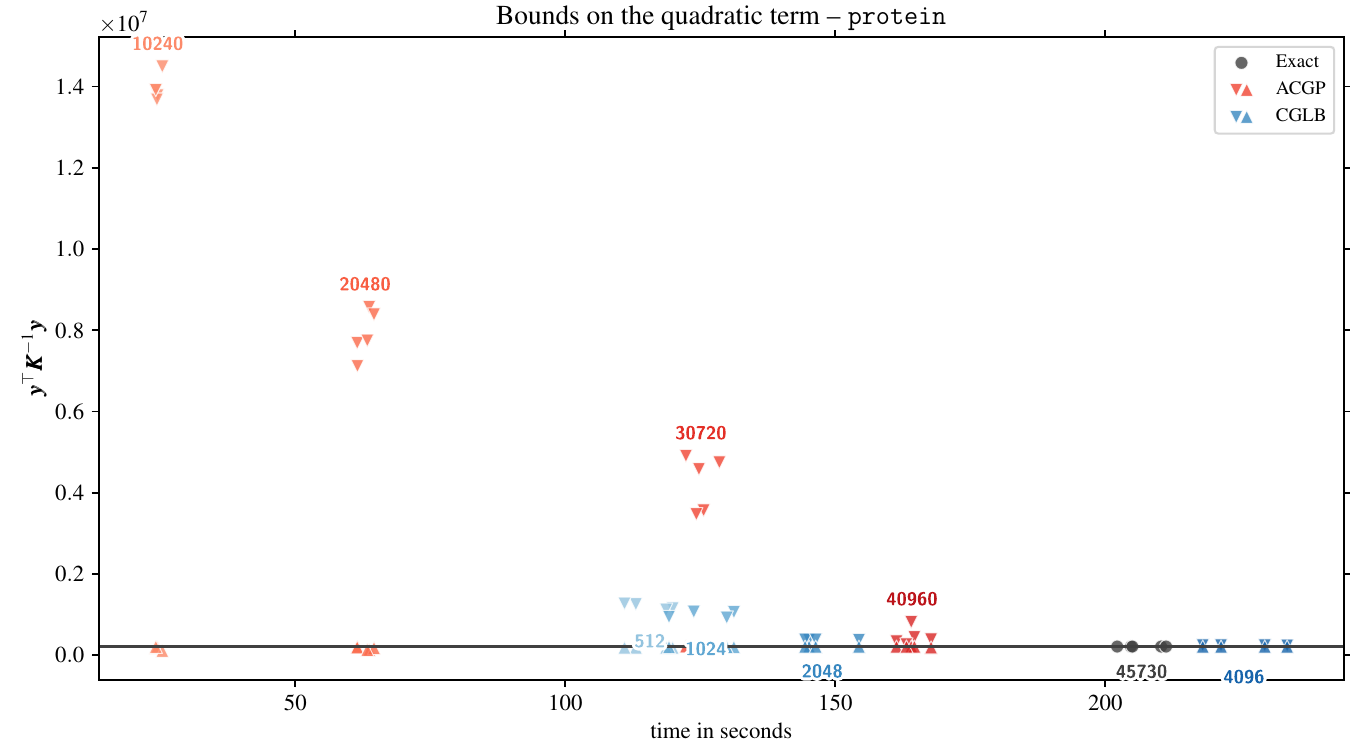}
		\subcaption{OU kernel, $\log\ell = 1$}
		\label{subfig:protein_ou_quadratic_1}
	\end{minipage}

	\begin{minipage}[b]{.5\textwidth}
		\centering
		\includegraphics[width=0.96\textwidth]{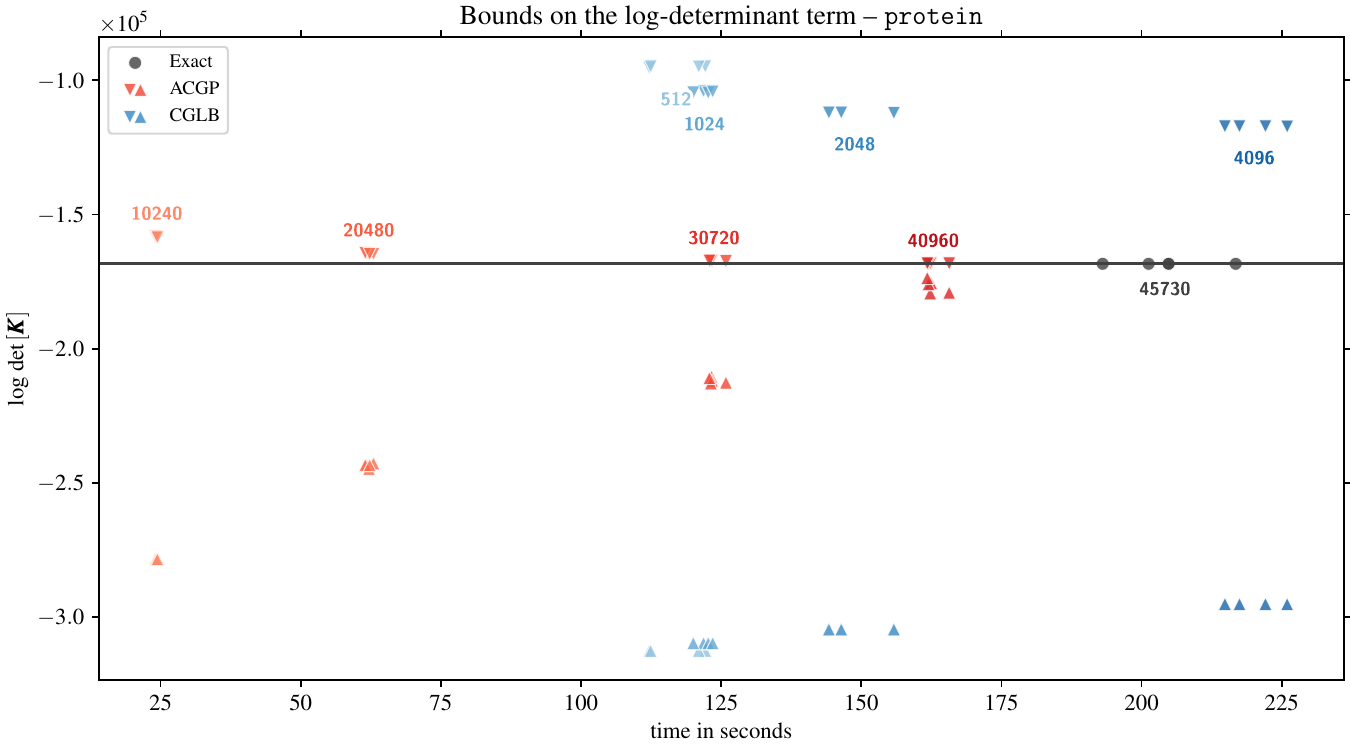}
		\subcaption{OU kernel, $\log\ell = 2$}
		\label{subfig:protein_ou_loget_2}
	\end{minipage}
	\begin{minipage}[b]{.5\textwidth}
		\centering
		\includegraphics[width=0.96\textwidth]{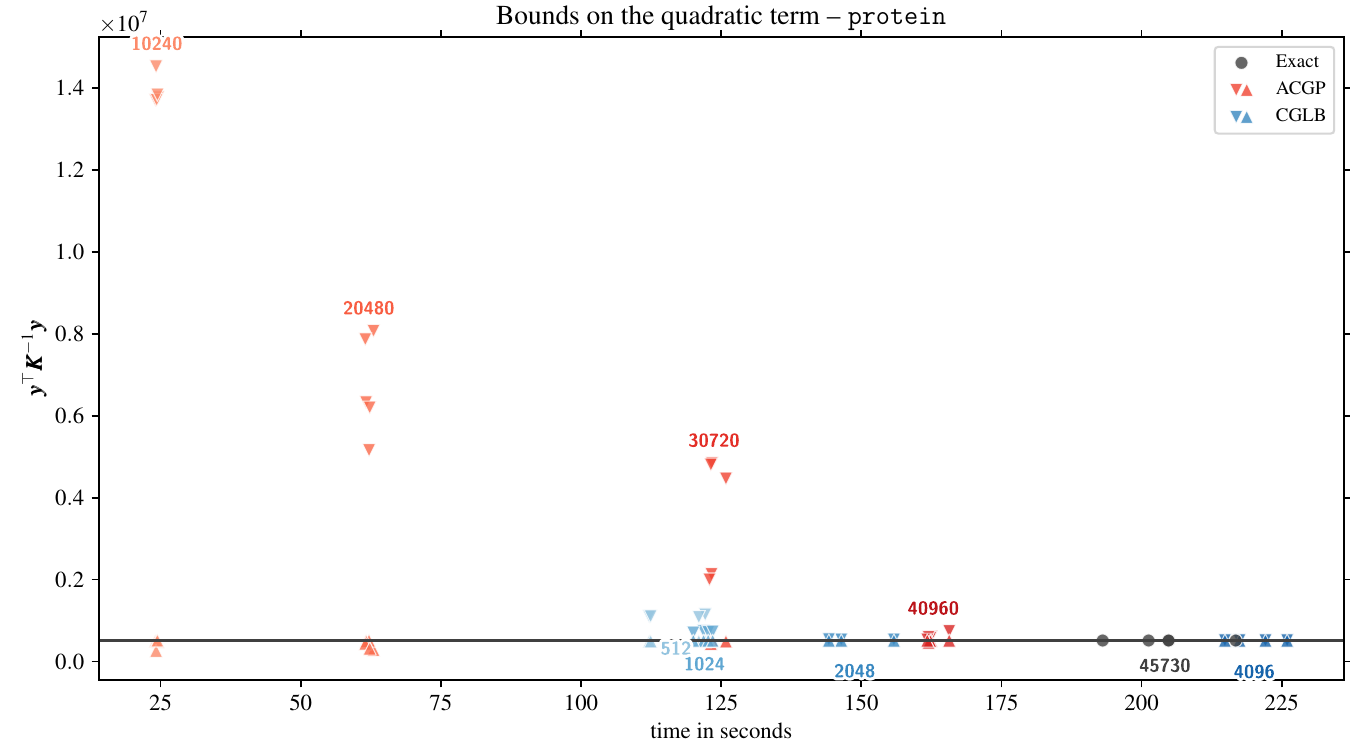}
		\subcaption{OU kernel, $\log\ell = 2$}
		\label{subfig:protein_ou_quadratic_2}
	\end{minipage}
    \caption{Upper and lower bounds on the log-determinant term (left column) and the quadratic term (right column) for the \texttt{protein} dataset using an Ornstein-Uhlenbeck (OU) kernel.}
	\label{fig:bounds_protein_ou}
\end{figure}

\clearpage
\subsubsection{Bounds for experiments on \texttt{kin40k}}
\label{subsec:bounds_kin40k}
\begin{figure}[htb!]
	\begin{minipage}[b]{.5\textwidth}
		\centering
		\includegraphics[width=0.96\textwidth]{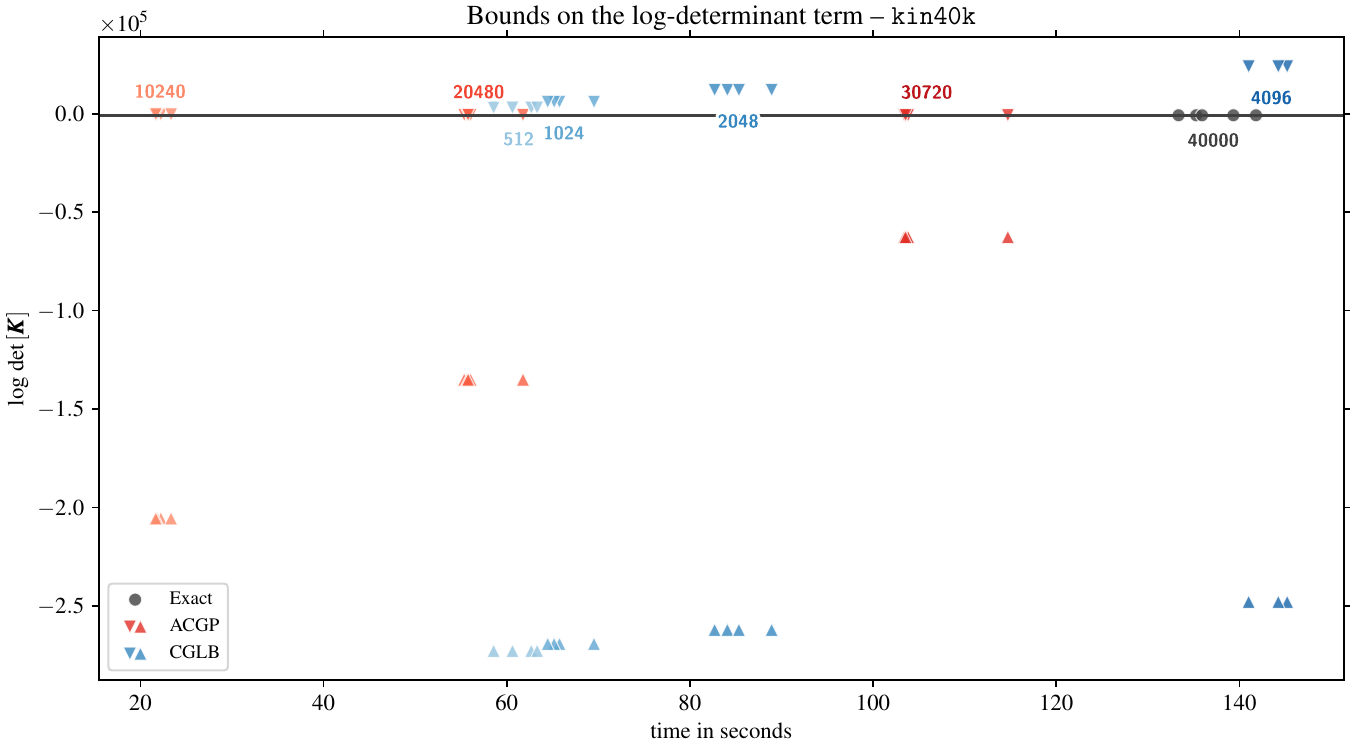}
		\subcaption{SE kernel, $\log\ell = -1$}
		\label{subfig:kin40k_rbf_loget_-1}
	\end{minipage}
	\begin{minipage}[b]{.5\textwidth}
		\centering
		\includegraphics[width=0.96\textwidth]{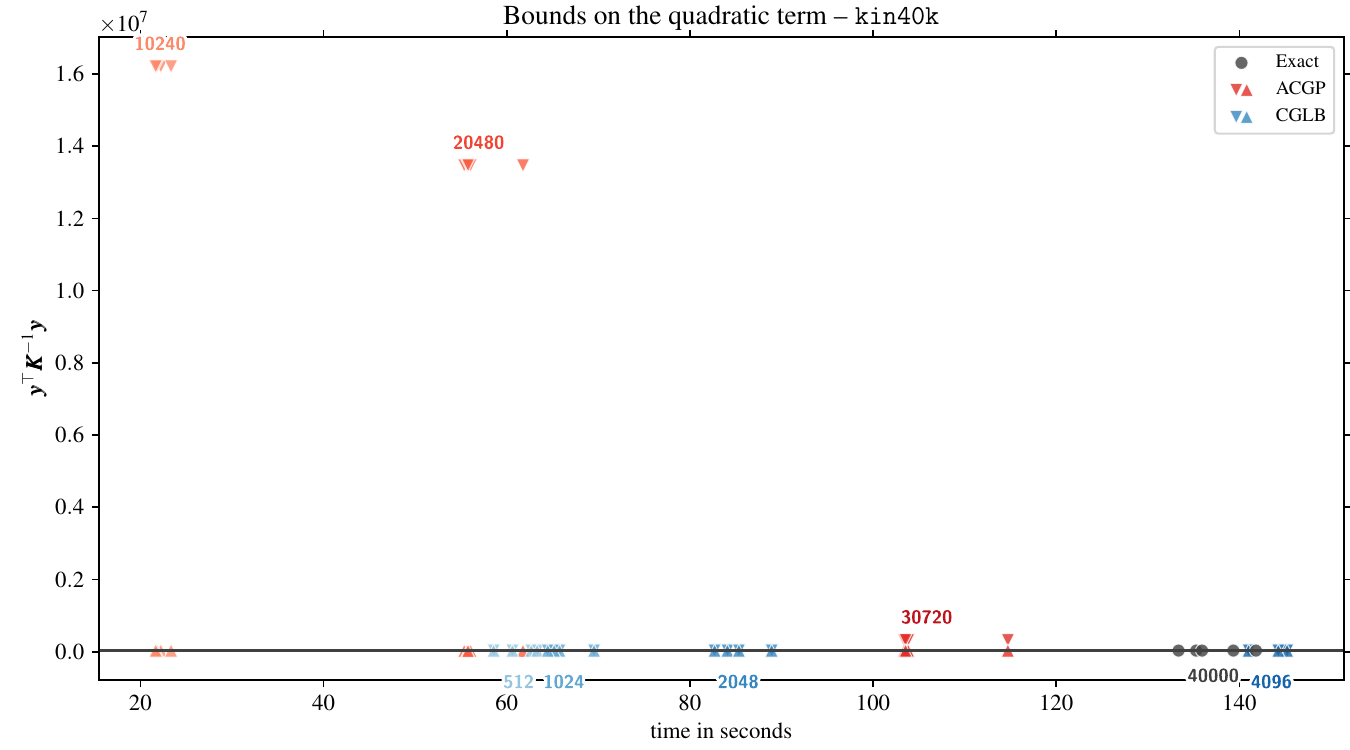}
		\subcaption{SE kernel, $\log\ell = -1$}
		\label{subfig:kin40k_rbf_quadratic_-1}
	\end{minipage}

	\begin{minipage}[b]{.5\textwidth}
		\centering
		\includegraphics[width=0.96\textwidth]{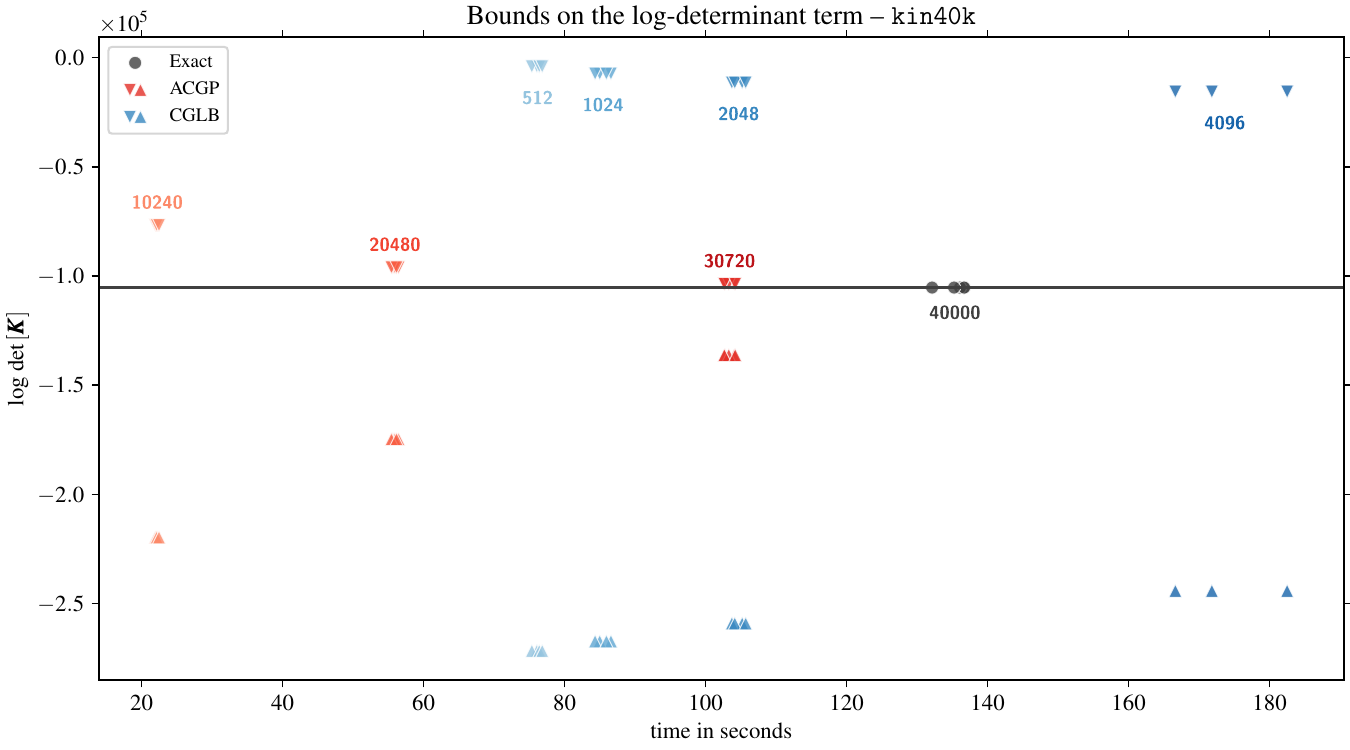}
		\subcaption{SE kernel, $\log\ell = 0$}
		\label{subfig:kin40k_rbf_loget_0}
	\end{minipage}
	\begin{minipage}[b]{.5\textwidth}
		\centering
		\includegraphics[width=0.96\textwidth]{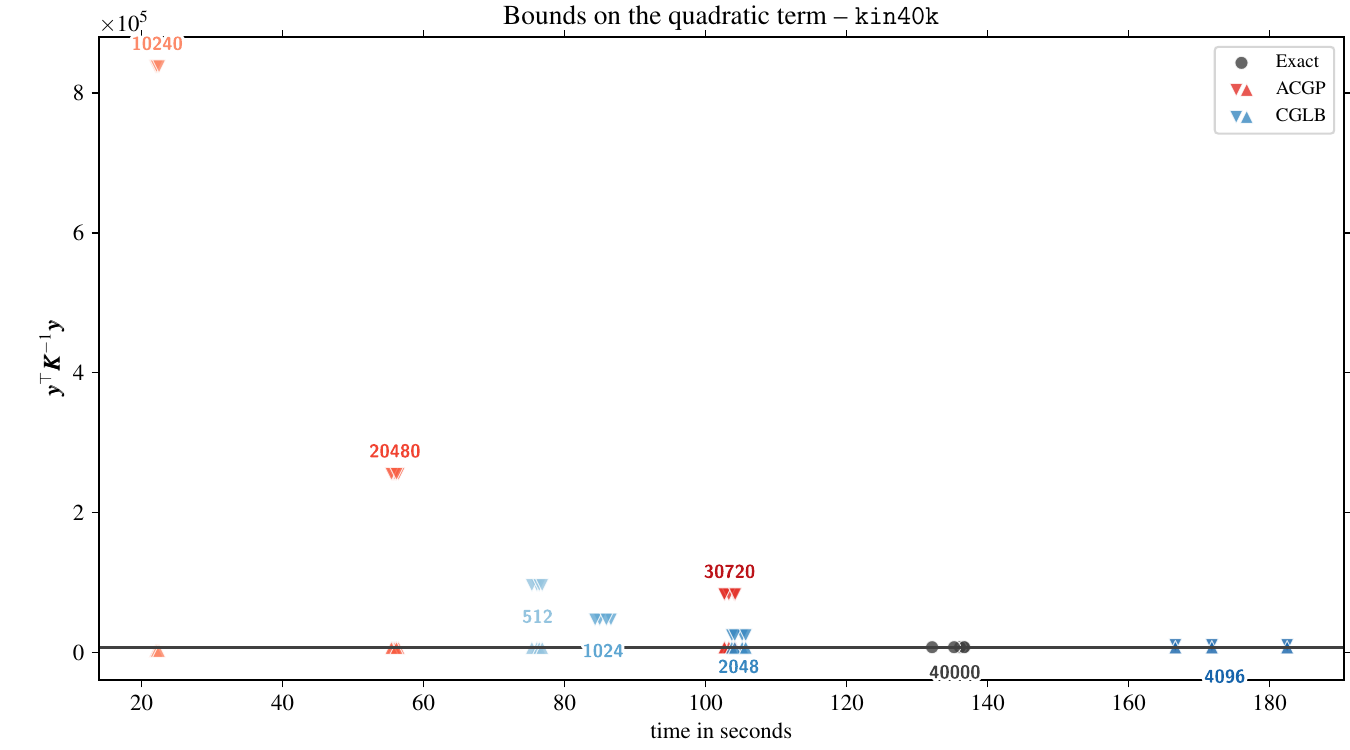}
		\subcaption{SE kernel, $\log\ell = 0$}
		\label{subfig:kin40k_rbf_quadratic_0}
	\end{minipage}

	\begin{minipage}[b]{.5\textwidth}
		\centering
		\includegraphics[width=0.96\textwidth]{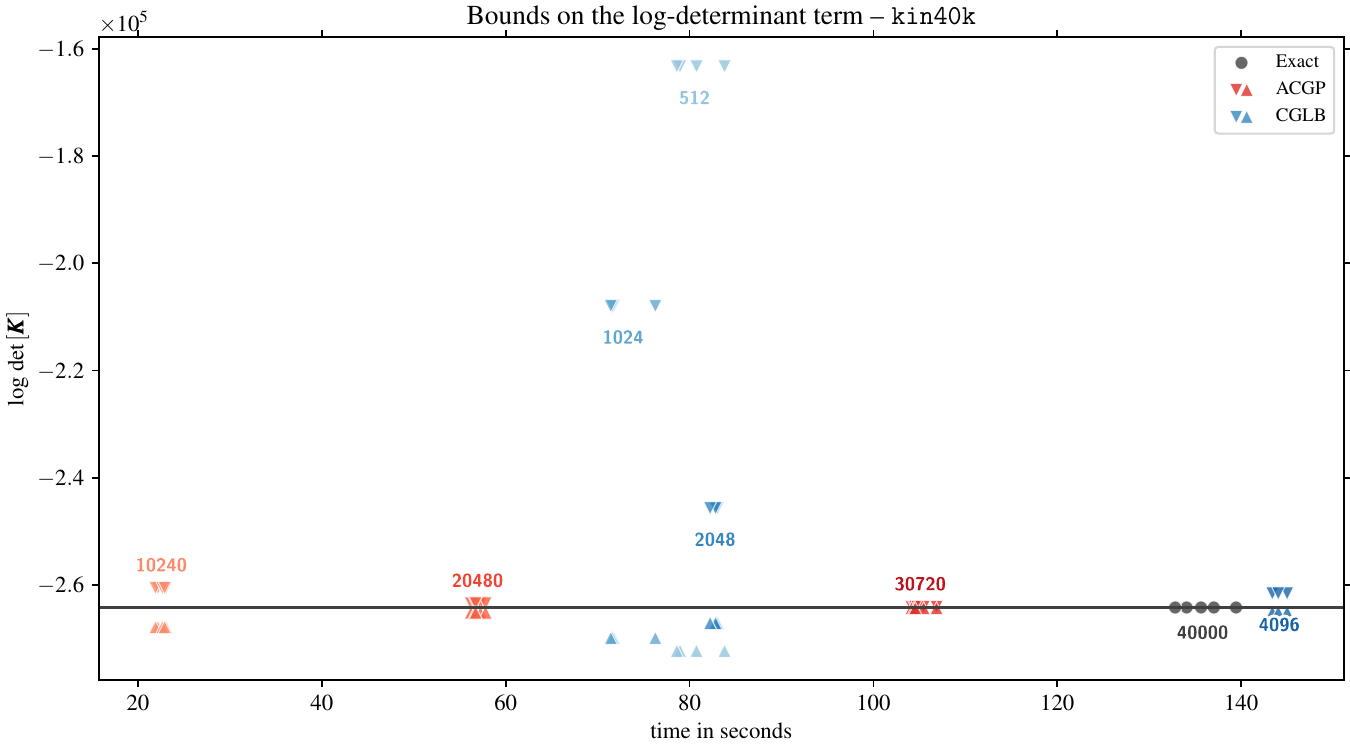}
		\subcaption{SE kernel, $\log\ell = 1$}
		\label{subfig:kin40k_rbf_loget_1}
	\end{minipage}
	\begin{minipage}[b]{.5\textwidth}
		\centering
		\includegraphics[width=0.96\textwidth]{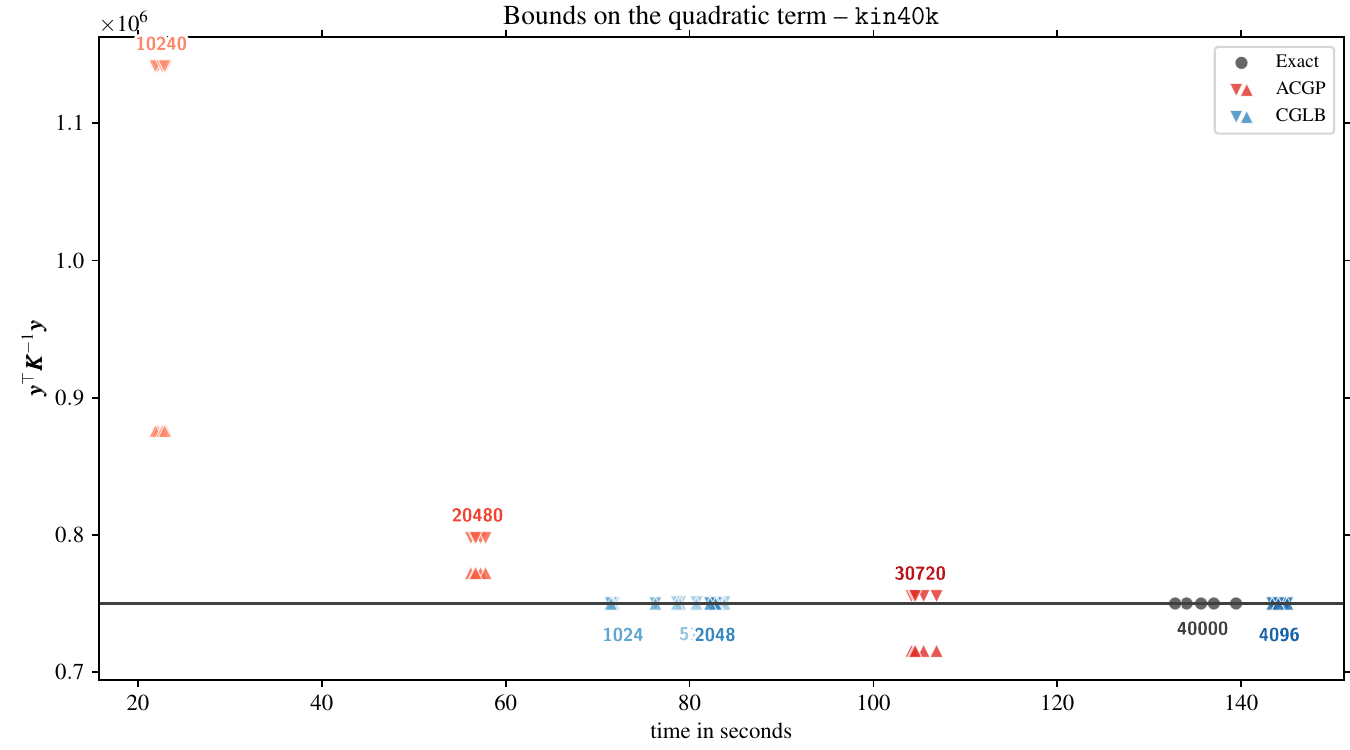}
		\subcaption{SE kernel, $\log\ell = 1$}
		\label{subfig:kin40k_rbf_quadratic_1}
	\end{minipage}

	\begin{minipage}[b]{.5\textwidth}
		\centering
		\includegraphics[width=0.96\textwidth]{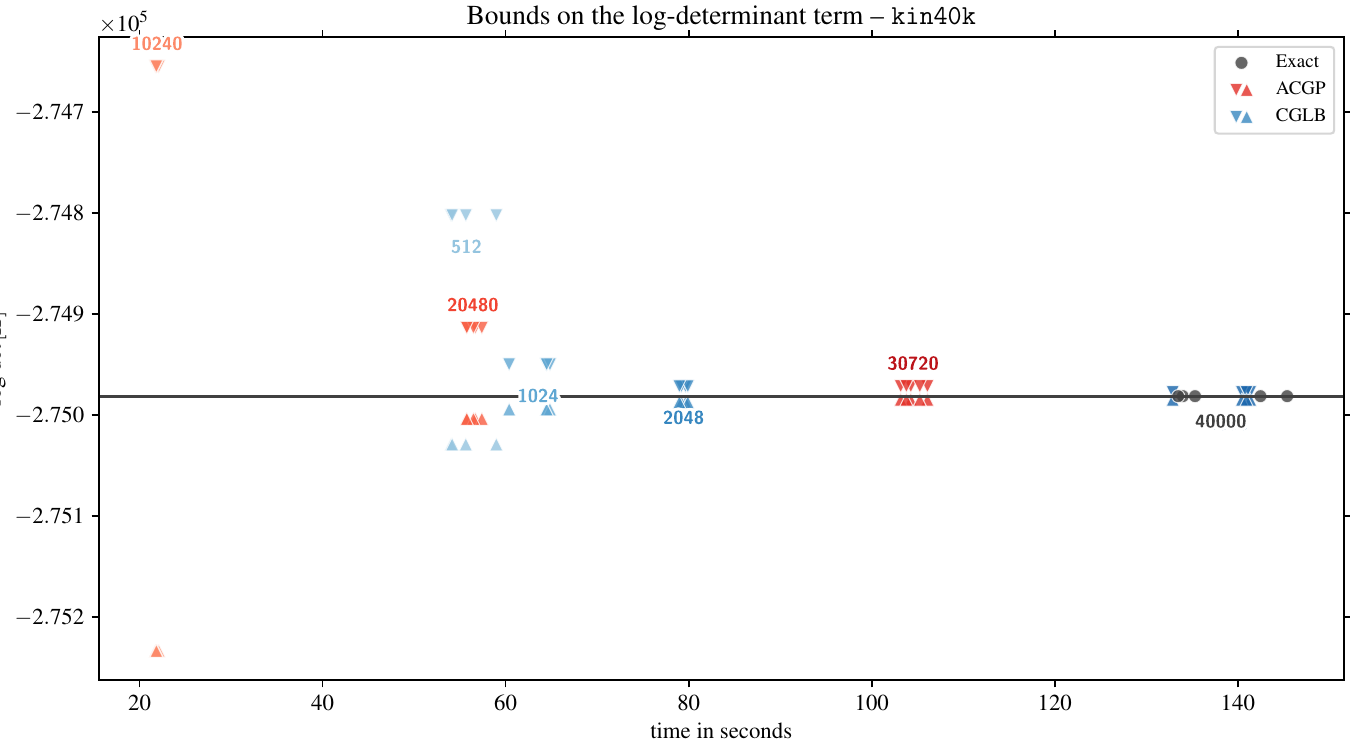}
		\subcaption{SE kernel, $\log\ell = 2$}
		\label{subfig:kin40k_rbf_loget_2}
	\end{minipage}
	\begin{minipage}[b]{.5\textwidth}
		\centering
		\includegraphics[width=0.96\textwidth]{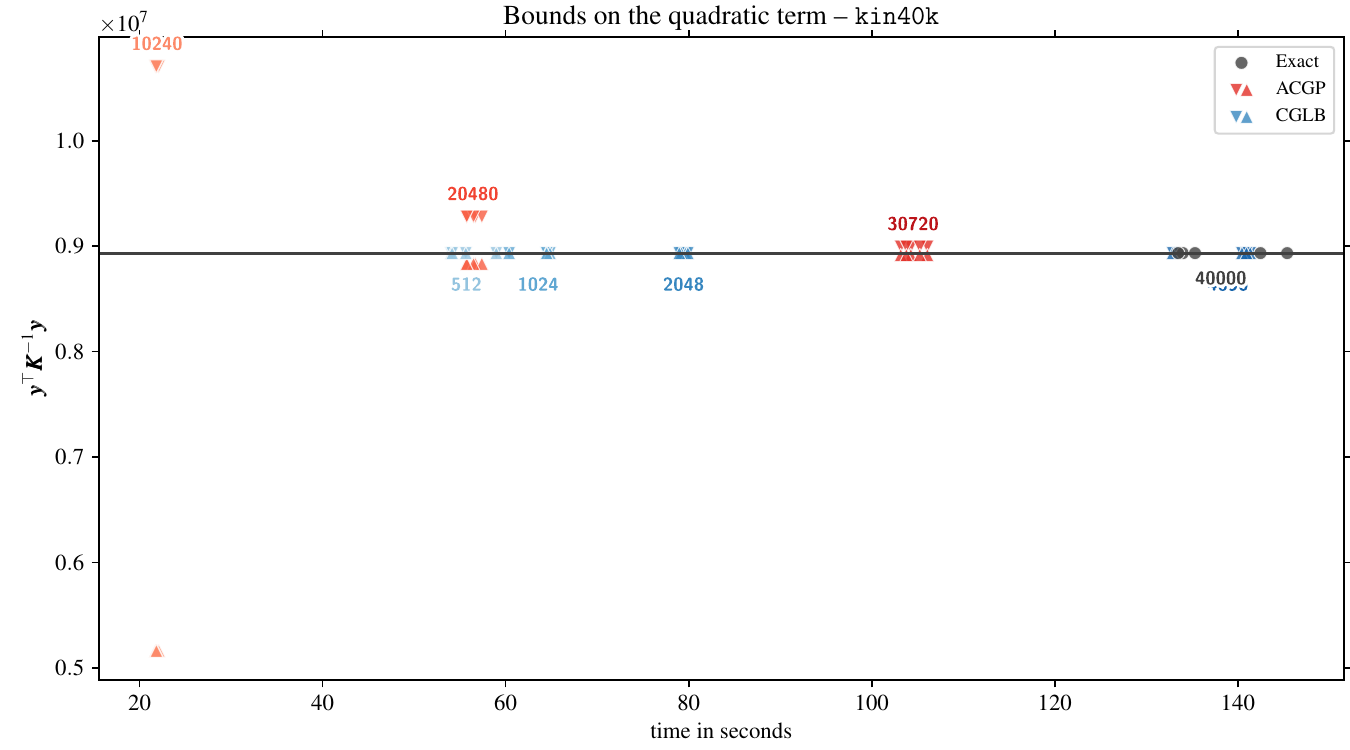}
		\subcaption{SE kernel, $\log\ell = 2$}
		\label{subfig:kin40k_rbf_quadratic_2}
	\end{minipage}
	\caption{Upper and lower bounds on the log-determinant term (left column) and the quadratic term (right column) for the \texttt{kin40k} dataset.}
	\label{fig:bounds__kin40k_rbf}
\end{figure}

\begin{figure}[htb]
	\begin{minipage}[b]{.5\textwidth}
		\centering
		\includegraphics[width=0.96\textwidth]{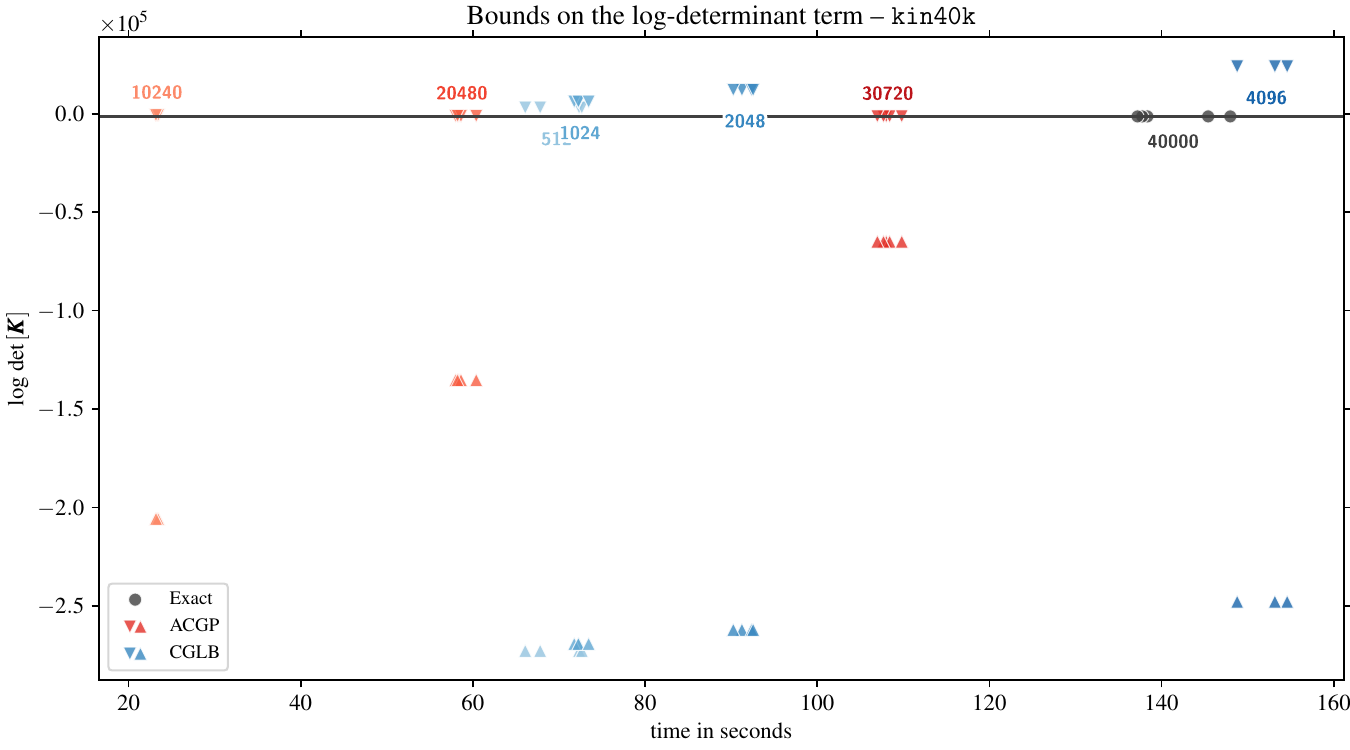}
		\subcaption{OU kernel, $\log\ell = -1$}
		\label{subfig:kin40k_ou_loget_-1}
	\end{minipage}
	\begin{minipage}[b]{.5\textwidth}
		\centering
		\includegraphics[width=0.96\textwidth]{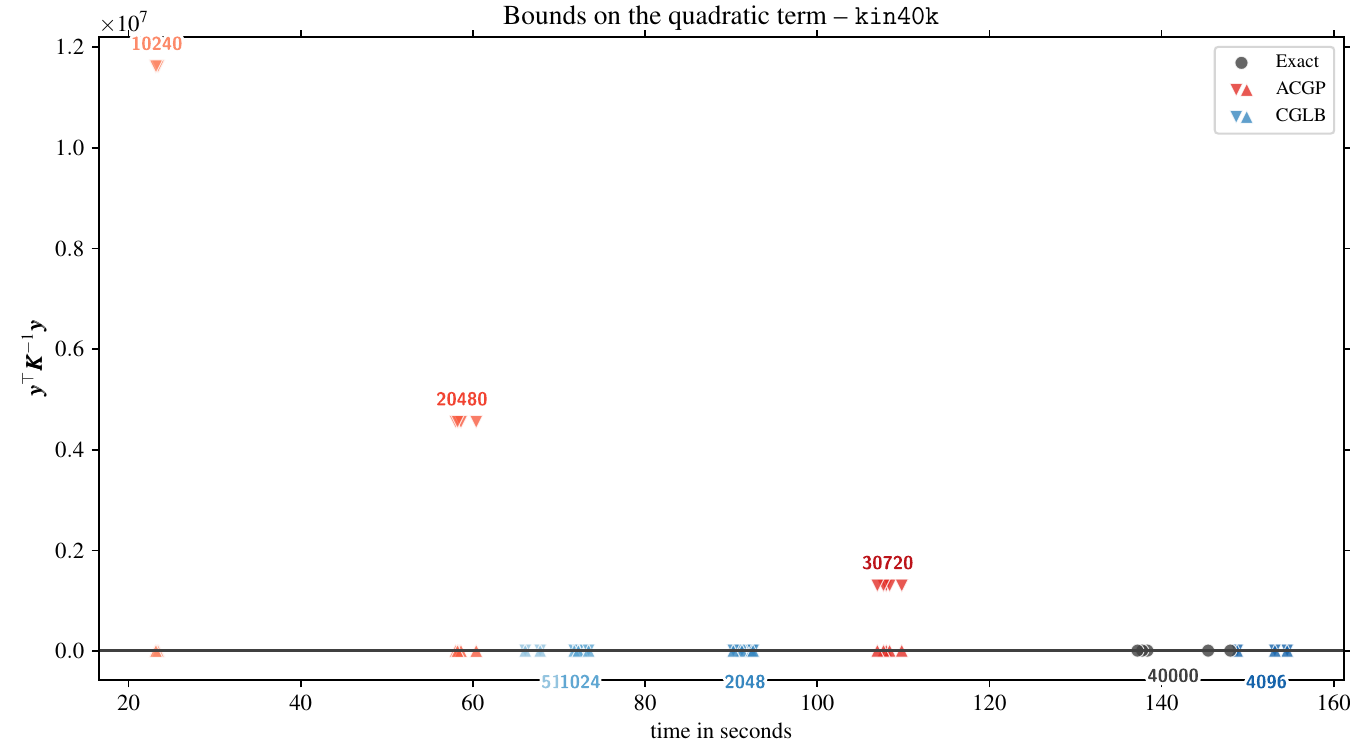}
		\subcaption{OU kernel, $\log\ell = -1$}
		\label{subfig:kin40k_ou_quadratic_-1}
	\end{minipage}

	\begin{minipage}[b]{.5\textwidth}
		\centering
		\includegraphics[width=0.96\textwidth]{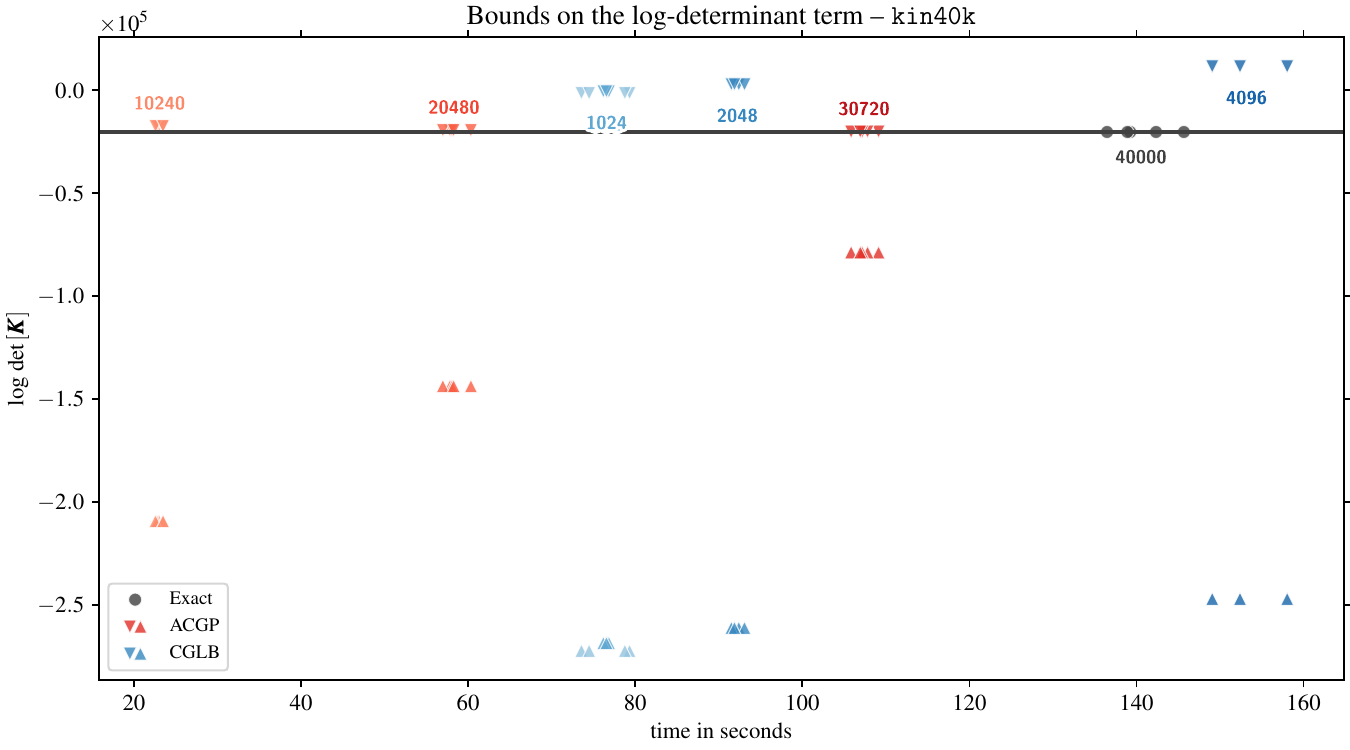}
		\subcaption{OU kernel, $\log\ell = 0$}
		\label{subfig:kin40k_ou_loget_0}
	\end{minipage}
	\begin{minipage}[b]{.5\textwidth}
		\centering
		\includegraphics[width=0.96\textwidth]{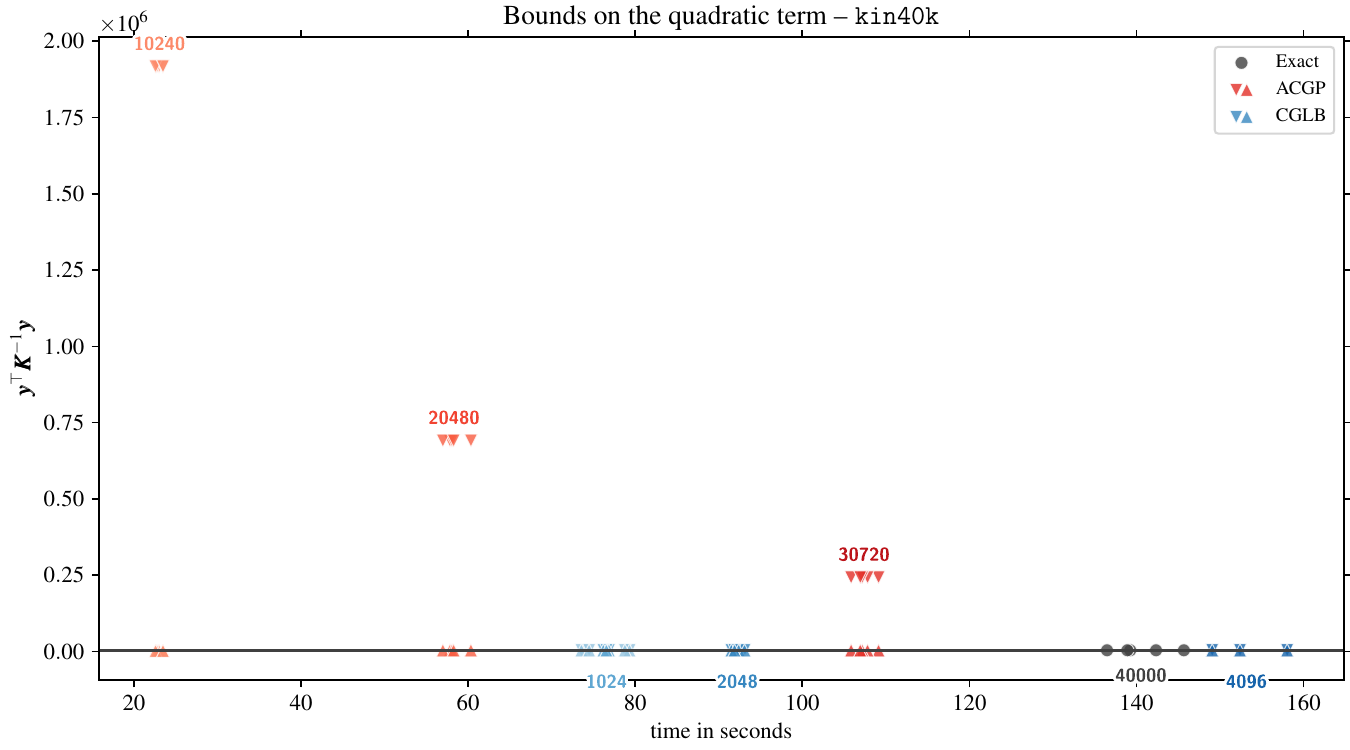}
		\subcaption{OU kernel, $\log\ell = 0$}
		\label{subfig:kin40k_ou_quadratic_0}
	\end{minipage}

	\begin{minipage}[b]{.5\textwidth}
		\centering
		\includegraphics[width=0.96\textwidth]{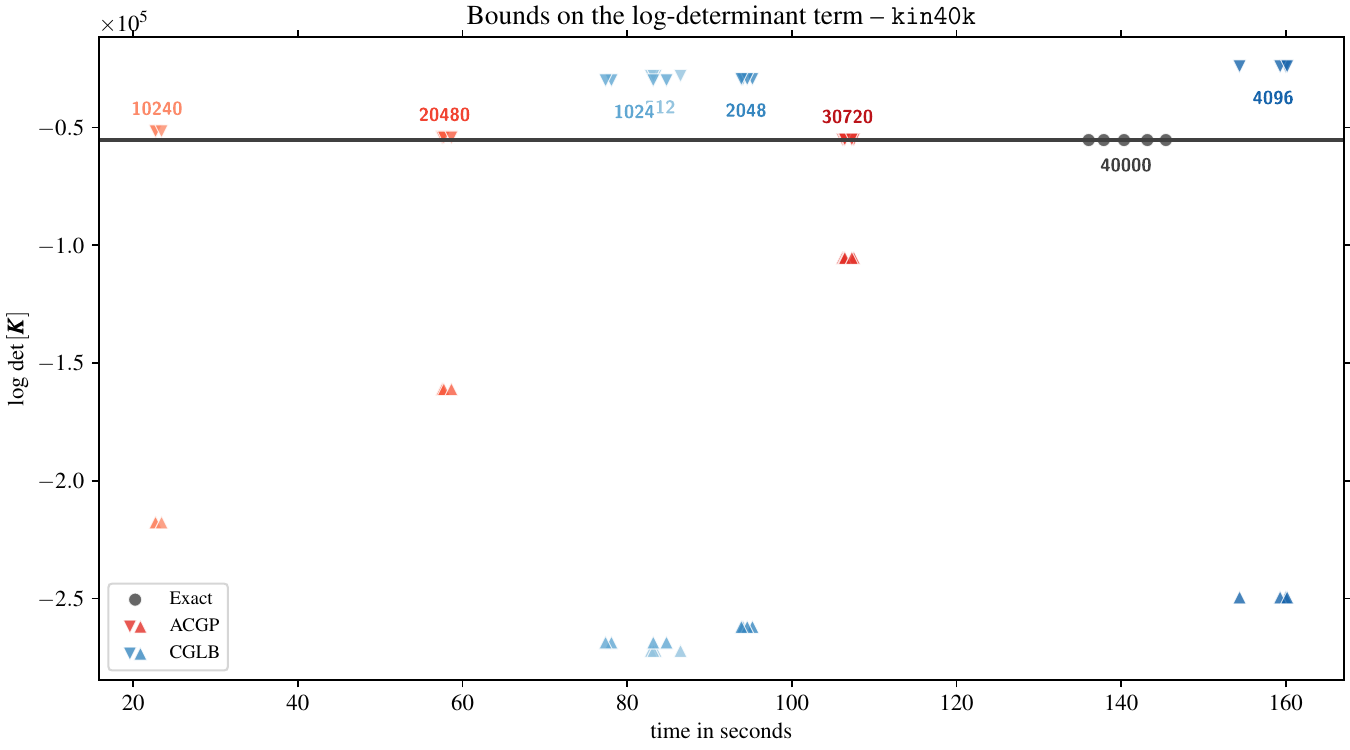}
		\subcaption{OU kernel, $\log\ell = 1$}
		\label{subfig:kin40k_ou_loget_1}
	\end{minipage}
	\begin{minipage}[b]{.5\textwidth}
		\centering
		\includegraphics[width=0.96\textwidth]{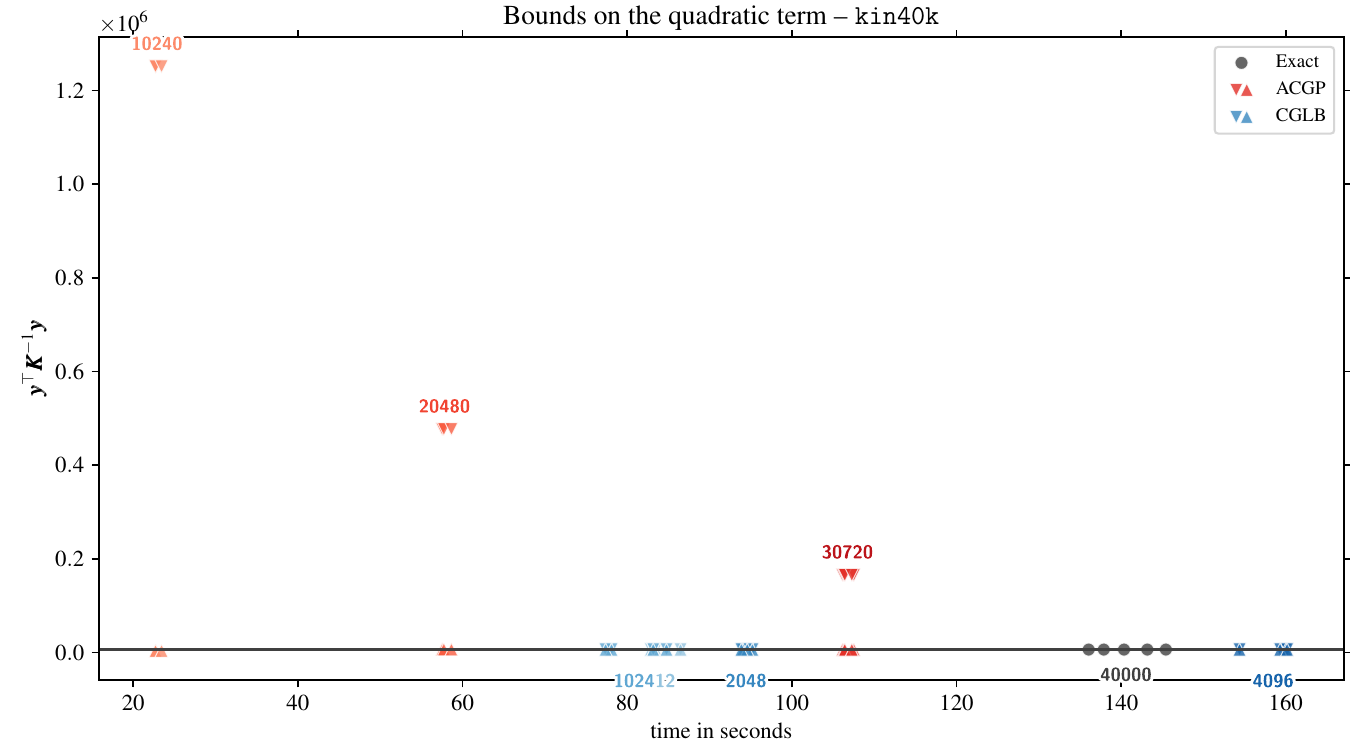}
		\subcaption{OU kernel, $\log\ell = 1$}
		\label{subfig:kin40k_ou_quadratic_1}
	\end{minipage}

	\begin{minipage}[b]{.5\textwidth}
		\centering
		\includegraphics[width=0.96\textwidth]{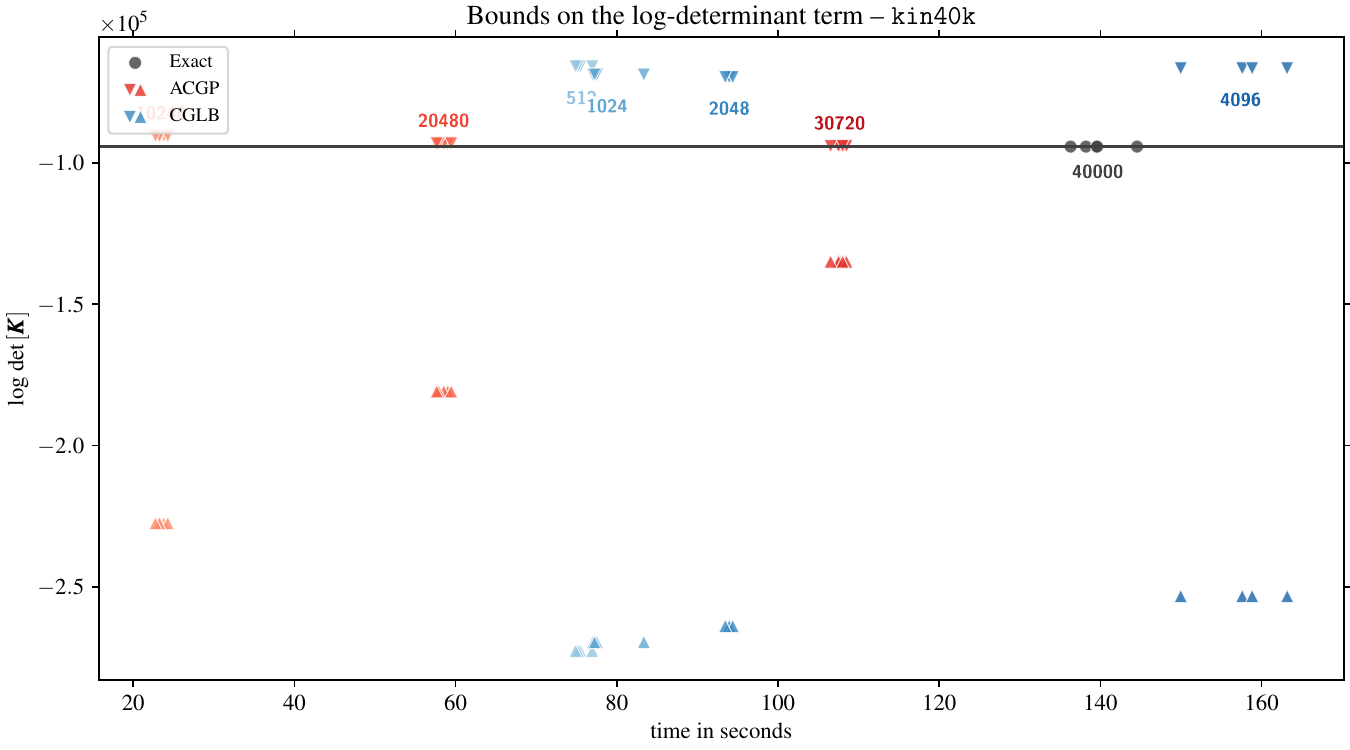}
		\subcaption{OU kernel, $\log\ell = 2$}
		\label{subfig:kin40k_ou_loget_2}
	\end{minipage}
	\begin{minipage}[b]{.5\textwidth}
		\centering
		\includegraphics[width=0.96\textwidth]{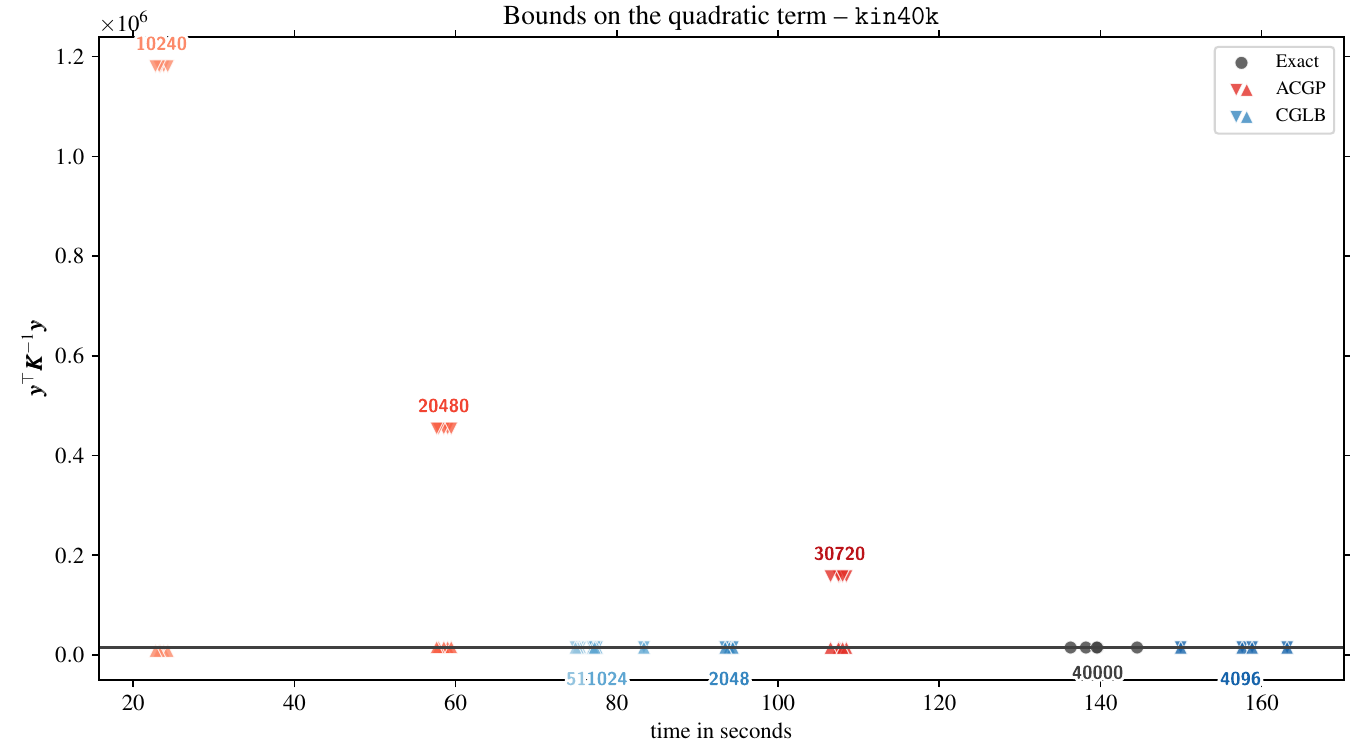}
		\subcaption{OU kernel, $\log\ell = 2$}
		\label{subfig:kin40k_ou_quadratic_2}
	\end{minipage}
	\caption{Upper and lower bounds on the log-determinant term (left column) and the quadratic term (right column) for the \texttt{kin40k} dataset using an Ornstein-Uhlenbeck (OU) kernel.}
	\label{fig:bounds_kin40k_ou}
\end{figure}

\clearpage
\subsection{Aggregated plots for the bound quality experiments}
\label{subsec:llh_bounds}
\subsubsection{Bounds for experiments on \texttt{metro}}
\label{subsec:llh_bounds_metro}
\begin{figure}[htb!]
	\begin{minipage}[b]{.5\textwidth}
		\centering
		\includegraphics[width=0.96\textwidth]{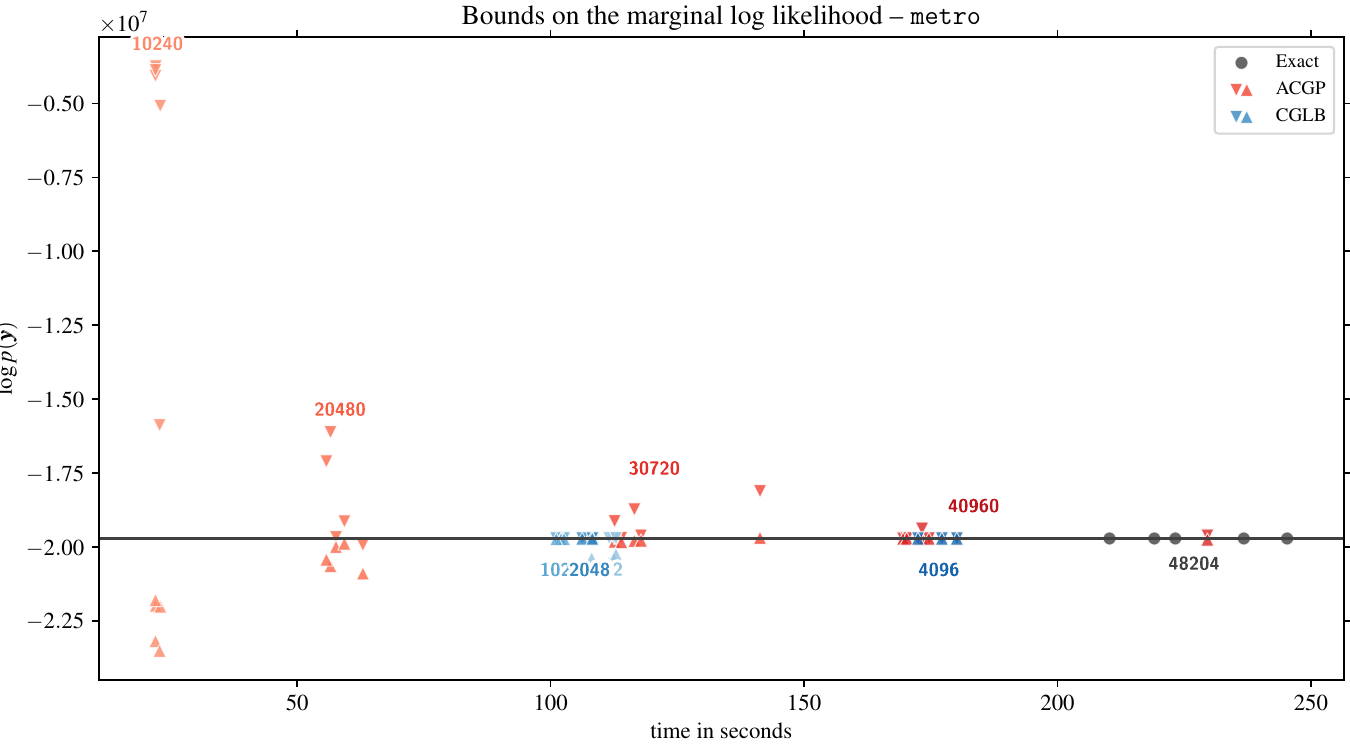}
		\subcaption{SE kernel, $\log\ell = -1$}
		\label{subfig:metro_rbf_llh_-1}
	\end{minipage}
	\begin{minipage}[b]{.5\textwidth}
		\centering
		\includegraphics[width=0.96\textwidth]{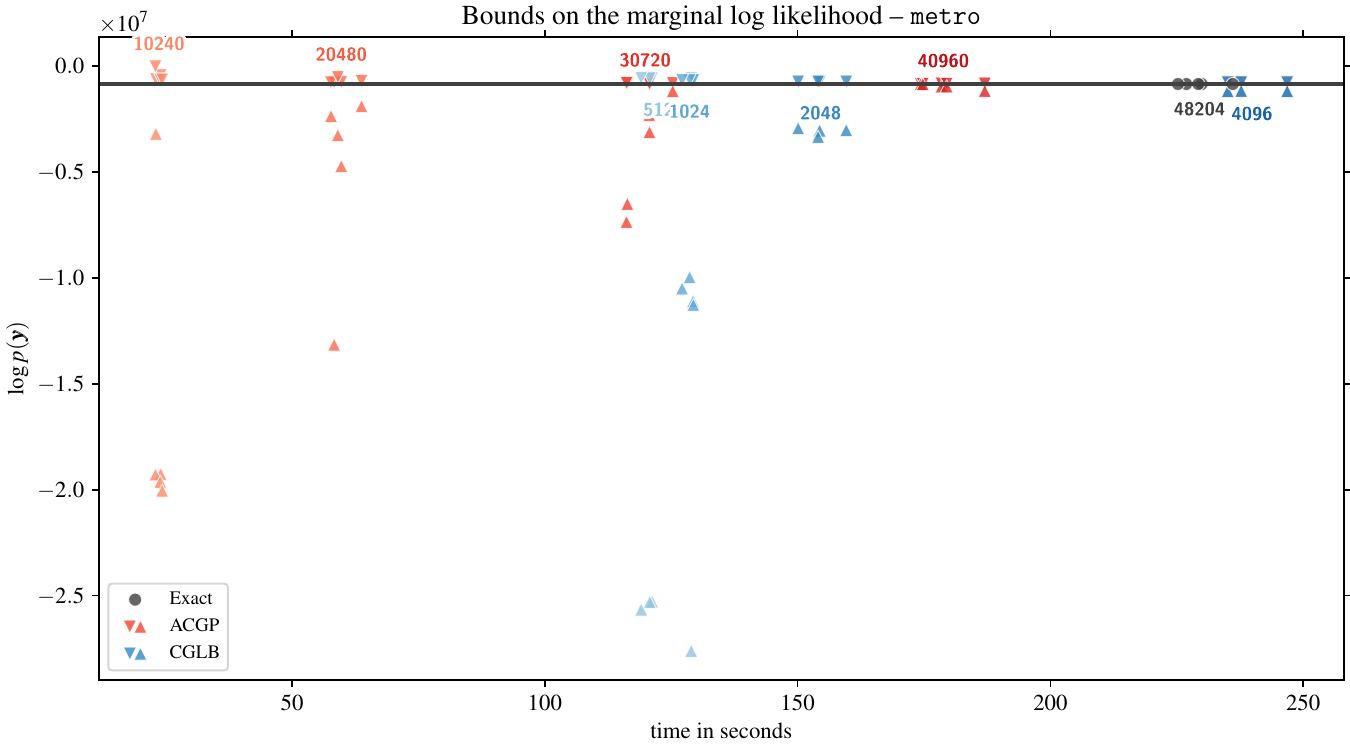}
		\subcaption{OU kernel, $\log\ell = -1$}
		\label{subfig:metro_ou_llh_-1}
	\end{minipage}
	\begin{minipage}[b]{.5\textwidth}
		\centering
		\includegraphics[width=0.96\textwidth]{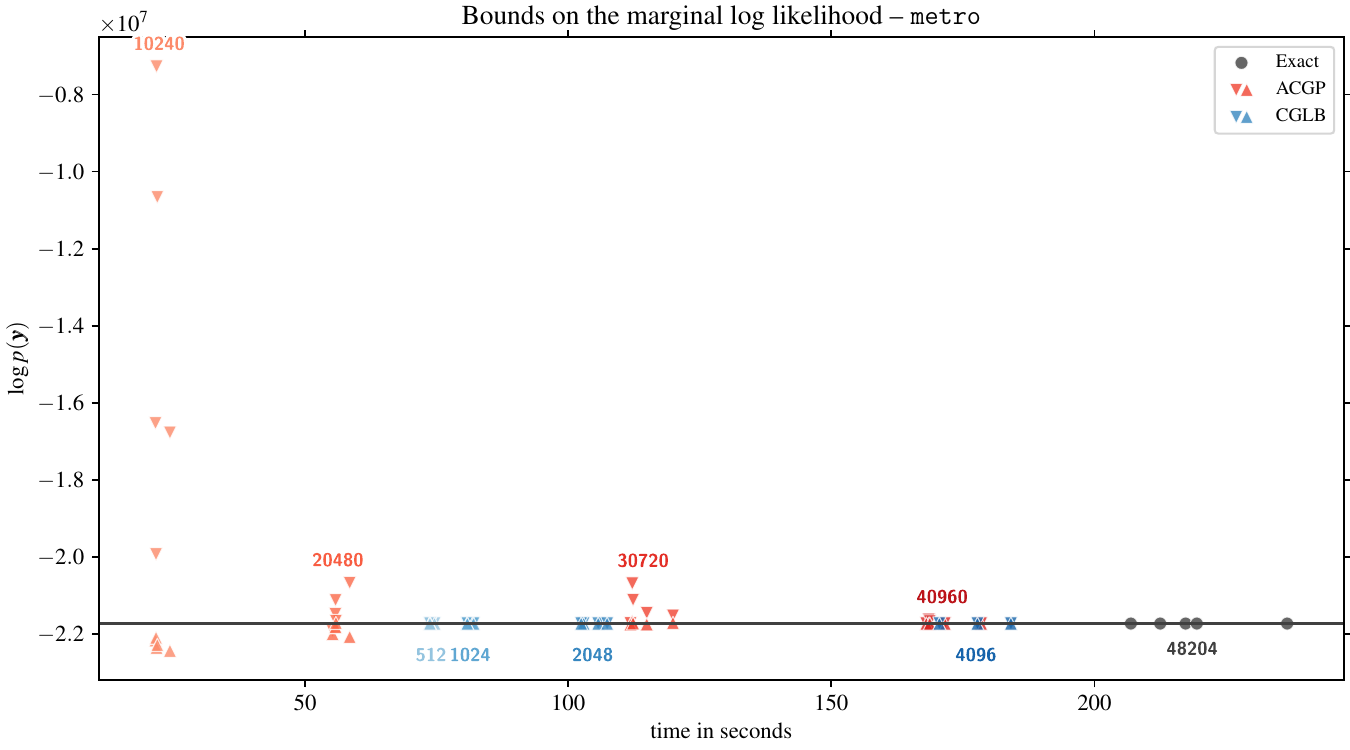}
		\subcaption{SE kernel, $\log\ell = 0$}
		\label{subfig:metro_rbf_llh_0}
	\end{minipage}
	\begin{minipage}[b]{.5\textwidth}
		\centering
		\includegraphics[width=0.96\textwidth]{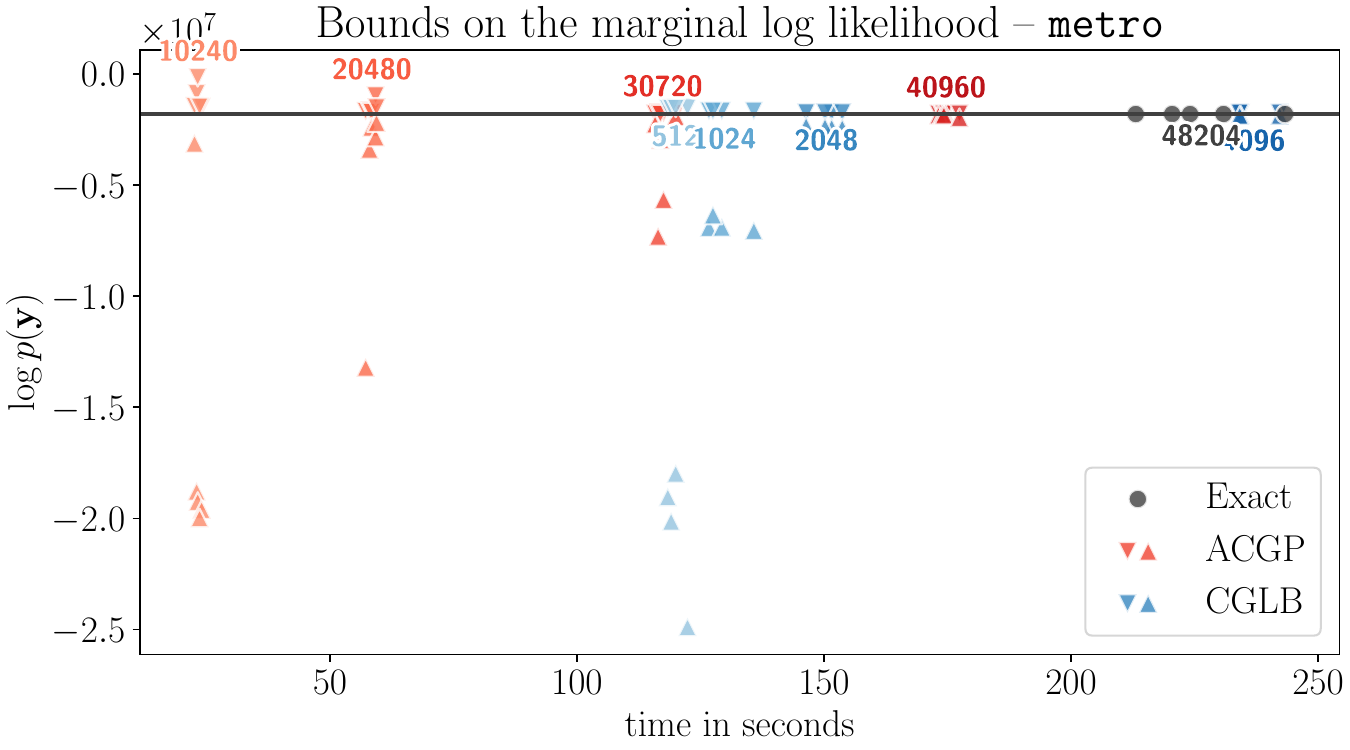}
		\subcaption{OU kernel, $\log\ell = 0$}
		\label{subfig:metro_ou_llh_0}
	\end{minipage}
	\begin{minipage}[b]{.5\textwidth}
		\centering
		\includegraphics[width=0.96\textwidth]{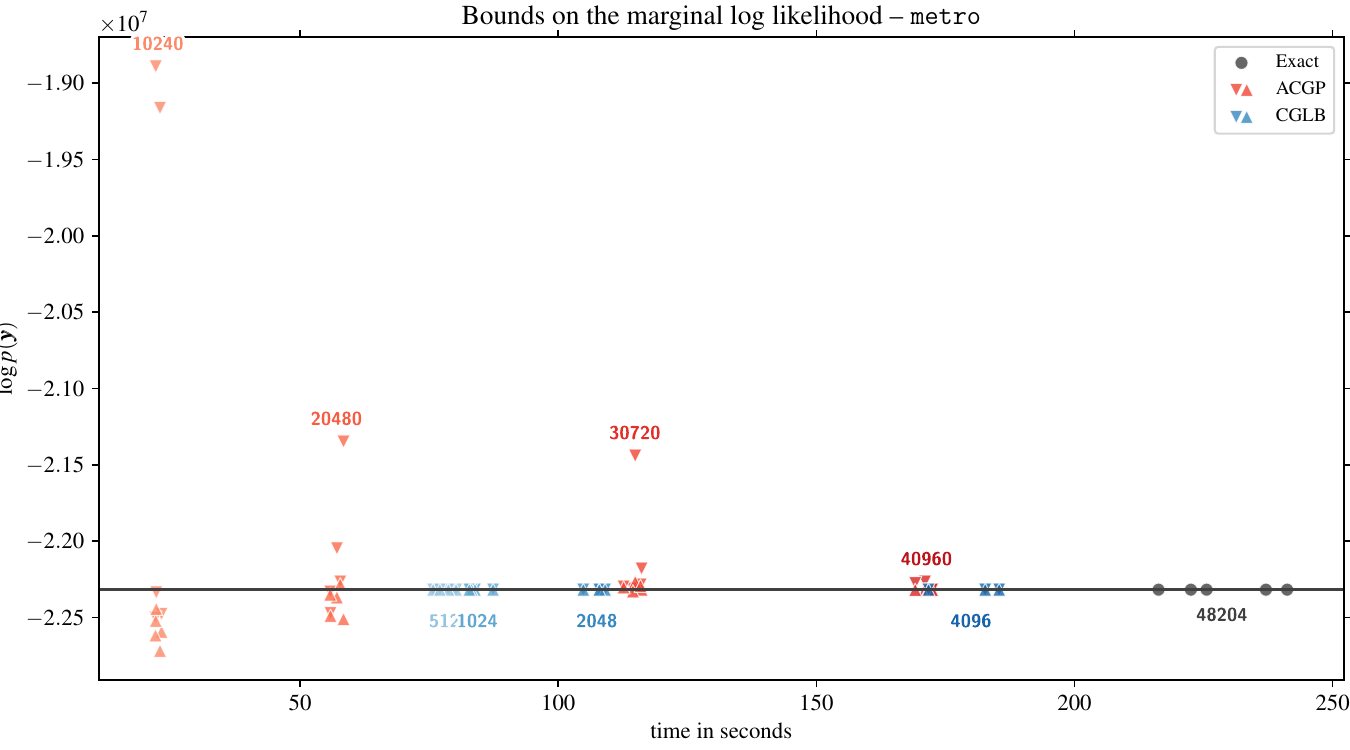}
		\subcaption{SE kernel, $\log\ell = 1$}
		\label{subfig:metro_rbf_llh_1}
	\end{minipage}
	\begin{minipage}[b]{.5\textwidth}
		\centering
		\includegraphics[width=0.96\textwidth]{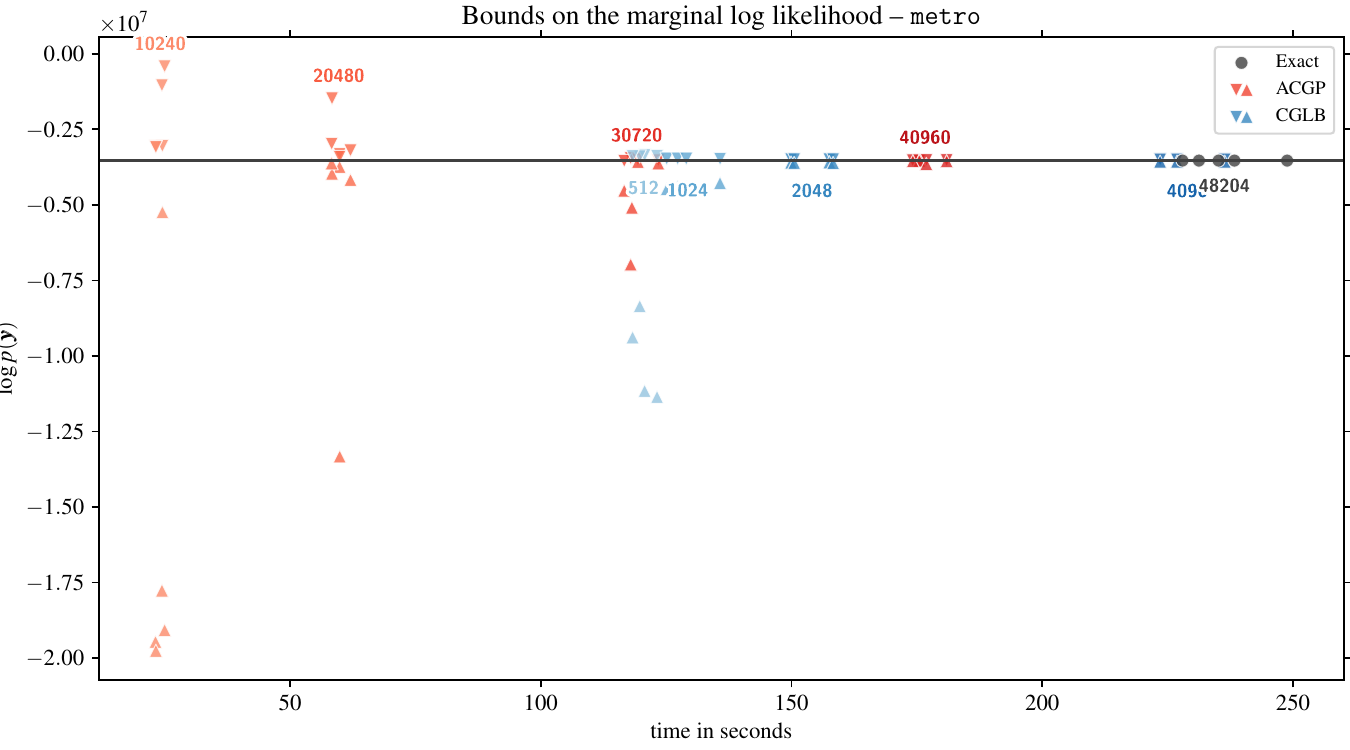}
		\subcaption{OU kernel, $\log\ell = 1$}
		\label{subfig:metro_ou_llh_1}
	\end{minipage}
	\begin{minipage}[b]{.5\textwidth}
		\centering
		\includegraphics[width=0.96\textwidth]{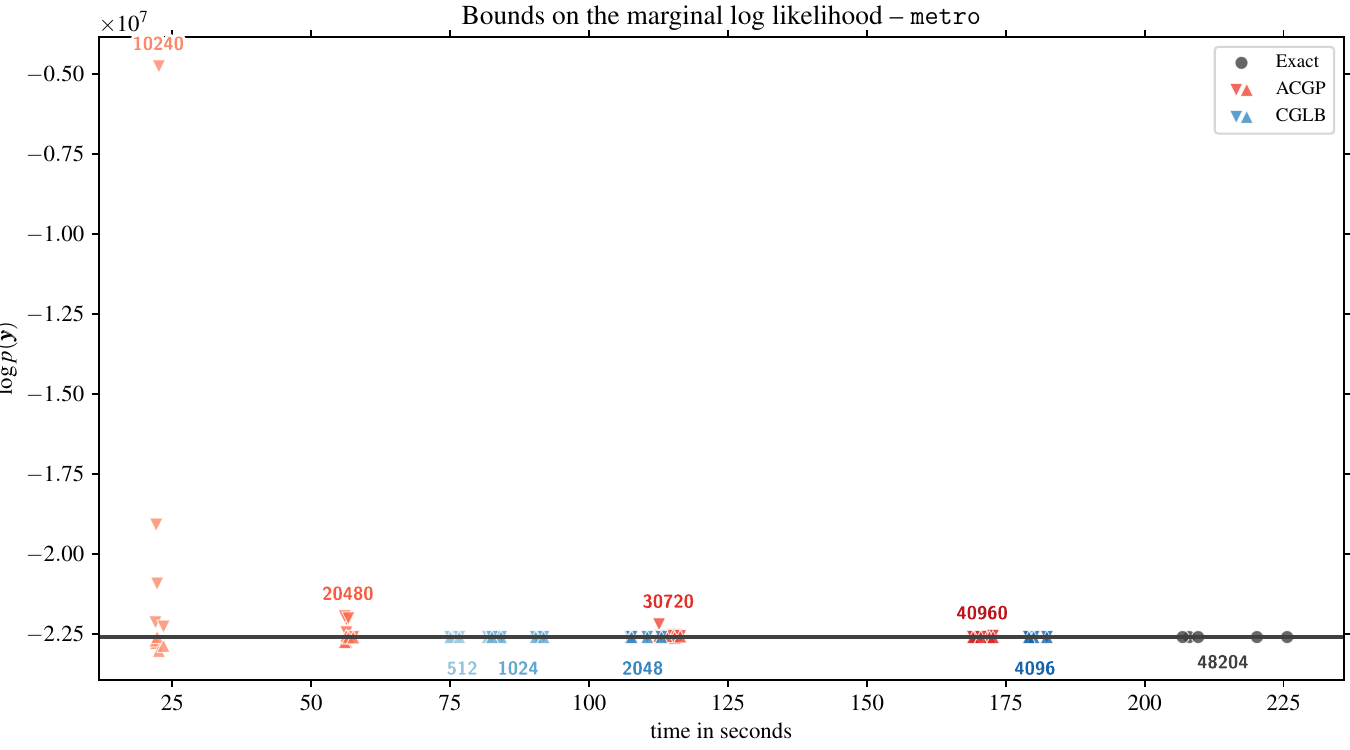}
		\subcaption{SE kernel, $\log\ell = 2$}
		\label{subfig:metro_rbf_llh_2}
	\end{minipage}
	\begin{minipage}[b]{.5\textwidth}
		\centering
		\includegraphics[width=0.96\textwidth]{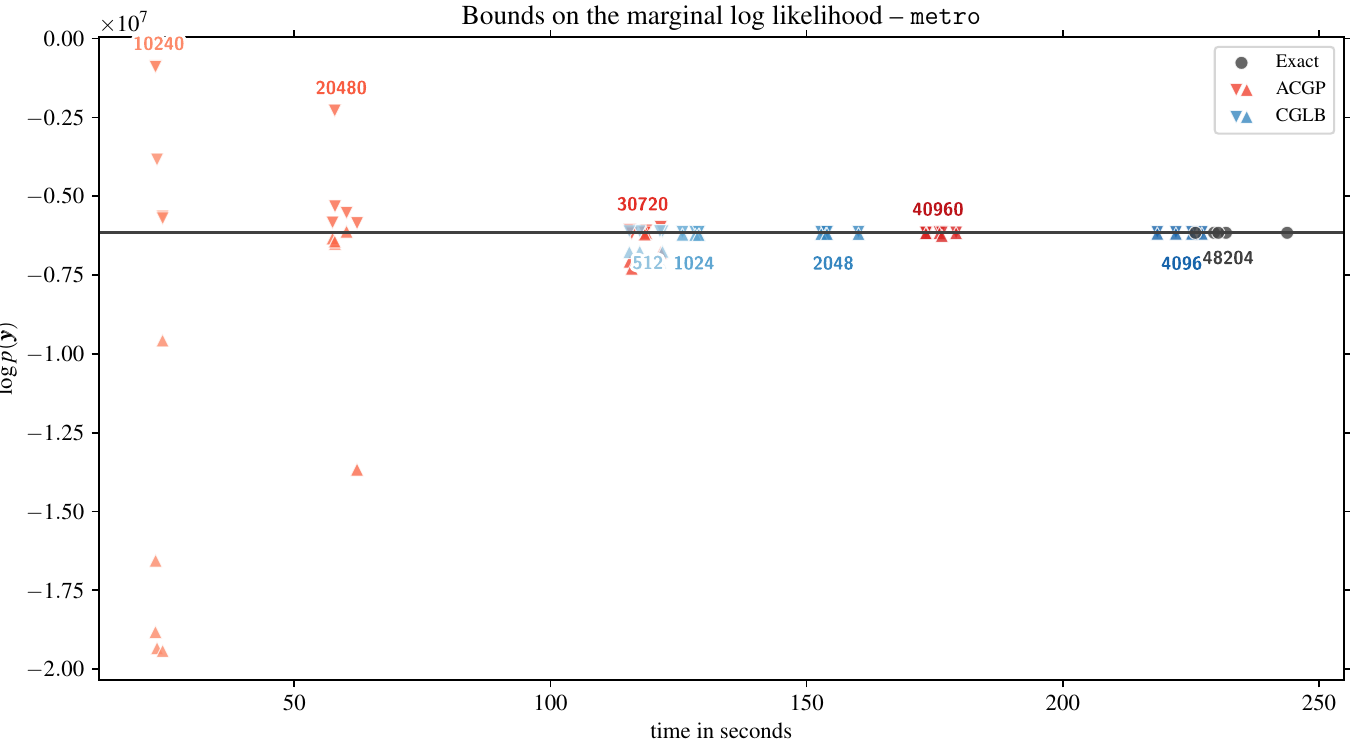}
		\subcaption{OU kernel, $\log\ell = 2$}
		\label{subfig:metro_ou_llh_2}
	\end{minipage}
	\caption{Upper and lower bounds on the marginal log-likeihood for the \texttt{metro} dataset when using a squared exponential (SE) kernel (left column) and the Ornstein-Uhlenbeck (OU) kernel (right column).}
	\label{fig:llh_bounds_metro_rbf}
\end{figure}

\clearpage
\subsubsection{Bounds for experiments on \texttt{pm25}}
\label{subsec:llh_bounds_pm25}
\begin{figure}[htb!]
	\begin{minipage}[b]{.5\textwidth}
		\centering
		\includegraphics[width=0.96\textwidth]{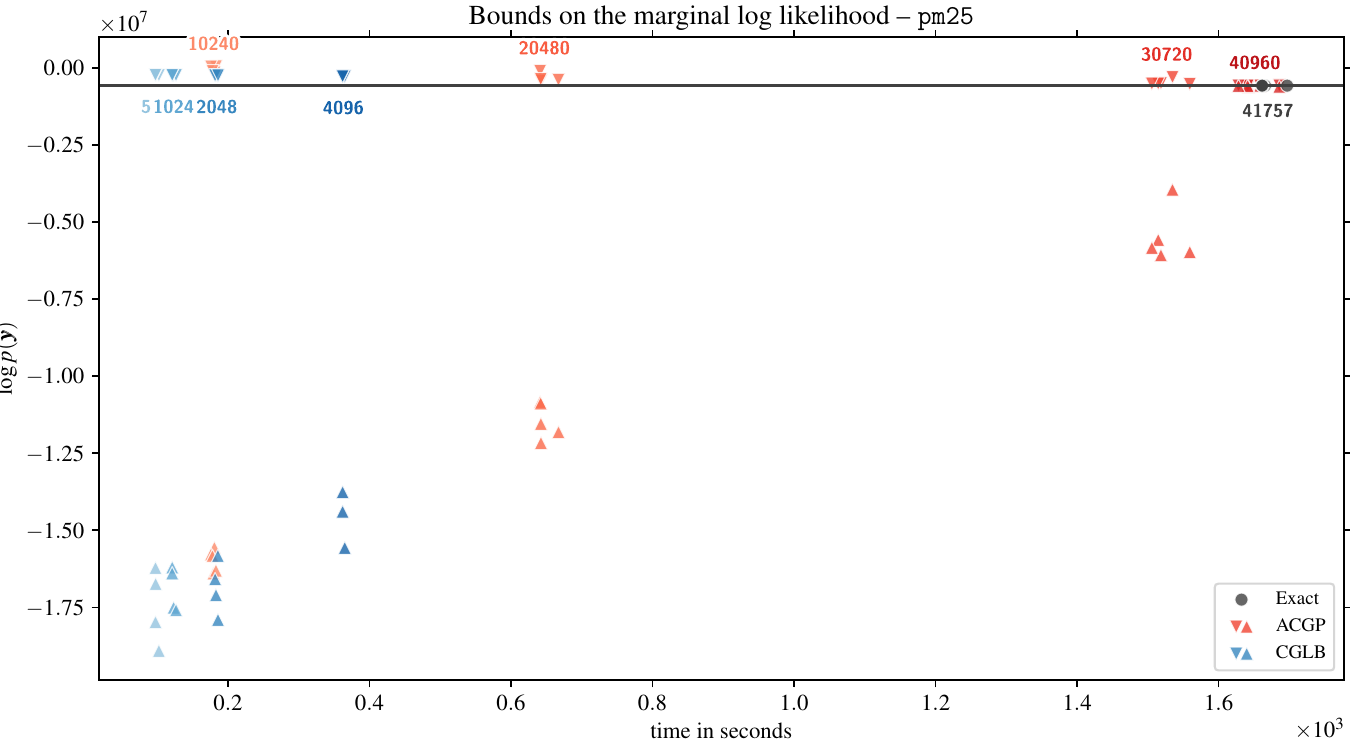}
		\subcaption{SE kernel, $\log\ell = -1$}
		\label{subfig:pm25_rbf_llh_-1}
	\end{minipage}
	\begin{minipage}[b]{.5\textwidth}
		\centering
		\includegraphics[width=0.96\textwidth]{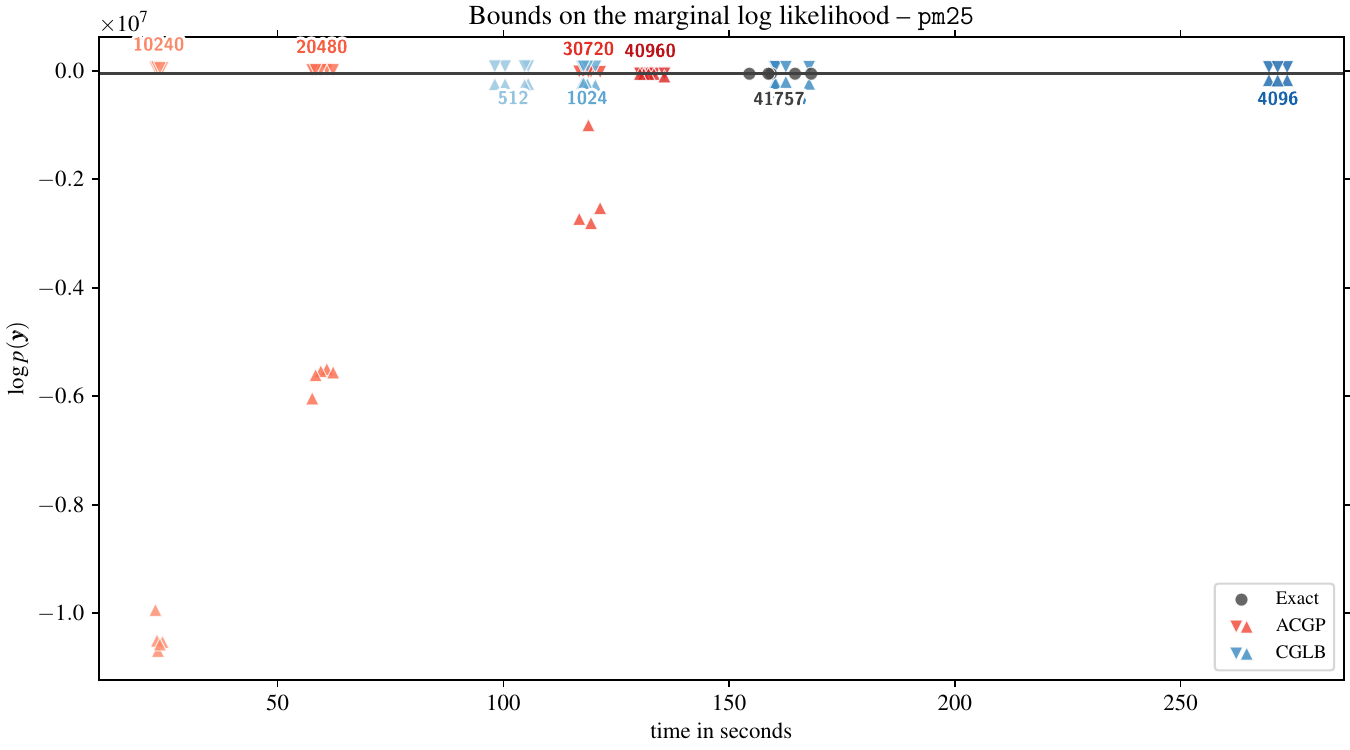}
		\subcaption{OU kernel, $\log\ell = -1$}
		\label{subfig:pm25_ou_llh_-1}
	\end{minipage}

	\begin{minipage}[b]{.5\textwidth}
		\centering
		\includegraphics[width=0.96\textwidth]{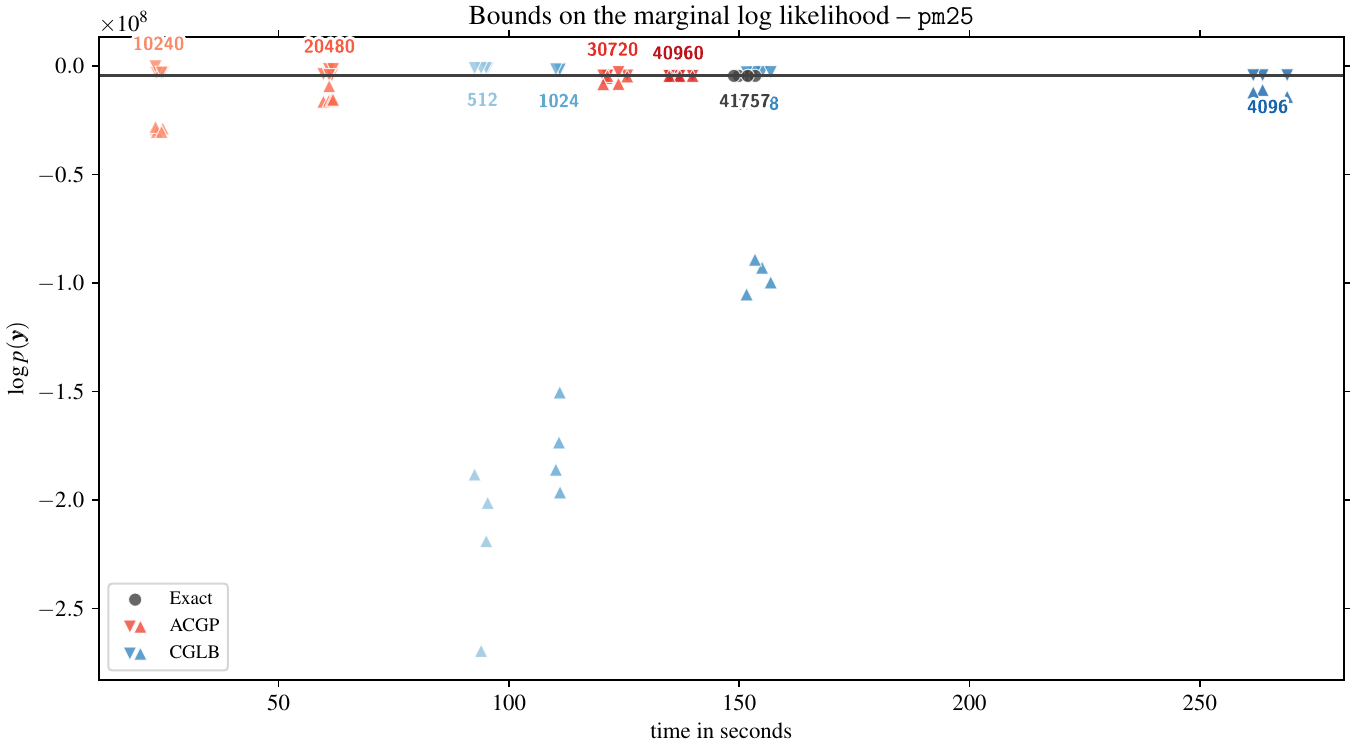}
		\subcaption{SE kernel, $\log\ell = 0$}
		\label{subfig:pm25_rbf_llh_0}
	\end{minipage}
	\begin{minipage}[b]{.5\textwidth}
		\centering
		\includegraphics[width=0.96\textwidth]{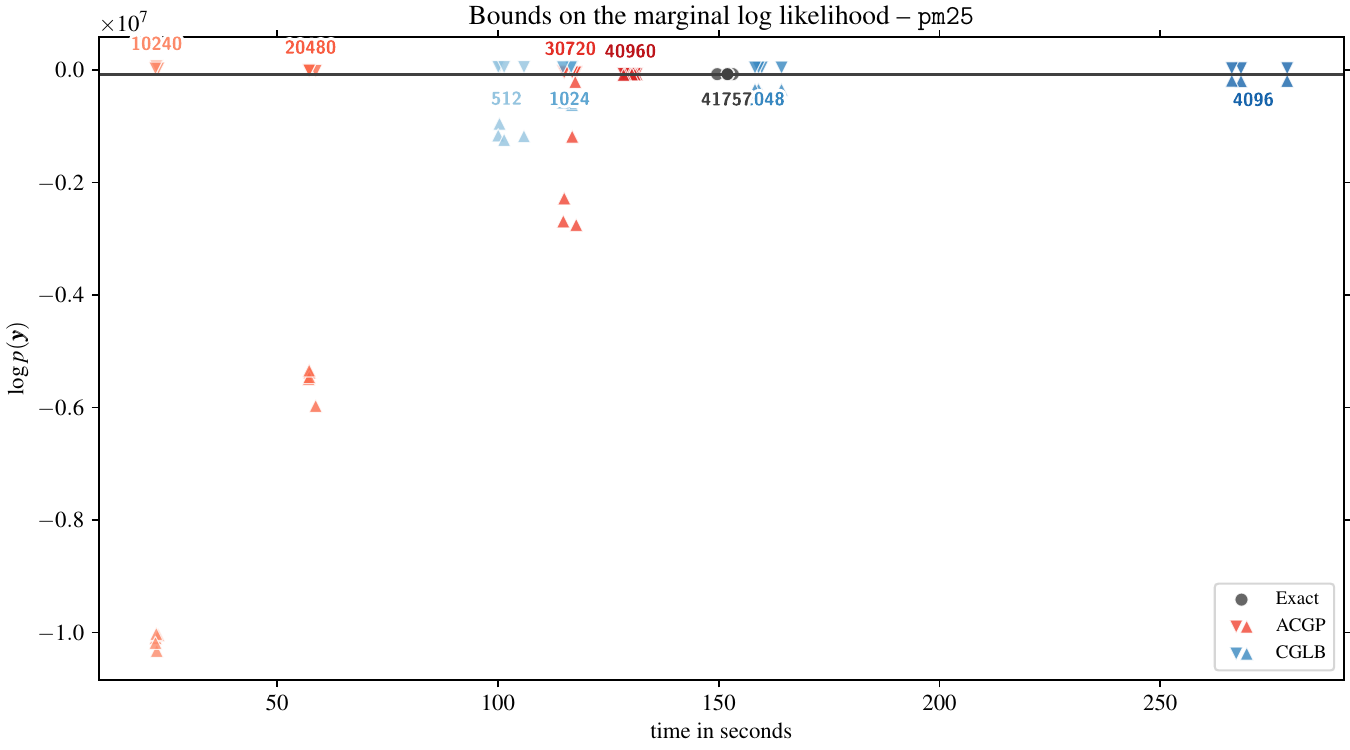}
		\subcaption{OU kernel, $\log\ell = 0$}
		\label{subfig:pm25_ou_llh_0}
	\end{minipage}

	\begin{minipage}[b]{.5\textwidth}
		\centering
		\includegraphics[width=0.96\textwidth]{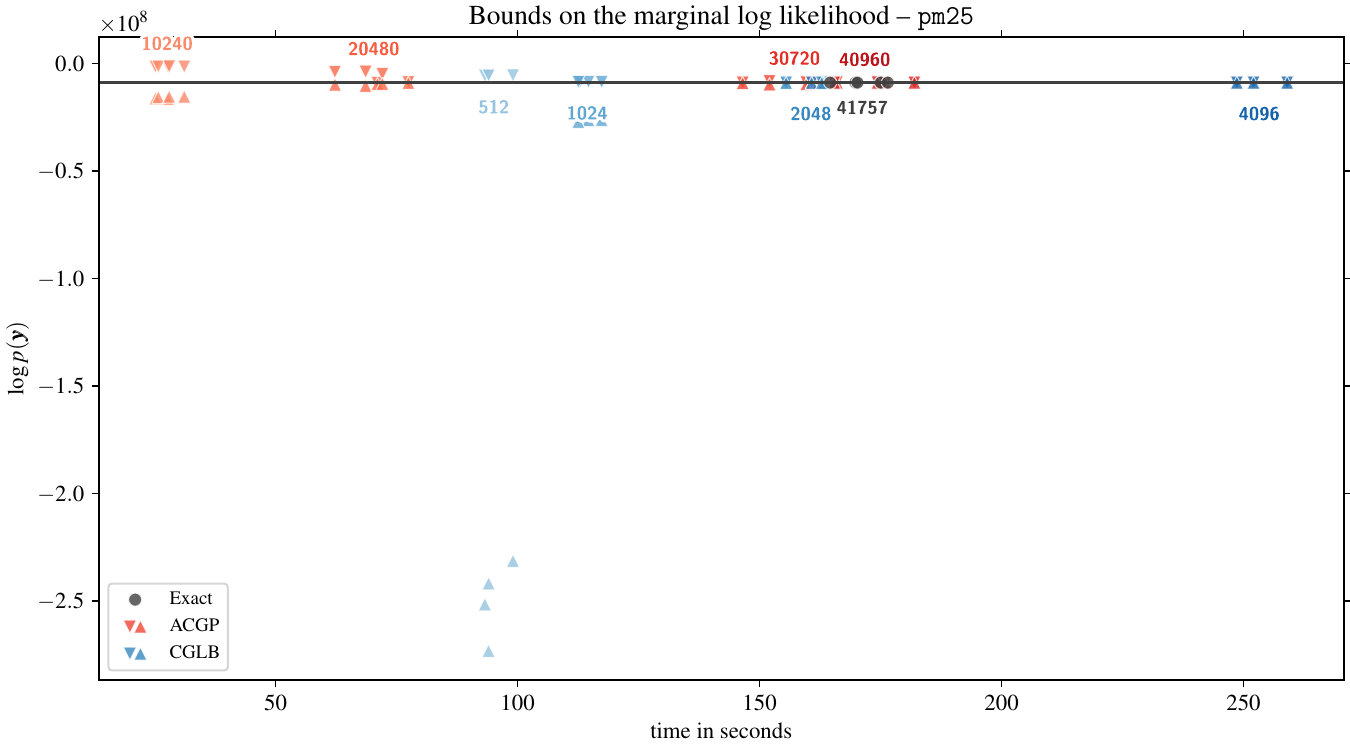}
		\subcaption{SE kernel, $\log\ell = 1$}
		\label{subfig:pm25_rbf_llh_1}
	\end{minipage}
	\begin{minipage}[b]{.5\textwidth}
		\centering
		\includegraphics[width=0.96\textwidth]{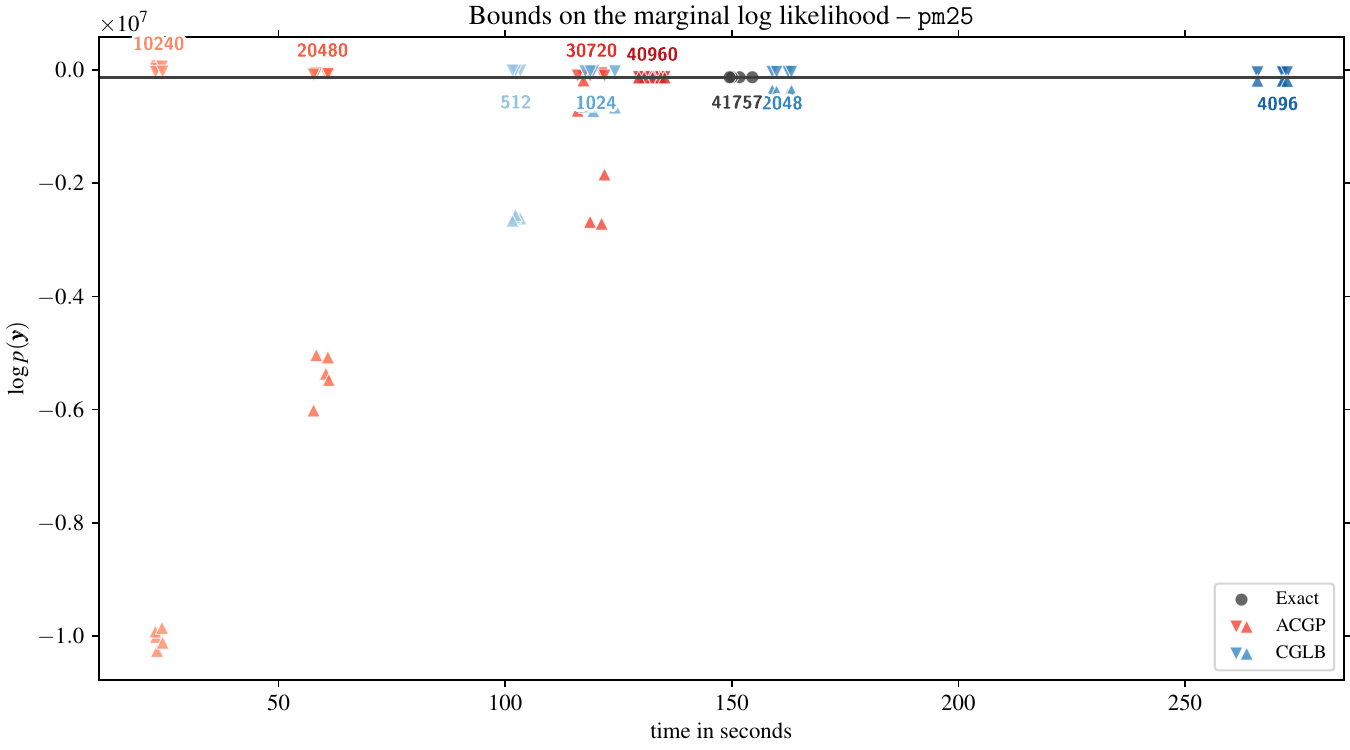}
		\subcaption{OU kernel, $\log\ell = 1$}
		\label{subfig:pm25_ou_llh_1}
	\end{minipage}

	\begin{minipage}[b]{.5\textwidth}
		\centering
		\includegraphics[width=0.96\textwidth]{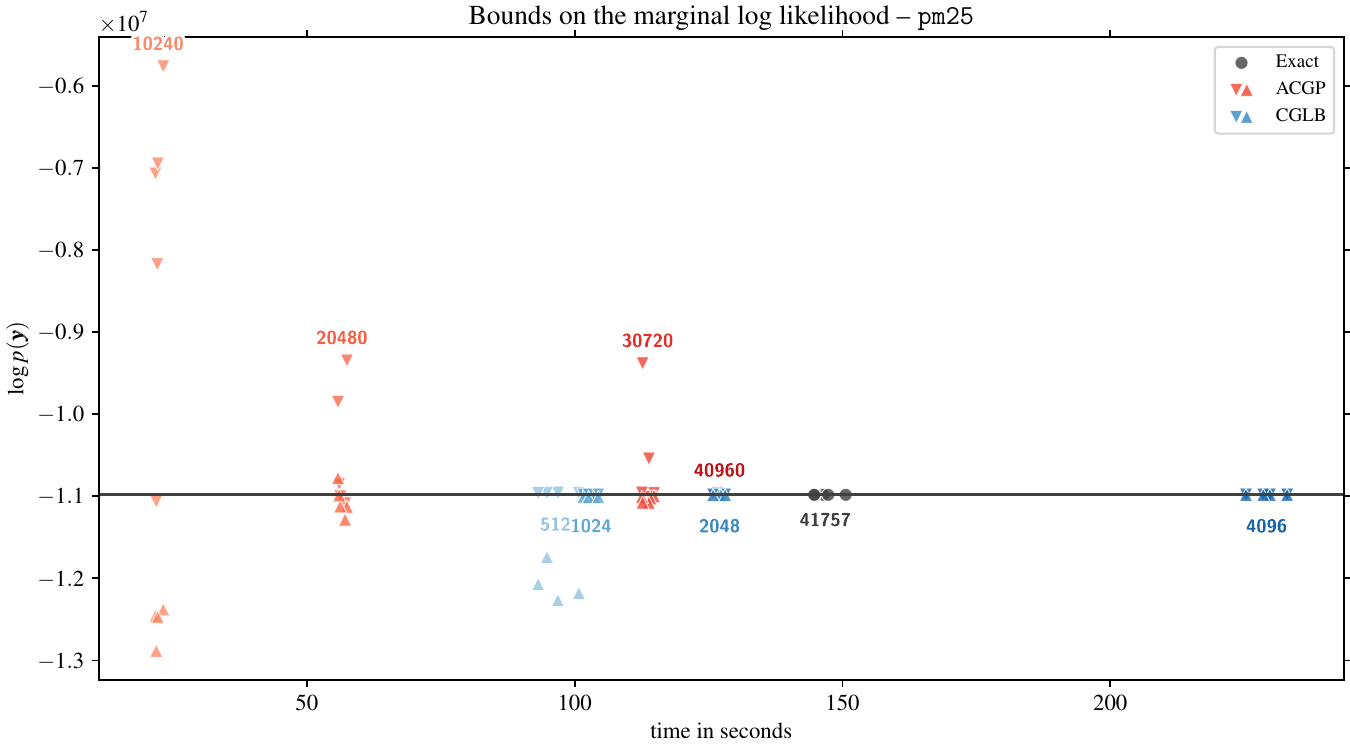}
		\subcaption{SE kernel, $\log\ell = 2$}
		\label{subfig:pm25_rbf_llh_2}
	\end{minipage}
	\begin{minipage}[b]{.5\textwidth}
		\centering
		\includegraphics[width=0.96\textwidth]{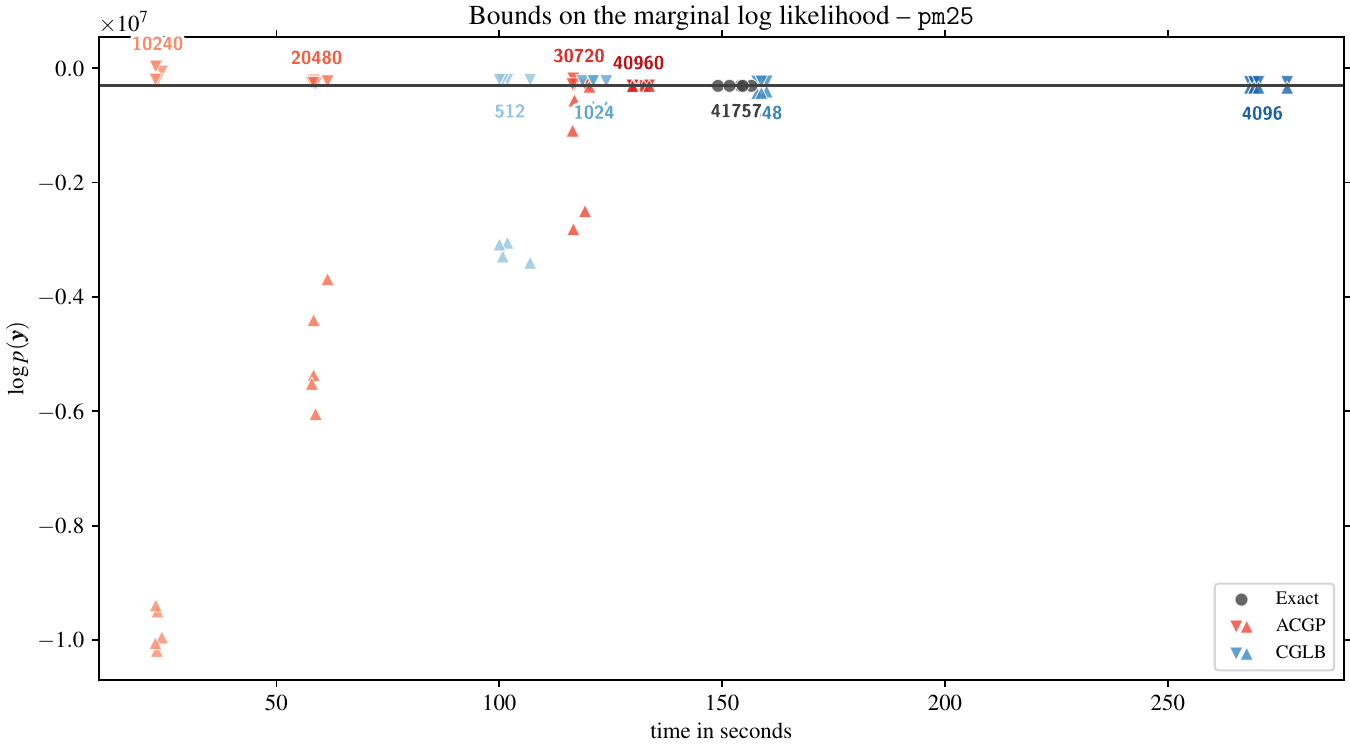}
		\subcaption{OU kernel, $\log\ell = 2$}
		\label{subfig:pm25_ou_llh_2}
	\end{minipage}
	\caption{Upper and lower bounds on the marginal log-likeihood for the \texttt{pm25} dataset when using a squared exponential (SE) kernel (left column) and the Ornstein-Uhlenbeck (OU) kernel (right column).}
	\label{fig:llh_bounds_pm25}
\end{figure}

\clearpage
\subsubsection{Bounds for experiments on \texttt{protein}}
\label{subsec:llh_bounds_protein}
\begin{figure}[htb!]
	\begin{minipage}[b]{.5\textwidth}
		\centering
		\includegraphics[width=0.96\textwidth]{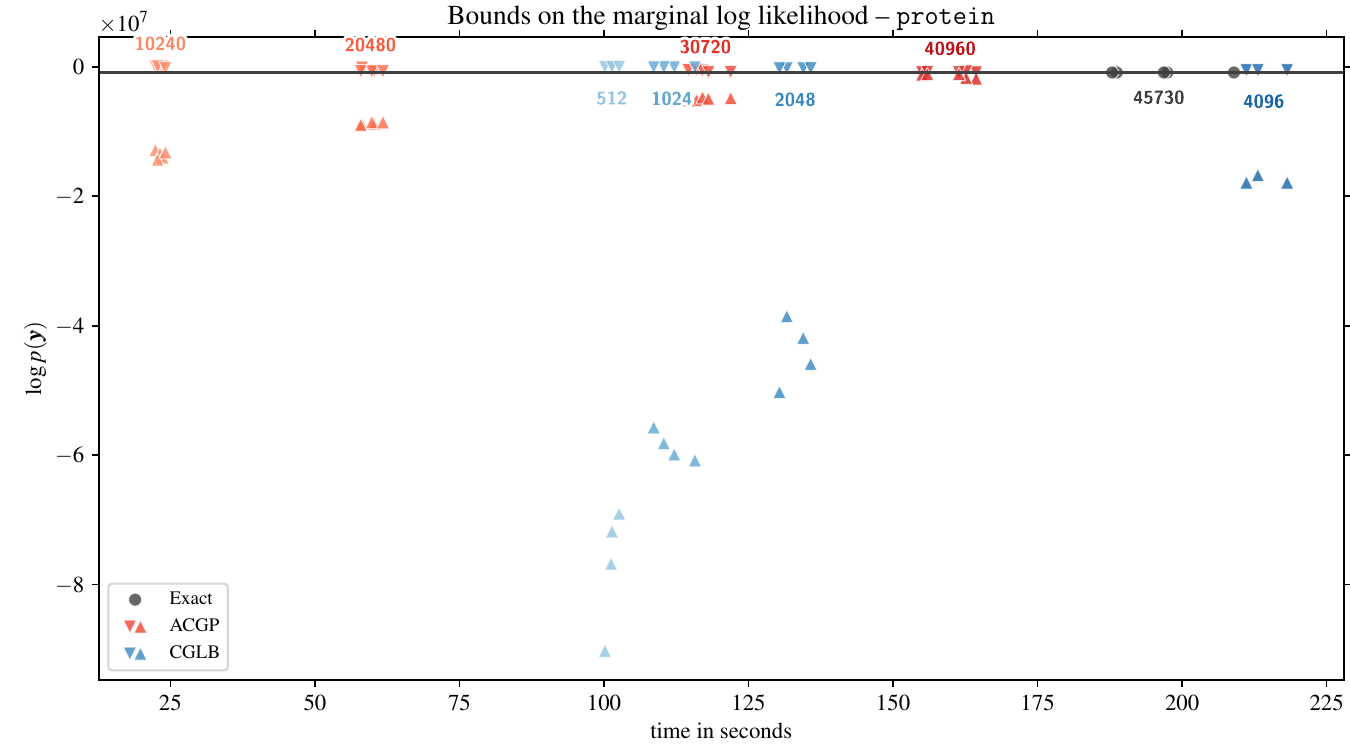}
		\subcaption{SE kernel, $\log\ell = -1$}
		\label{subfig:protein_rbf_llh_-1}
	\end{minipage}
	\begin{minipage}[b]{.5\textwidth}
		\centering
		\includegraphics[width=0.96\textwidth]{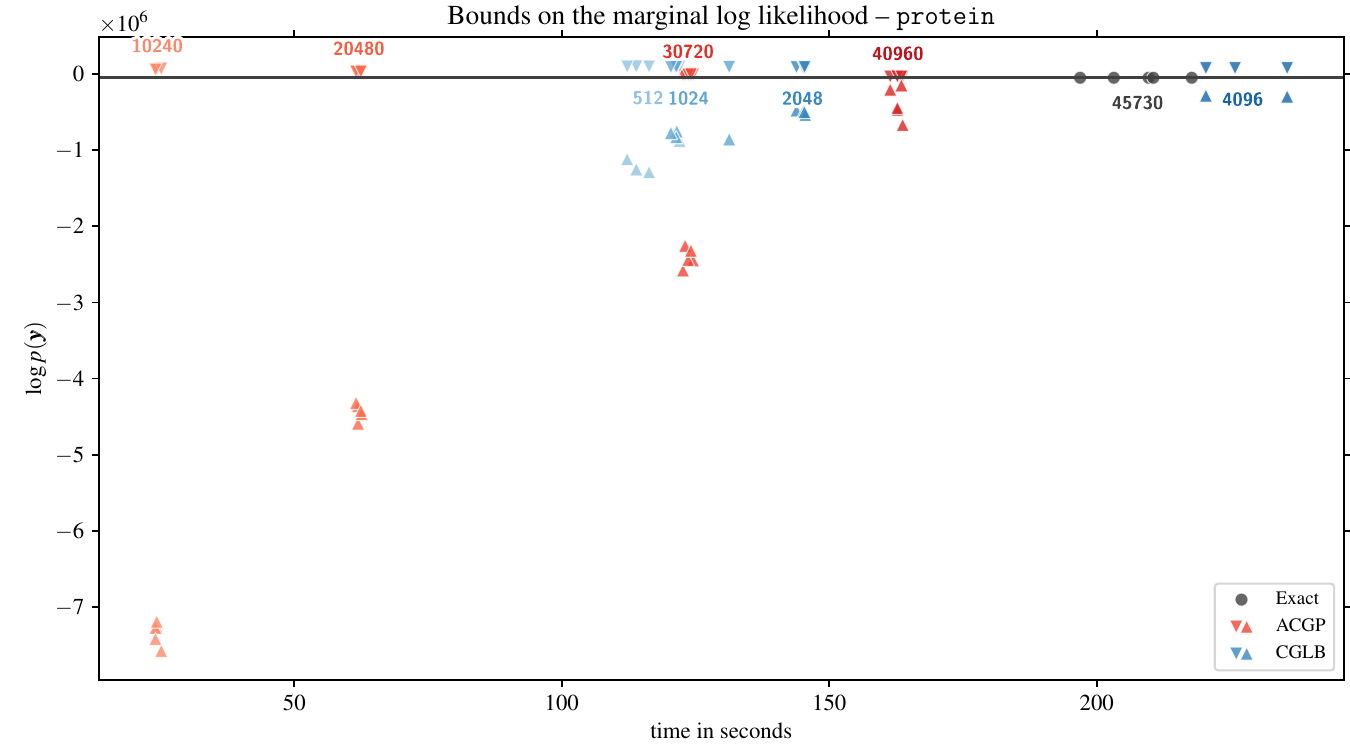}
		\subcaption{OU kernel, $\log\ell = -1$}
		\label{subfig:protein_ou_llh_-1}
	\end{minipage}

	\begin{minipage}[b]{.5\textwidth}
		\centering
		\includegraphics[width=0.96\textwidth]{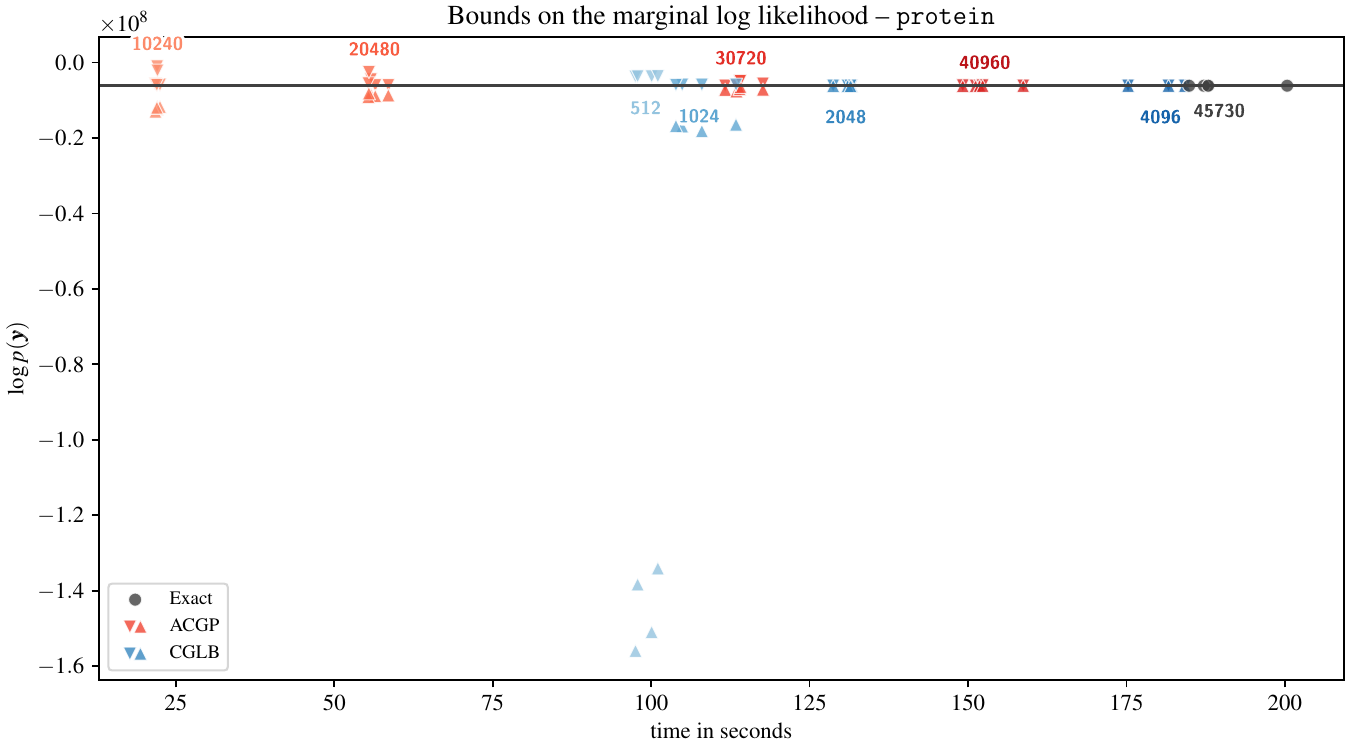}
		\subcaption{SE kernel, $\log\ell = 0$}
		\label{subfig:protein_rbf_llh_0}
	\end{minipage}
	\begin{minipage}[b]{.5\textwidth}
		\centering
		\includegraphics[width=0.96\textwidth]{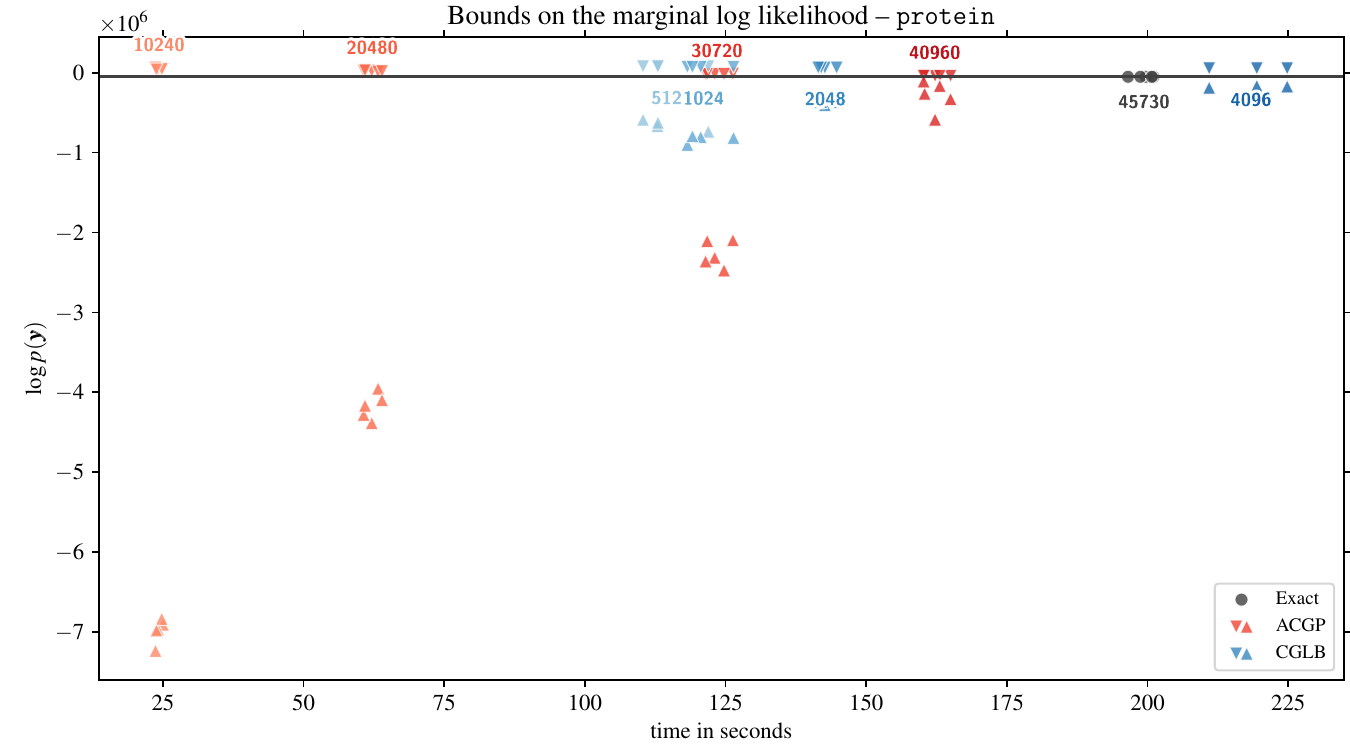}
		\subcaption{OU kernel, $\log\ell = 0$}
		\label{subfig:protein_ou_llh_0}
	\end{minipage}

	\begin{minipage}[b]{.5\textwidth}
		\centering
		\includegraphics[width=0.96\textwidth]{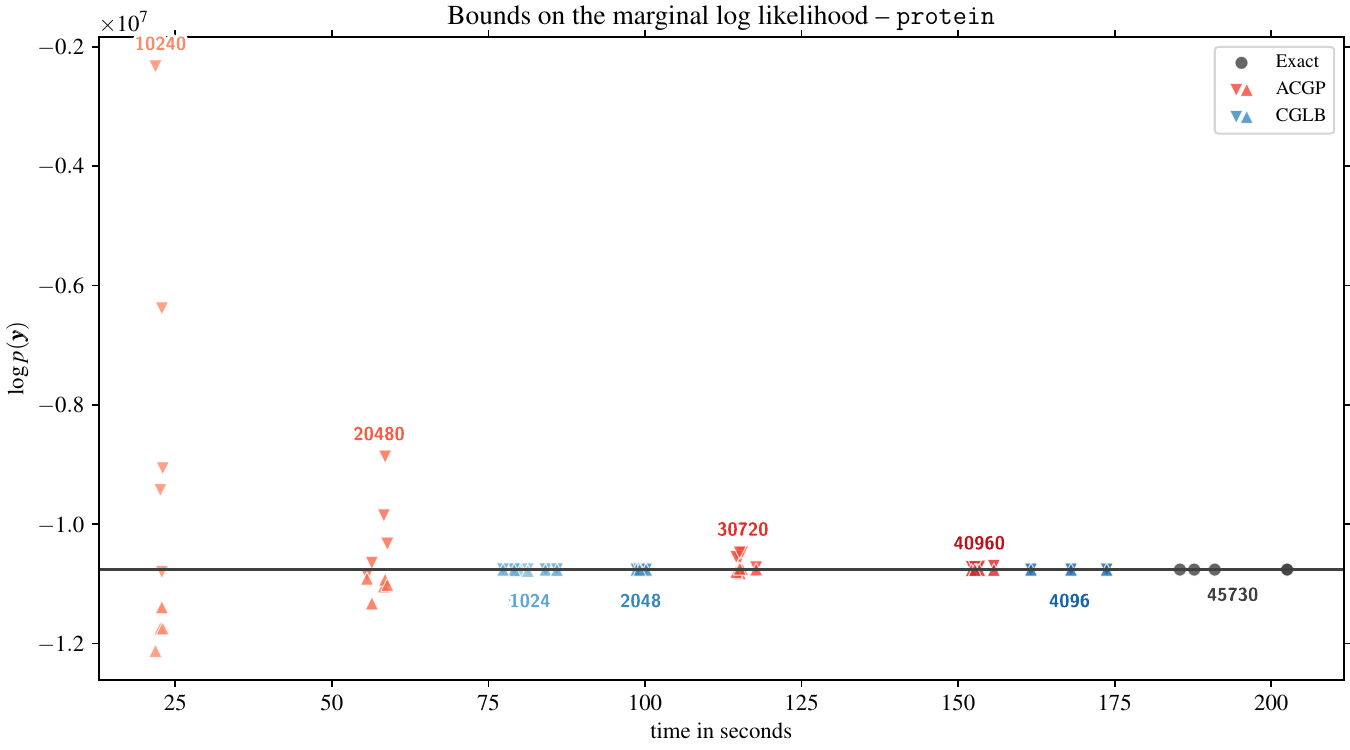}
		\subcaption{SE kernel, $\log\ell = 1$}
		\label{subfig:protein_rbf_llh_1}
	\end{minipage}
	\begin{minipage}[b]{.5\textwidth}
		\centering
		\includegraphics[width=0.96\textwidth]{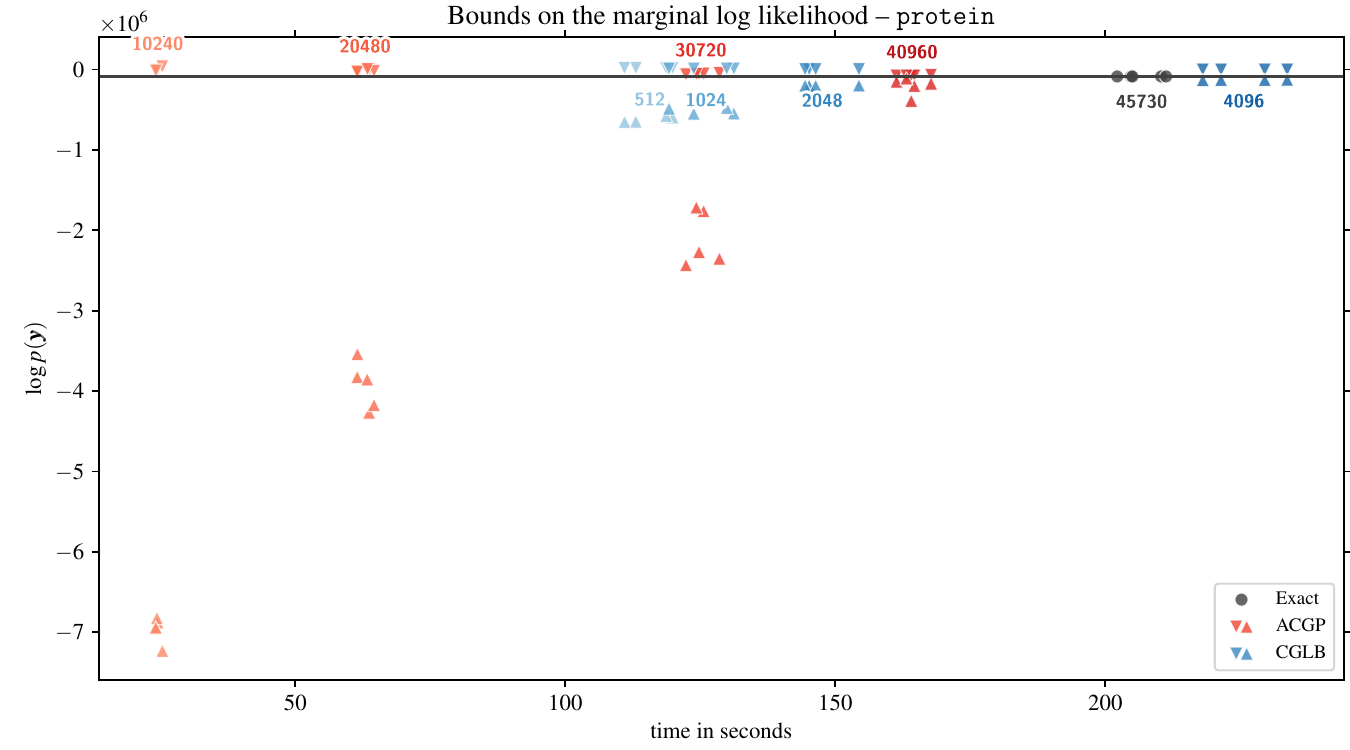}
		\subcaption{OU kernel, $\log\ell = 1$}
		\label{subfig:protein_ou_llh_1}
	\end{minipage}

	\begin{minipage}[b]{.5\textwidth}
		\centering
		\includegraphics[width=0.96\textwidth]{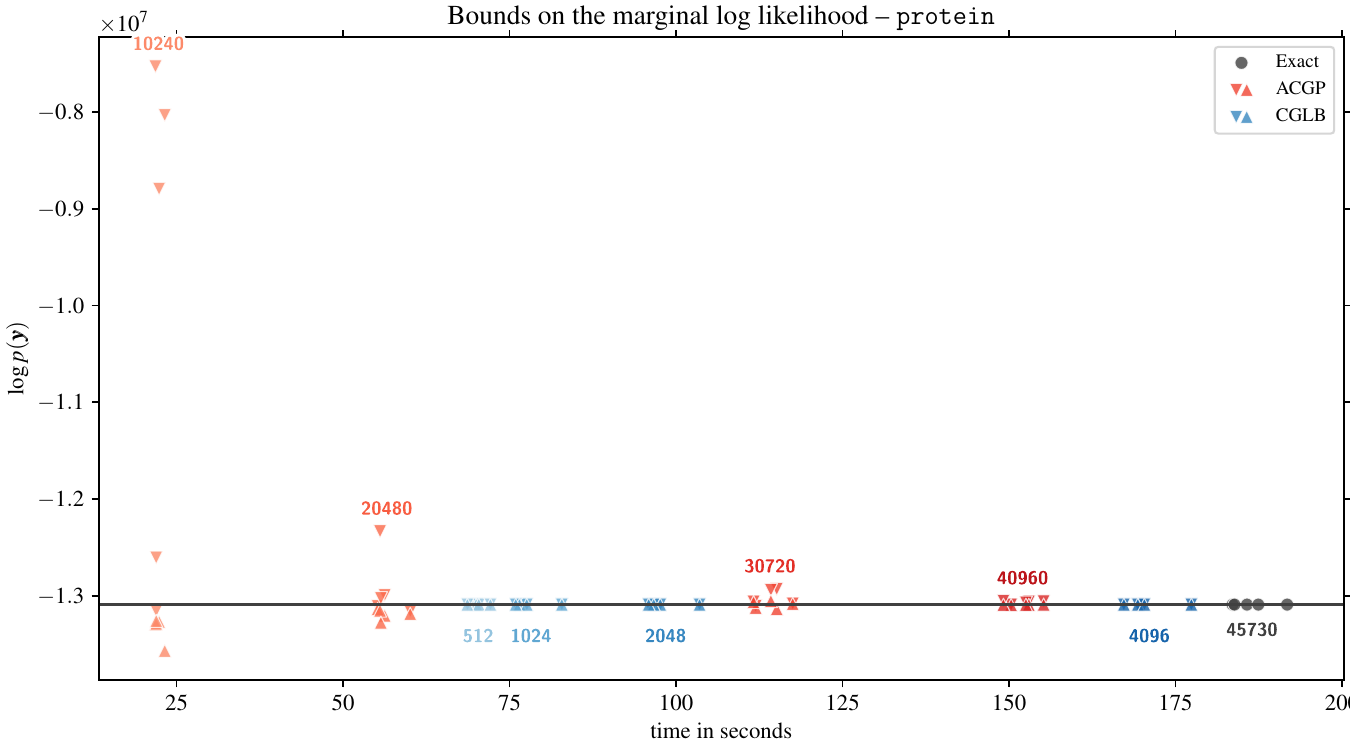}
		\subcaption{SE kernel, $\log\ell = 2$}
		\label{subfig:protein_rbf_llh_2}
	\end{minipage}
	\begin{minipage}[b]{.5\textwidth}
		\centering
		\includegraphics[width=0.96\textwidth]{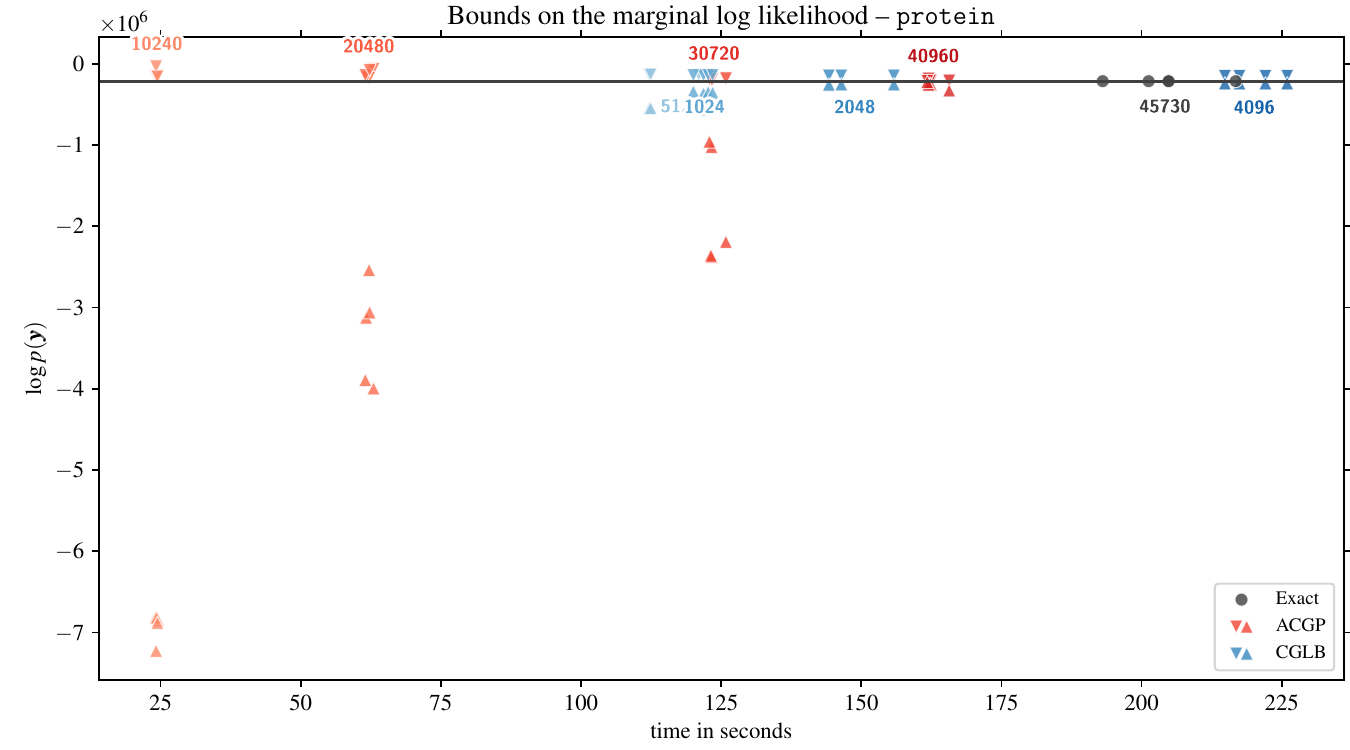}
		\subcaption{OU kernel, $\log\ell = 2$}
		\label{subfig:protein_ou_llh_2}
	\end{minipage}
	\caption{Upper and lower bounds on the marginal log-likeihood for the \texttt{protein} dataset when using a squared exponential (SE) kernel (left column) and the Ornstein-Uhlenbeck (OU) kernel (right column).}
	\label{fig:llh_bounds_protein}
\end{figure}

\clearpage
\subsubsection{Bounds for experiments on \texttt{kin40k}}
\label{subsec:llh_bounds_kin40k}
\begin{figure}[htb!]
	\begin{minipage}[b]{.5\textwidth}
		\centering
		\includegraphics[width=0.96\textwidth]{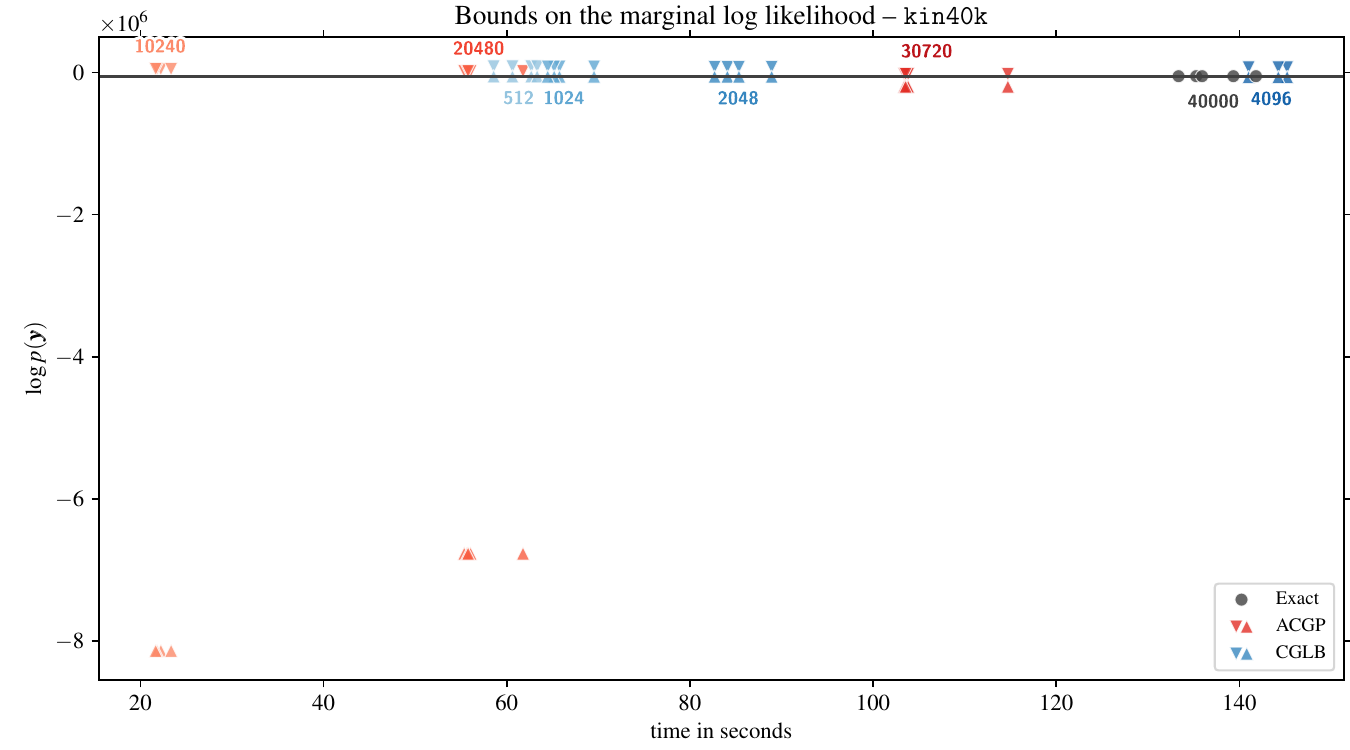}
		\subcaption{SE kernel, $\log\ell = -1$}
		\label{subfig:kin40k_rbf_llh_-1}
	\end{minipage}
	\begin{minipage}[b]{.5\textwidth}
		\centering
		\includegraphics[width=0.96\textwidth]{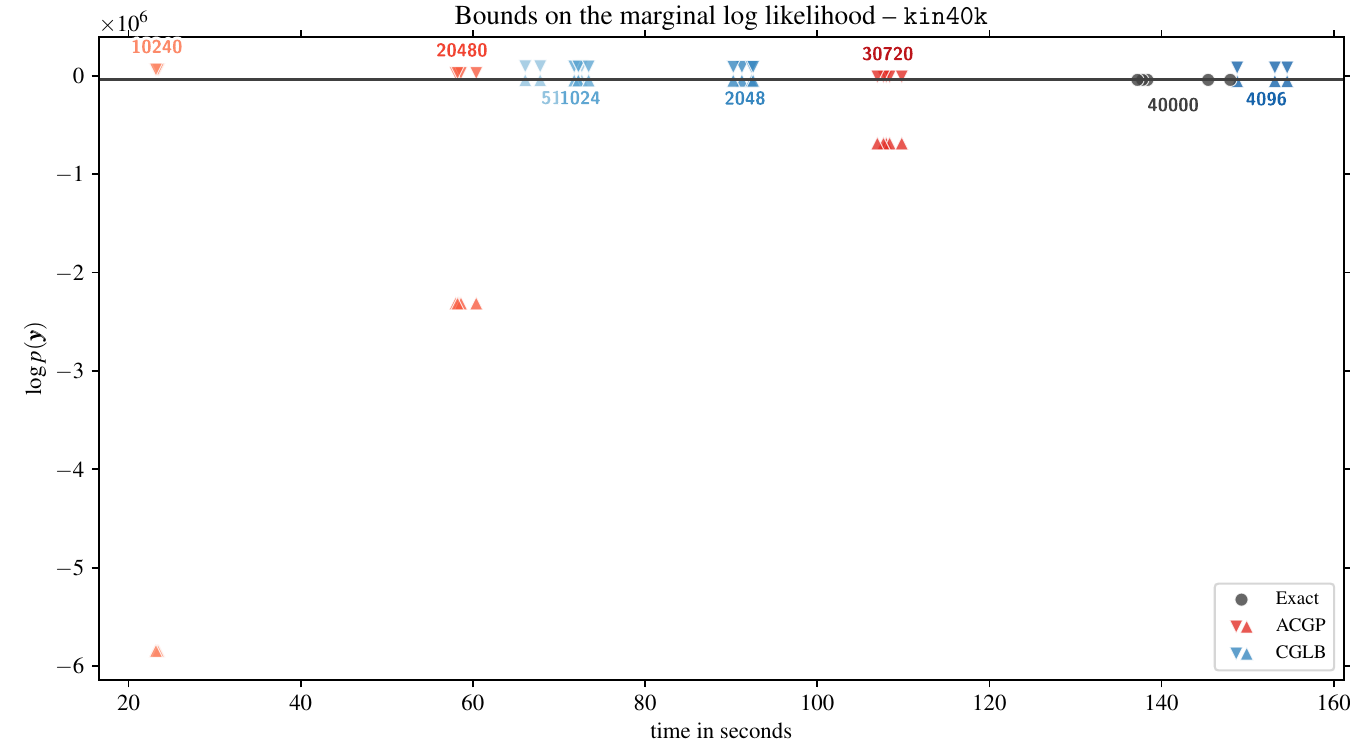}
		\subcaption{OU kernel, $\log\ell = -1$}
		\label{subfig:kin40k_ou_llh_-1}
	\end{minipage}

	\begin{minipage}[b]{.5\textwidth}
		\centering
		\includegraphics[width=0.96\textwidth]{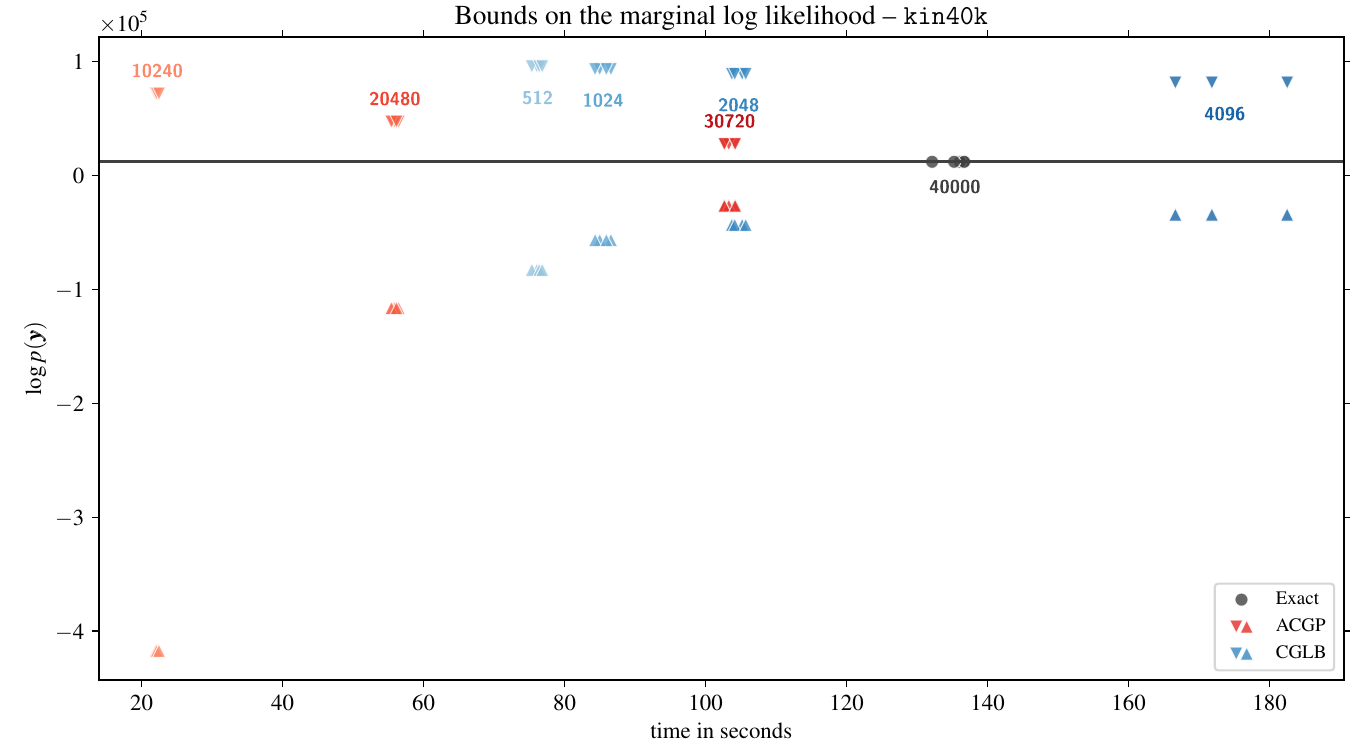}
		\subcaption{SE kernel, $\log\ell = 0$}
		\label{subfig:kin40k_rbf_llh_0}
	\end{minipage}
	\begin{minipage}[b]{.5\textwidth}
		\centering
		\includegraphics[width=0.96\textwidth]{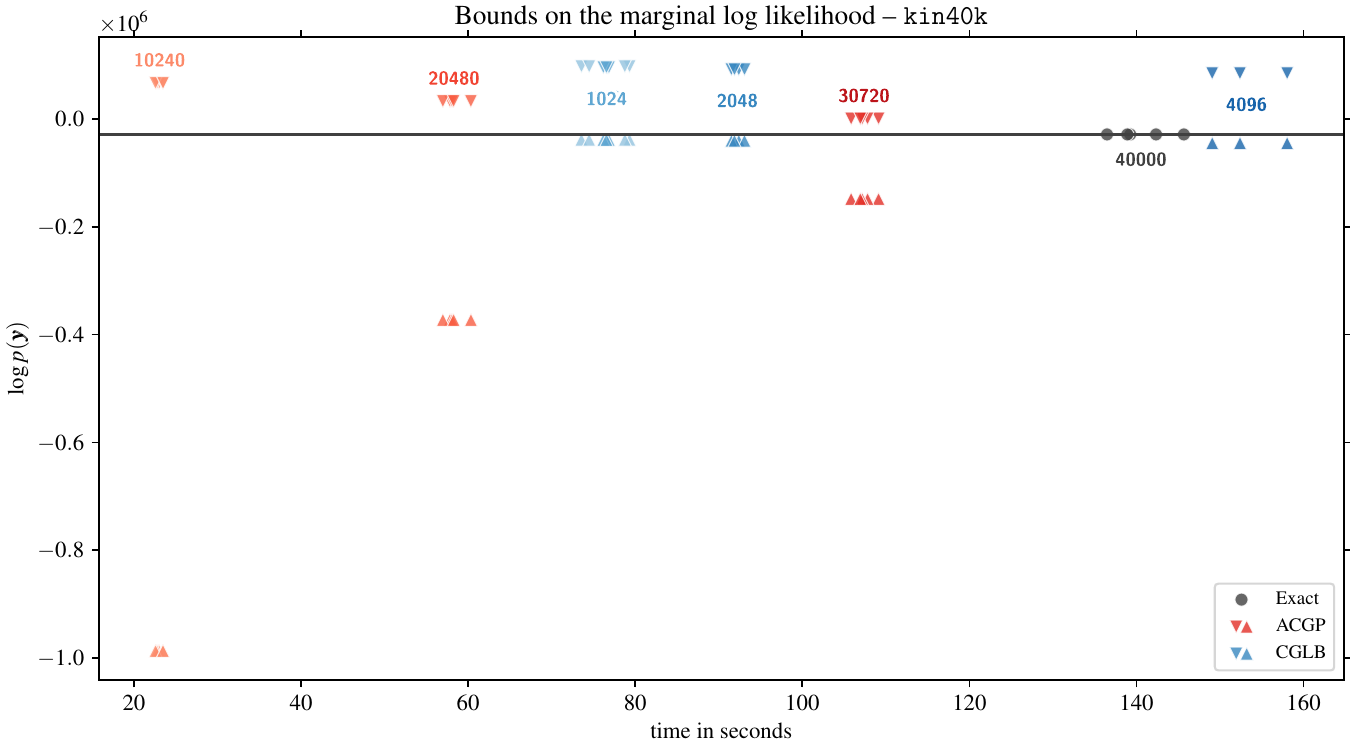}
		\subcaption{OU kernel, $\log\ell = 0$}
		\label{subfig:kin40k_ou_llh_0}
	\end{minipage}

	\begin{minipage}[b]{.5\textwidth}
		\centering
		\includegraphics[width=0.96\textwidth]{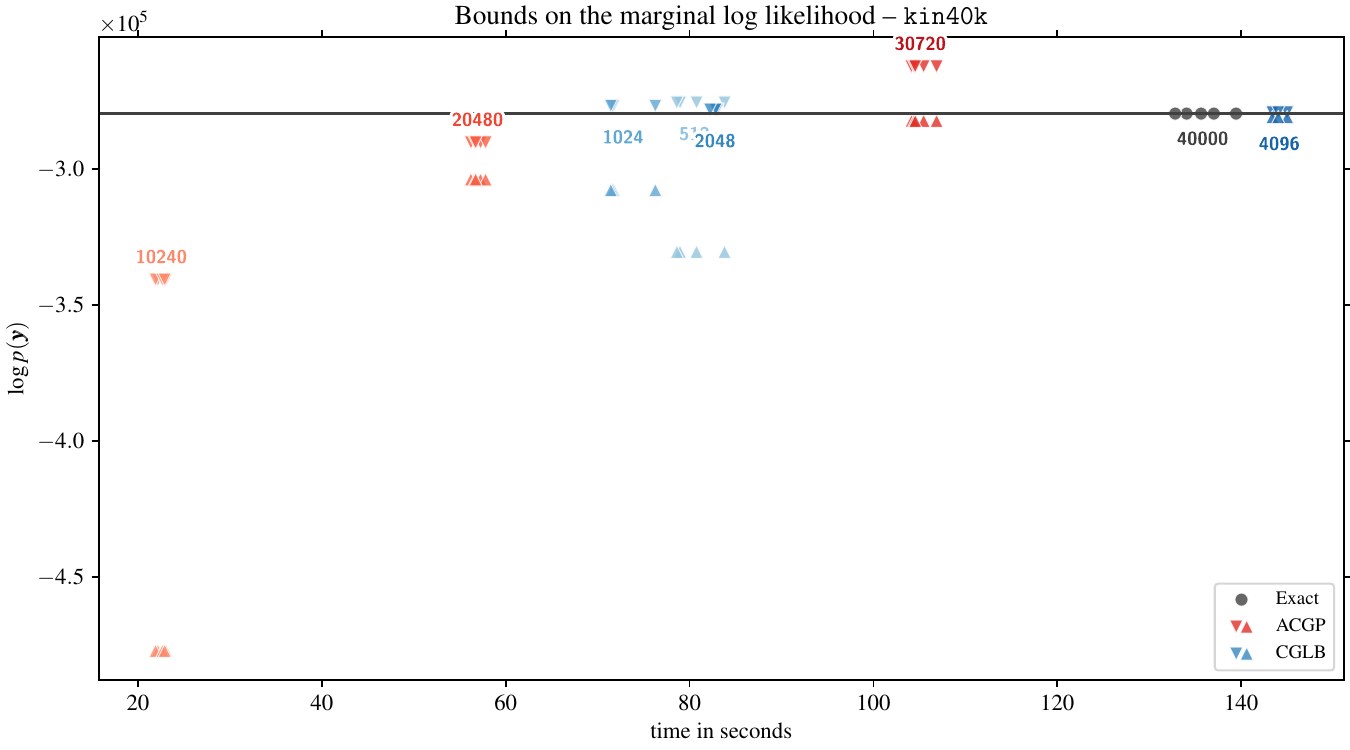}
		\subcaption{SE kernel, $\log\ell = 1$}
		\label{subfig:kin40k_rbf_llh_1}
	\end{minipage}
	\begin{minipage}[b]{.5\textwidth}
		\centering
		\includegraphics[width=0.96\textwidth]{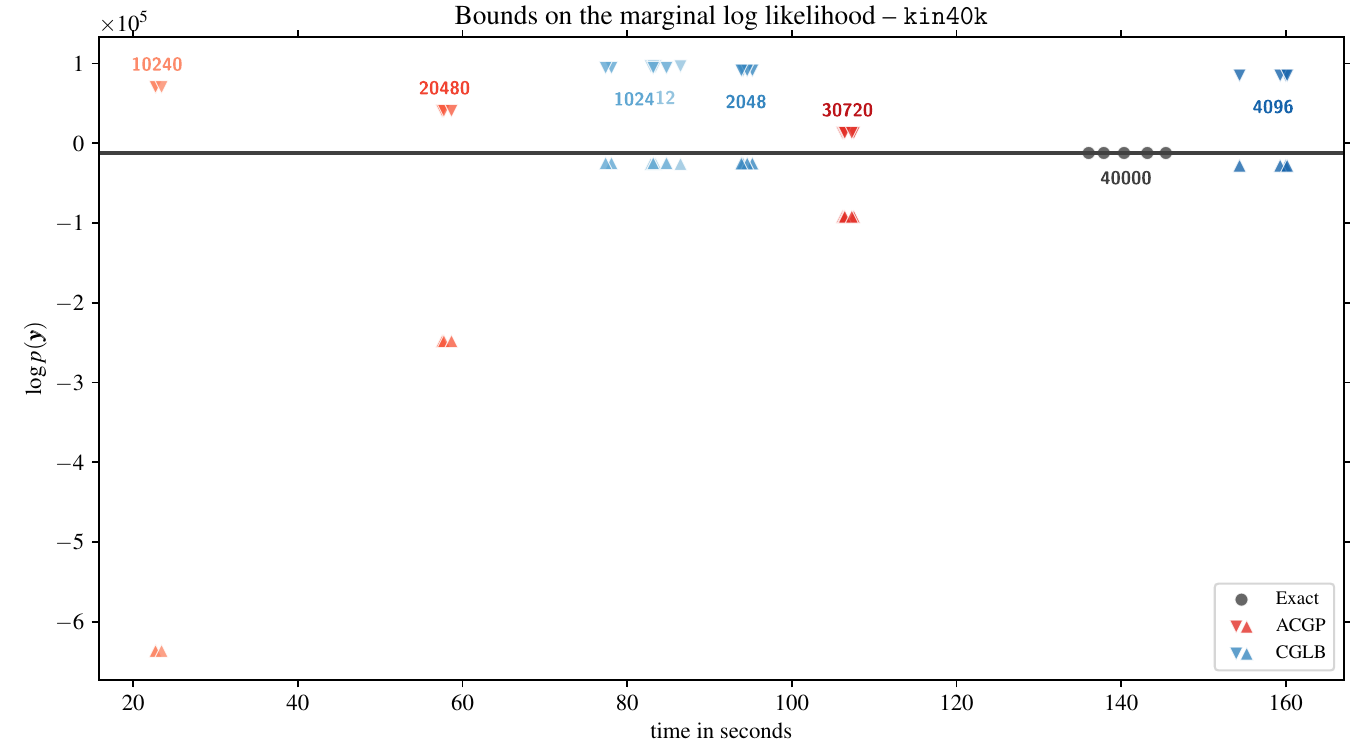}
		\subcaption{OU kernel, $\log\ell = 1$}
		\label{subfig:kin40k_ou_llh_1}
	\end{minipage}

	\begin{minipage}[b]{.5\textwidth}
		\centering
		\includegraphics[width=0.96\textwidth]{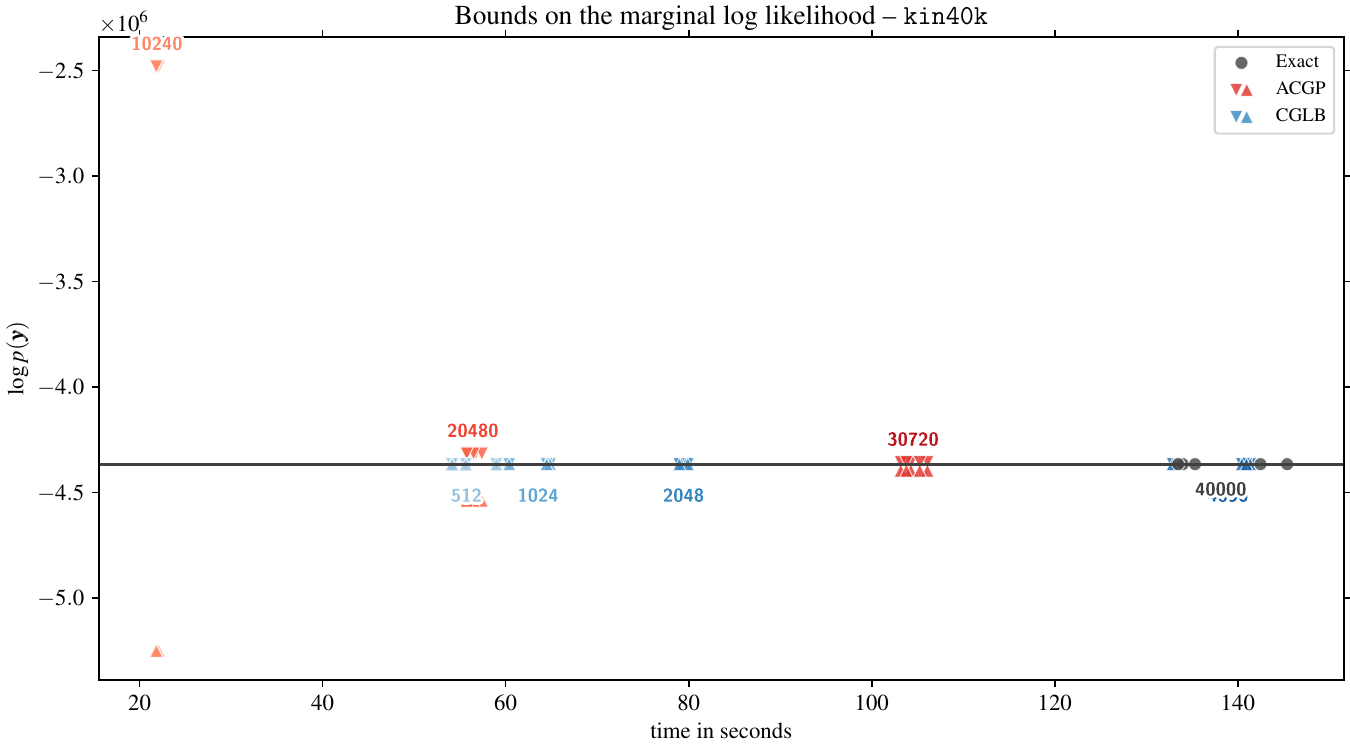}
		\subcaption{SE kernel, $\log\ell = 2$}
		\label{subfig:kin40k_rbf_llh_2}
	\end{minipage}
	\begin{minipage}[b]{.5\textwidth}
		\centering
		\includegraphics[width=0.96\textwidth]{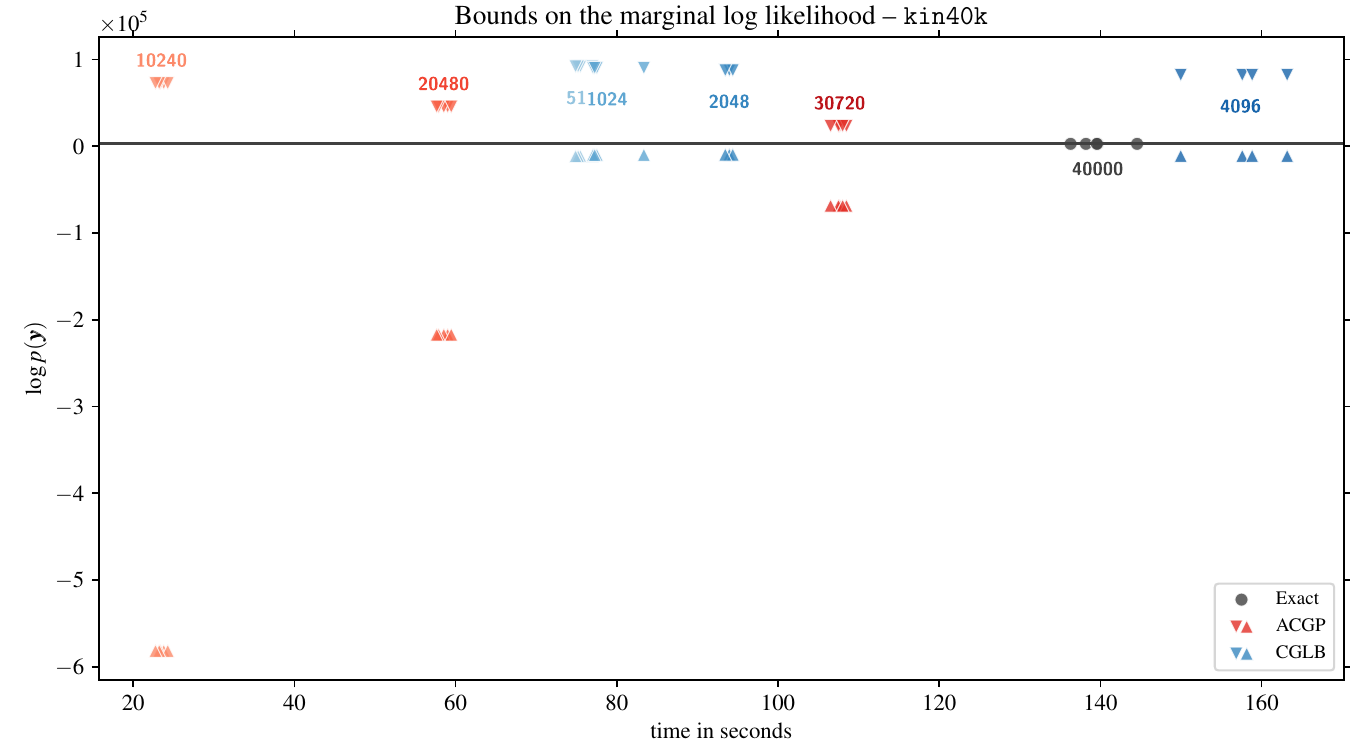}
		\subcaption{OU kernel, $\log\ell = 2$}
		\label{subfig:kin40k_ou_llh_2}
	\end{minipage}
	\caption{Upper and lower bounds on the marginal log-likeihood for the \texttt{kin40k} dataset when using a squared exponential (SE) kernel (left column) and the Ornstein-Uhlenbeck (OU) kernel (right column).}
	\label{fig:llh_bounds_kin40k}
\end{figure}
